# Supplementary material for: Thermodynamic stability of a cosmological SU(2)-weak gauge field
Source: arXiv:2203.12052 ancillary file (2022-03-24)
Supplement: Supplementary file 1 [file Calculations_for_Thermodynamic_stability.pdf]

# Calculations for “Thermodynamic stability of a cosmological SU(2)-weak gauge field”

Daniel Friedan

*New High Energy Theory Center and Department of Physics and Astronomy,  
Rutgers, The State University of New Jersey,  
Piscataway, New Jersey 08854-8019 U.S.A. and*

*Science Institute, The University of Iceland, Reykjavik, Iceland*

*dfriedan@gmail.com      physics.rutgers.edu/~friedan*

March 22, 2022

## ABSTRACT

This note shows calculations for the paper *Thermodynamic stability of a cosmological SU(2)-weak gauge field*. The section numbers and headings match those of the paper. The numerical calculations and some algebra calculations are performed in two SageMath notebooks. The Supplemental Materials — this note and the SageMath notebooks along with printouts as html and pdf — are available at [arXiv.org](https://arxiv.org) as ancillary files associated with the paper, at [cocalc.com/dfriedan/DM/SM](https://cocalc.com/dfriedan/DM/SM), and at [physics.rutgers.edu/~friedan](https://physics.rutgers.edu/~friedan).

## CONTENTS

|    |                                                                 |    |
|----|-----------------------------------------------------------------|----|
| 2  | Spin(4)-symmetric CGF                                           | 2  |
| 6  | Quadratic term in the action                                    | 3  |
|    | 6.1 Expand the action . . . . .                                 | 3  |
|    | 6.2 Operators $\Gamma$ and $*\hat{\nabla}$ . . . . .            | 4  |
| 7  | Spin(4) decomposition                                           | 5  |
| 8  | Five ODEs                                                       | 5  |
|    | 8.1 $\mathfrak{su}(2)$ notation . . . . .                       | 5  |
|    | 8.2 The representation $\{B_i\}$ . . . . .                      | 6  |
|    | 8.3 $\Gamma$ and $*\hat{\nabla}$ in terms of Casimirs . . . . . | 7  |
|    | 8.4 Wigner 6-j symbol and Racah W-coefficient . . . . .         | 8  |
|    | 8.5 The five $\mathbf{K}(z)$ matrices . . . . .                 | 9  |
|    | 8.6 Gauge symmetries . . . . .                                  | 11 |
| 9  | Time-translation zero-mode                                      | 12 |
|    | 9.1 More on Jacobi elliptic functions . . . . .                 | 13 |
| 10 | Classical mechanics analytic in complex time $z$                | 15 |
| 11 | Quantum mechanics analytic in complex time $z$                  | 15 |

|      |                                                                 |    |
|------|-----------------------------------------------------------------|----|
| 18   | Numerical evidence for Property <b>P</b>                        | 16 |
| 18.1 | Imaginary period monodromy $\mathcal{M}_i$ at $t = K$ . . . . . | 16 |
| 18.2 | $\mathcal{V}_{\text{phys}}(t)$ . . . . .                        | 17 |
|      | References                                                      | 17 |

## 2 Spin(4)-symmetric CGF

$S^3$  is the unit 3-sphere in  $\mathbb{R}^4$  with metric  $\hat{g}_{ij}(\hat{x})$ .

$$\hat{x} \in \mathbb{R}^4 \quad \delta_{\mu\nu} \hat{x}^\mu \hat{x}^\nu = 1 \quad (\hat{x}^\mu) = (\hat{x}^i, \hat{x}^4) \quad \hat{g}_{ij}(\hat{x}) d\hat{x}^i d\hat{x}^j = \delta_{\mu\nu} d\hat{x}^\mu d\hat{x}^\nu \quad (2.1)$$

$S^3$  is identified with  $\text{SU}(2)$  by

$$\hat{x} \in S^3 \quad \longleftrightarrow \quad g_{\hat{x}} = \hat{x}^4 \mathbf{1} + \hat{x}^k i^{-1} \sigma_k \in \text{SU}(2) \quad (2.2)$$

$\sigma_k$  are the Pauli matrices,

$$\sigma_i \sigma_j = \delta_{ij} + i \epsilon_{ij}{}^k \sigma_k \quad (2.3)$$

$\text{Spin}(4)$  is  $\text{SU}(2)_L \times \text{SU}(2)_R$ . It acts on  $S^3$  as  $\text{SO}(4)$ .

$$U = (g_L, g_R) \quad \hat{x} \mapsto U \hat{x} \quad g_{U\hat{x}} = g_L g_{\hat{x}} g_R^{-1} \quad (2.4)$$

The metric is

$$\hat{g}_{ij}(\hat{x}) = \frac{1}{2} \text{tr} \left[ \hat{\partial}_i g_{\hat{x}} \hat{\partial}_j (g_{\hat{x}}^{-1}) \right] \quad \hat{\partial}_i = \frac{\partial}{\partial \hat{x}^i} \quad (2.5)$$

The Dirac matrices at  $\hat{x}$  are the components of an  $\mathfrak{su}(2)$ -valued 1-form

$$\hat{\gamma}_i(\hat{x}) = \frac{1}{2} g_{\hat{x}} \hat{\partial}_i (g_{\hat{x}}^{-1}) \quad (2.6)$$

At the north pole,

$$\hat{N} = (0, 0, 0, 1) \quad \hat{g}_{ij}(\hat{N}) = \delta_{ij} \quad \hat{\gamma}_i(\hat{N}) = \frac{i}{2} \sigma_i \quad (2.7)$$

so everywhere on  $S^3$

$$\hat{\gamma}_i(\hat{x}) \hat{\gamma}_j(\hat{x}) = -\frac{1}{4} \hat{g}_{ij}(\hat{x}) - \frac{1}{2} \hat{\epsilon}_{ij}{}^k(\hat{x}) \hat{\gamma}_k(\hat{x}) \quad (2.8)$$

where  $\hat{\epsilon}_{ijk}(\hat{x})$  is the volume 3-form. Also at  $\hat{N}$ ,

$$\hat{\partial}_{[i} \hat{\gamma}_{j]} = \frac{1}{2} \hat{\partial}_{[i} g_{\hat{x}} \hat{\partial}_{j]} (g_{\hat{x}}^{-1}) = \frac{1}{2} i^{-1} \sigma_{[i} i \sigma_{j]} = i \epsilon_{ij}{}^k \sigma_k = 2 \epsilon_{ij}{}^k \hat{\gamma}_k = -2 [\hat{\gamma}_i, \hat{\gamma}_j] \quad (2.9)$$

$$\hat{\partial}_i \hat{\gamma}_j + [\hat{\gamma}_i, \hat{\gamma}_j] - i \leftrightarrow j = 0$$

so the  $\text{Spin}(4)$ -symmetric covariant derivative acting on spinors is

$$\hat{\nabla}_i = \hat{\partial}_i + \hat{\gamma}_i \quad \hat{\nabla}_{[i} \hat{\gamma}_{j]} = 0 \quad (2.10)$$

with curvature

$$[\hat{\nabla}_i, \hat{\nabla}_j] = \hat{\partial}_{[i} \hat{\gamma}_{j]} + [\hat{\gamma}_i, \hat{\gamma}_j] = \hat{\epsilon}_{ij}{}^k \hat{\gamma}_k \quad (2.11)$$

Extending  $\hat{\nabla}_i$  to be the metric covariant derivative on tensors as well,

$$\hat{\nabla}_i \hat{\gamma}_j = 0 \quad (2.12)$$

because  $\hat{\nabla}_{[i} \hat{\gamma}_{j]} = 0$  and  $\hat{\nabla}_i \hat{\gamma}_j + \hat{\nabla}_j \hat{\gamma}_i$  would have to equal  $A_{ij}^k \hat{\gamma}_k$  for  $A_{ij}^k$  a 3-tensor symmetric in  $i, j$ . There is no such  $\text{SO}(4)$ -symmetric 3-tensor.

## 6 Quadratic term in the action

### 6.1 Expand the action

The Spin(4)-symmetric classical gauge field has covariant derivative:

$$D_0^{\text{cl}} = \partial_t \quad D_k^{\text{cl}} = \hat{\nabla}_k + \hat{b}(\hat{t})\hat{\gamma}_k \quad (6.1)$$

The curvature is

$$\begin{aligned} F_{0j}^{\text{cl}} &= [D_0^{\text{cl}}, D_j^{\text{cl}}] = \partial_t \hat{b} \hat{\gamma}_j \\ F_{ij}^{\text{cl}} &= [D_i^{\text{cl}}, D_j^{\text{cl}}] = [\hat{\nabla}_i, \hat{\nabla}_j] + \hat{b}^2 [\hat{\gamma}_i, \hat{\gamma}_j] = (1 - \hat{b}^2) \hat{\epsilon}_{ij}{}^k \hat{\gamma}_k \end{aligned} \quad (6.2)$$

The perturbed gauge field has covariant derivative

$$D_0 = D_0^{\text{cl}} = \partial_t \quad D_i = D_i^{\text{cl}} + B_i \quad (6.3)$$

and curvature

$$\begin{aligned} F_{0j} &= [D_0, D_j] = F_{0j}^{\text{cl}} + \partial_t B_j \\ F_{ij} &= [D_i, D_j] = F_{ij}^{\text{cl}} + D_{[i}^{\text{cl}} B_{j]} + [B_i, B_j] \\ D_i^{\text{cl}} B_j &= \hat{\nabla}_i B_j + \hat{b} [\hat{\gamma}_i, B_j] \end{aligned} \quad (6.4)$$

The Yang-Mills action is

$$\frac{1}{\hbar} S_{\text{gauge}} = \frac{1}{2g^2} \int \text{tr}(-F_{\mu\nu} F^{\mu\nu}) \sqrt{-\hat{g}} d^3 \hat{x} d\hat{t} \quad (6.5)$$

$$\text{tr}(-F_{\mu\nu} F^{\mu\nu}) = \text{tr}(2F_{0j} F_0{}^j - F_{ij} F^{ij}) \quad (6.6)$$

The zeroth order term in  $B$  is

$$\begin{aligned} \text{tr}(-F_{\mu\nu} F^{\mu\nu})_0 &= \text{tr} \left( 2(\partial_t \hat{b})^2 \hat{\gamma}_j \hat{\gamma}^j - (1 - \hat{b}^2)^2 \hat{\epsilon}_{ij}{}^k \hat{\epsilon}^{ijk'} \gamma_k \gamma_{k'} \right) \\ &= 3 \left[ -(\partial_t \hat{b})^2 + (1 - \hat{b}^2)^2 \right] \end{aligned} \quad (6.7)$$

The first order term is

$$\begin{aligned} \text{tr}(-F_{\mu\nu} F^{\mu\nu})_1 &= \text{tr} (4F_{0j}^{\text{cl}} \partial_t B^j - 4F_{ij}^{\text{cl}} D^{\text{cl}i} B^j) \\ &= \text{tr} \left( 4\partial_t \hat{b} \hat{\gamma}_j \partial_t B^j - 4(1 - \hat{b}^2) \hat{\epsilon}^{ijk} \hat{\gamma}_k (\hat{\nabla}_i B_j + \hat{b} [\hat{\gamma}_i, B_j]) \right) \\ &= \partial_t \left( 4\partial_t \hat{b} \text{tr}(\hat{\gamma}_j B^j) \right) - 4 \left( \partial_t^2 \hat{b} + 2(\hat{b}^2 - 1)\hat{b} \right) \text{tr}(\hat{\gamma}_j B^j) \end{aligned} \quad (6.8)$$

The second order term is

$$\text{tr}(-F_{\mu\nu} F^{\mu\nu})_2 = \text{tr}(-2\partial_t B_j \partial_t B^j - D_{[i}^{\text{cl}} B_{j]} D^{\text{cl}i} B^j - 2F_{ij}^{\text{cl}} [B^i, B^j]) \quad (6.9)$$

The zeroth order term in the action is

$$\frac{1}{\hbar} S_0 = \text{Vol}(S^3) \frac{3}{g^2} \int \left[ -\frac{1}{2} \left( \frac{d\hat{b}}{d\hat{t}} \right)^2 + \frac{1}{2} (\hat{b}^2 - 1)^2 \right] d\hat{t} \quad \text{Vol}(S^3) = 2\pi^2 \quad (6.10)$$

The first order term is

$$\begin{aligned} \frac{1}{\hbar} S_1 &= \frac{2}{g^2} \int \left[ \partial_{\hat{t}} \left( \partial_{\hat{t}} \hat{b} B_0 \right) - \left( \partial_{\hat{t}}^2 \hat{b} + 2(\hat{b}^2 - 1)\hat{b} \right) B_0 \right] d\hat{t} \\ B_0(\hat{t}) &= \int \text{tr}(\hat{\gamma}_j B^j) \sqrt{-\hat{g}} d^3 \hat{x} \end{aligned} \quad (6.11)$$

The second order term in the action is

$$\begin{aligned} \frac{1}{\hbar} S_2 &= \frac{1}{2g^2} \int \text{tr}(2\partial_{\hat{t}} B_j \partial_{\hat{t}} B^j - D_{[i}^{\text{cl}} B_{j]} D^{\text{cl} i} B^j - 2F_{ij}^{\text{cl}}[B^i, B^j]) \sqrt{-\hat{g}} d^3 \hat{x} d\hat{t} \\ &= \frac{1}{g^2} \int \text{tr}(\partial_{\hat{t}} B_j \partial_{\hat{t}} B^j - B_i \square B^i) \sqrt{-\hat{g}} d^3 \hat{x} d\hat{t} \end{aligned} \quad (6.12)$$

$$\int \text{tr}(B_i \square B^i) \sqrt{-\hat{g}} d^3 \hat{x} = \int \text{tr}(D_{[i}^{\text{cl}} B_{j]} D^{\text{cl} i} B^j + F_{ij}^{\text{cl}}[B^i, B^j]) \sqrt{-\hat{g}} d^3 \hat{x} \quad (6.13)$$

Changing variables

$$\hat{t} = \epsilon z \quad \hat{b}(\hat{t}) = \frac{1}{\epsilon} b(z) \quad (6.14)$$

the second order term becomes

$$\frac{1}{\hbar} S_2 = \frac{1}{\epsilon g^2} \int \text{tr}(\partial_z B_i \partial_z B^i - B_i \mathbf{K} B^i) \sqrt{-\hat{g}} d^3 \hat{x} dz \quad (6.15)$$

$$\mathbf{K} = \epsilon^2 \square \quad (6.16)$$

$$\int \text{tr}(B_i \mathbf{K} B^i) \sqrt{-\hat{g}} d^3 \hat{x} = \int \text{tr}(\epsilon^2 D_{[i}^{\text{cl}} B_{j]} D^{\text{cl} i} B^j + \epsilon^2 F_{ij}^{\text{cl}}[B^i, B^j]) \sqrt{-\hat{g}} d^3 \hat{x} \quad (6.17)$$

## 6.2 Operators $\Gamma$ and $*\hat{\nabla}$

Define linear operators on the perturbations  $B_i$ .

$$\Gamma B_i = \epsilon_i^{jk} [\gamma_j, B_k] \quad *\hat{\nabla} B_i = \epsilon_i^{jk} \hat{\nabla}_j B_k \quad (6.18)$$

so

$$\begin{aligned} *D^{\text{cl}} B_i &= \epsilon_i^{jk} D_j^{\text{cl}} B_k = *\hat{\nabla} B_i + \hat{b} \Gamma B_i \\ D_{[i}^{\text{cl}} B_{j]} D^{\text{cl} i} B^j &= (*D^{\text{cl}} B_k) (*D^{\text{cl}} B^k) \end{aligned} \quad (6.19)$$

$$\text{tr}(F_{ij}^{\text{cl}}[B^i, B^j]) = (1 - \hat{b}^2) \text{tr}(2\epsilon_{ij}^k \hat{\gamma}_k B^i B^j) = (1 - \hat{b}^2) \text{tr}(B_k \Gamma B^k)$$

$\Gamma$  and  $*\hat{\nabla}$  are symmetric operators.

$$\begin{aligned} \int \text{tr}(B'^i *\hat{\nabla} B_i) &= \int \text{tr}(B'^i \epsilon_i^{jk} \hat{\nabla}_j B_k) = \int \text{tr}(\epsilon_k^{ji} \hat{\nabla}_j B'_i B^k) \\ &= \int \text{tr}(*\hat{\nabla} B'_k B^k) \end{aligned} \quad (6.20)$$

$$\begin{aligned} \int \text{tr}(B'^i \Gamma B_i) &= \int \text{tr}(B'^i \epsilon_i^{jk} (\gamma_j B_k - B_k \gamma_j)) = \int \text{tr}(\epsilon_i^{jk} (B'^i \gamma_j B_k - \gamma_j B'^i B_k)) \\ &= \int \text{tr}(\epsilon_k^{ji} [\gamma_j, B'_i] B^k) = \int \text{tr}(\Gamma B'_k B^k) \end{aligned} \quad (6.21)$$

So

$$\begin{aligned}\mathbf{K} &= \epsilon^2(*\hat{\nabla} + \hat{b}\Gamma)^2 + \epsilon^2(1 - \hat{b}^2)\Gamma \\ &= (\Gamma^2 - \Gamma)b^2 + (*\hat{\nabla}\Gamma + \Gamma*\hat{\nabla})\epsilon b + \left((*\hat{\nabla})^2 + \Gamma\right)\epsilon^2\end{aligned}\tag{6.22}$$

## 7 Spin(4) decomposition

The perturbations of the gauge field form the Spin(4) representation

$$\begin{aligned}\{B_i^j(\hat{x})\} &= \bigoplus_{j_3} (j_1 \otimes j_2 \otimes j_3, j_3) \quad j_1 = j_2 = 1 \\ &= \bigoplus_{j_3, J} \mathbb{C}^{N(J, j_3)} \otimes (J, j_3) \quad (J, j_3) = (j_L, j_R)\end{aligned}\tag{7.1}$$

The infinitesimal gauge transformations form the representation

$$\begin{aligned}\{v^i(\hat{x})\} &= \bigoplus_{j_3} (1 \otimes j_3, j_3) = \bigoplus_{j_3, J} \mathbb{C}^{N_{\text{gauge}}(J, j_3)} \otimes (J, j_3) \\ \mathbb{C}^{N_{\text{gauge}}(J, j_3)} &\subseteq \mathbb{C}^{N(J, j_3)}\end{aligned}\tag{7.2}$$

The triple tensor product  $j_1 \otimes j_2 \otimes j_3$  can be decomposed in two ways,

$$\begin{aligned}(j_1 \otimes j_2) \otimes j_3 &= \left(\bigoplus_{J_{12}} J_{12}\right) \otimes j_3 = \bigoplus_J \left(\bigoplus_{J_{12}} J\right) = \bigoplus_J (\mathbb{C}^{N(J, j_3)} \otimes J) \\ j_1 \otimes (j_2 \otimes j_3) &= j_1 \otimes \left(\bigoplus_{J_{23}} J_{23}\right) = \bigoplus_J \left(\bigoplus_{J_{23}} J\right) = \bigoplus_J (\mathbb{C}^{N(J, j_3)} \otimes J)\end{aligned}\tag{7.3}$$

with

$$J_{12} \in \{0, 1, 2\} \quad J_{23} - j_3 \in \{-1, 0, 1\} \quad J - j_3 \in \{0, \pm 1, \pm 2\}\tag{7.4}$$

The tensor product for the gauge symmetries decomposes

$$1 \otimes j_3 = \bigoplus_J (\mathbb{C}^{N_{\text{gauge}}(J, j_3)} \otimes \mathbf{J}) \quad J - j_3 \in \{-1, 0, 1\}\tag{7.5}$$

The representations that occur in the decompositions are listed in Table 1. The physical degrees of freedom are the representations with  $N_{\text{phys}} = N - N_{\text{gauge}} > 0$ . The physical representations are listed in Table 2. The infinite series are parametrized by  $j$  rather than  $j_R$  so that the symmetry  $j_L \leftrightarrow j_R$  becomes  $j \leftrightarrow -j$ .

## 8 Five ODEs

### 8.1 $\mathfrak{su}(2)$ notation

The  $\mathfrak{su}(2)$  generators in the  $j = 1/2$  representation are

$$L_a^{(1/2)} = \mu_a = \frac{i\sigma_a}{2} \quad [\mu_a, \mu_b] = -\epsilon_{ab}^{\phantom{ab}c} \mu_c\tag{8.1}$$

The generators  $L_a$  of a general representation satisfy the same commutation relations,

$$[L_a, L_b] = -\epsilon_{ab}^{\phantom{ab}c} L_c\tag{8.2}$$

| $J - j_3$ | $j_3$              | $J_{12}$ | $J_{23} - j_3$ | $N$ | $N_{\text{gauge}}$ | $N_{\text{phys}}$ |
|-----------|--------------------|----------|----------------|-----|--------------------|-------------------|
| 0         | 0                  | 0        | 1              | 1   | 0                  | 1                 |
| 0         | $\frac{1}{2}$      | 0, 1     | 0, 1           | 2   | 1                  | 1                 |
| 0         | $\geq 1$           | 0, 1, 2  | -1, 0, 1       | 3   | 1                  | 2                 |
| 1         | 0                  | 1        | 1              | 1   | 1                  | 0                 |
| 1         | $\geq \frac{1}{2}$ | 1, 2     | 0, 1           | 2   | 1                  | 1                 |
| -1        | 1                  | 1        | 0              | 1   | 1                  | 0                 |
| -1        | $\geq \frac{3}{2}$ | 1, 2     | -1, 0          | 2   | 1                  | 1                 |
| 2         | $\geq 0$           | 2        | 1              | 1   | 0                  | 1                 |
| -2        | $\geq 2$           | 2        | -1             | 1   | 0                  | 1                 |

Table 1: Decomposition of  $\mathbf{1} \otimes \mathbf{1} \otimes \mathbf{j}_{\mathbf{R}}$ .

|                      | $j_L$              | $j_R$              |                       | $J_{12}$ | $J_{23}$                                            | $N$ | $N_{\text{gauge}}$ | $N_{\text{phys}}$ |
|----------------------|--------------------|--------------------|-----------------------|----------|-----------------------------------------------------|-----|--------------------|-------------------|
| <b>1</b>             | 0                  | 0                  |                       | 0        | 1                                                   | 1   | 0                  | 1                 |
| <b>2</b>             | $\frac{1}{2}$      | $\frac{1}{2}$      |                       | 0, 1     | $\frac{1}{2}, \frac{3}{2}$                          | 2   | 1                  | 1                 |
| <b>3<sub>j</sub></b> | $j - \frac{1}{2}$  | $j - \frac{1}{2}$  | $\frac{3}{2} \leq j$  | 0, 1, 2  | $j - \frac{3}{2}, j - \frac{1}{2}, j + \frac{1}{2}$ | 3   | 1                  | 2                 |
| <b>2<sub>j</sub></b> | $j$                | $j - 1$            | $\frac{3}{2} \leq j$  | 1, 2     | $j - 1, j$                                          | 2   | 1                  | 1                 |
|                      | $-j - 1$           | $-j$               | $j \leq -\frac{3}{2}$ | 1, 2     | $-j - 1, -j$                                        | 2   | 1                  | 1                 |
| <b>1<sub>j</sub></b> | $j + \frac{1}{2}$  | $j - \frac{3}{2}$  | $\frac{3}{2} \leq j$  | 2        | $j - \frac{1}{2}$                                   | 1   | 0                  | 1                 |
|                      | $-j - \frac{3}{2}$ | $-j + \frac{1}{2}$ | $j \leq -\frac{3}{2}$ | 2        | $-j - \frac{1}{2}$                                  | 1   | 0                  | 1                 |

Table 2: The physical representations  $N_{\text{phys}} = N - N_{\text{gauge}} > 0$ .

The Casimir operator is

$$C = -\frac{1}{2}L^a L_a \quad (8.3)$$

using  $\delta_{ab}$  to raise/lower indices. The Casimir for the irreducible representation  $j$  is

$$C_j = \frac{1}{2}j(j+1) \quad (8.4)$$

The adjoint representation is  $j = 1$ ,

$$L_a^{(1)} v_b = \epsilon_{ab}^c v_c \quad C_1 = 1 \quad (8.5)$$

## 8.2 The representation $\{B_i\}$

The Dirac matrices on  $S^3$  form an  $\mathfrak{su}(2)$ -valued 1-form which can be written

$$\hat{\gamma}_i(\hat{x}) = \hat{\gamma}_i^a(\hat{x})\mu_a \quad \hat{\gamma}_i^a \hat{\gamma}_a^j = \delta_i^j \quad \hat{\gamma}_i^a \hat{\gamma}_b^i = \delta_b^a \quad (8.6)$$

where indices are raised/lowered with  $\hat{g}_{ij}$  and  $\delta_{ab}$ . The gauge field perturbation  $B_i$  can be written

$$B_i(\hat{x}) = B_i^a(\hat{x})\mu_a = B_{ab}(\hat{x})\hat{\gamma}_i^b\mu^a \quad (8.7)$$

making explicit the representation

$$\{B_{ab}(\hat{x})\} = \oplus_{j_3}(j_1 \otimes j_2 \otimes j_3, j_3) \quad j_1 = j_2 = 1 \quad (8.8)$$

Let  $L_a^1, L_a^2, L_a^3$  be the generators of the representations  $j_1, j_2, j_3$ .

$$L_a^1 B_{bc} = \epsilon_{ab}{}^d B_{dc} \quad L_a^2 B_{bc} = \epsilon_{ac}{}^d B_{bd} \quad L_a^3 B_{bc} = \frac{1}{2}\hat{\gamma}_a^i(\hat{x})\hat{\partial}_i B_{bc} \quad (8.9)$$

The last formula is verified by noting that  $L_a^3$  is the generator of left multiplication acting on functions so should act as a right-invariant vector field and by checking at the north pole.

$$\hat{\gamma}_a^i(\hat{N}) = \delta_a^i \quad g_{\hat{N}+\epsilon^a \hat{\gamma}_a^i/2} = 1 - \epsilon^a \mu_a \quad (8.10)$$

The Casimirs of the individual factors are

$$C_{j_1} = C_{j_2} = 1 \quad C_{j_3} = \frac{1}{2}j_3(j_3 + 1) \quad (8.11)$$

Write

$$\begin{aligned} L_a^{12} &= L_a^1 + L_a^2 & C_{12} &= -\frac{1}{2}\delta^{ab}L_a^{12}L_b^{12} = -\frac{1}{2}\delta^{ab}(L_a^1 + L_a^2)(L_b^1 + L_b^2) \\ L_a^{23} &= L_a^2 + L_a^3 & C_{23} &= -\frac{1}{2}\delta^{ab}L_a^{23}L_b^{23} = -\frac{1}{2}\delta^{ab}(L_a^2 + L_a^3)(L_b^2 + L_b^3) \end{aligned} \quad (8.12)$$

In the decompositions (7.3)

$$C_{12} = \frac{1}{2}J_{12}(J_{12} + 1) \quad C_{23} = \frac{1}{2}J_{23}(J_{23} + 1) \quad (8.13)$$

### 8.3 $\Gamma$ and $*\hat{\nabla}$ in terms of Casimirs

The operator  $\Gamma$  defined in (6.18) is

$$\Gamma B_i = \epsilon_i{}^{jk}[\hat{\gamma}_j, B_k] = \epsilon_i{}^{jk}[\hat{\gamma}_j^c \mu_c, B_{a'b'}\hat{\gamma}_k^{b'}\mu^{a'}] = -\epsilon_i{}^{jk}\hat{\gamma}_j^c \hat{\gamma}_k^{b'} B_{a'b'}\epsilon_c{}^{a'}\mu^a \quad (8.14)$$

Now use

$$\epsilon_{abc} = \epsilon_{ijk}\hat{\gamma}_a^i \hat{\gamma}_b^j \hat{\gamma}_c^k \quad (8.15)$$

to get

$$\Gamma(B_{ab}\mu^a \hat{\gamma}_i^b) = -\epsilon_{i'}{}^{jk}\hat{\gamma}_b^{i'} \gamma_j^c \hat{\gamma}_k^{b'} \epsilon_c{}^{a'} B_{a'b'}\mu^a \hat{\gamma}_i^b = -\epsilon^{cb'} \epsilon_c{}^{a'} B_{a'b'}\mu^a \hat{\gamma}_i^b \quad (8.16)$$

$$\Gamma B_{ab} = -\delta^{cd}\epsilon_{ca}{}^{a'} \epsilon_{ab}{}^{b'} B_{a'b'}$$

$$\Gamma = -\delta^{cd}L_c^1 L_d^2 = C_{12} - C_{j_1} - C_{j_2} = C_{12} - 2 \quad (8.17)$$

Next, define

$$*d = *\hat{\nabla} - \Gamma \quad (8.18)$$

$$\begin{aligned}
*d(B_{ab}\hat{\gamma}_i^b\mu^a) &= \epsilon_i^{jk}\hat{\partial}_j(B_{ab}\hat{\gamma}_k^b\mu^a) = \epsilon_i^{jk}(\hat{\partial}_j B_{ab})\hat{\gamma}_k^b\mu^a + \epsilon_i^{jk}B_{ab}\hat{\partial}_j\hat{\gamma}_k^b\mu^a \\
&= -\epsilon_c^{b\ b'}(\hat{\gamma}_c^j\hat{\partial}_j B_{ab'})\hat{\gamma}_i^b\mu^a + \epsilon_{i'}^{jk}\hat{\gamma}_b^{i'}\hat{\partial}_j\hat{\gamma}_k^{b'}B_{ab'}\hat{\gamma}_i^b\mu^a \\
*dB_{ab} &= -2\delta^{cd}L_c^2L_d^3 + A_b^{b'}B_{ab'} \quad A_b^{b'} = \epsilon_{i'}^{jk}\hat{\gamma}_b^{i'}\hat{\partial}_j\hat{\gamma}_k^{b'} \\
A_b^{b'}\mu_{b'} &= \epsilon_{i'}^{jk}\hat{\gamma}_b^{i'}\hat{\partial}_j\hat{\gamma}_k^{b'} = \epsilon_{i'}^{jk}\hat{\gamma}_b^{i'}\frac{1}{2}\hat{\partial}_{[j}\hat{\gamma}_{k]} = -\epsilon_{i'}^{jk}\hat{\gamma}_b^{i'}[\hat{\gamma}_j, \hat{\gamma}_k] \\
&= \epsilon_{i'}^{jk}\hat{\gamma}_b^{i'}\epsilon_{jk}^i\hat{\gamma}_i = 2\gamma_b^i\hat{\gamma}_i = 2\gamma_b^i\hat{\gamma}_i^c\mu_c = 2\mu_b \\
A_b^{b'} &= 2\delta_b^{b'} \\
*d &= 2(C_{23} - C_{j_2} - C_{j_3}) + 2 = 2(C_{23} - C_{j_3})
\end{aligned} \tag{8.19}$$

#### 8.4 Wigner 6-j symbol and Racah W-coefficient

The two decompositions (7.3) give two canonical bases for  $\mathbb{C}^{N(J,j_3)}$ ,

$$\mathbb{C}^{N(J,j_3)} = \bigoplus_{J_{12}} \hat{e}_{12}(J_{12}) \otimes \mathbb{C} = \bigoplus_{J_{23}} \hat{e}_{23}(J_{23}) \otimes \mathbb{C} \tag{8.20}$$

$C_{12}$  is diagonal in the first basis,  $C_{23}$  in the second.

$$C_{12} \hat{e}_{12}(J_{12}) = \frac{1}{2}J_{12}(J_{12} + 1) \hat{e}_{12}(J_{12}) \quad C_{23} \hat{e}_{23}(J_{23}) = \frac{1}{2}J_{23}(J_{23} + 1) \hat{e}_{23}(J_{23}) \tag{8.21}$$

But they cannot be diagonalized simultaneously unless  $N = 1$ . The two bases are related by a matrix,

$$\hat{e}_{12}(J_{12}) = \sum_{J_{23}} U(J_{12}, J_{23}) \hat{e}_{23}(J_{23}) \tag{8.22}$$

The matrix elements  $U(J_{12}, J_{23})$  are called the *recoupling coefficients*. Traditionally the recoupling coefficients are written

$$U(J_{12}, J_{23}) = \langle (j_1, (j_2 j_3) J_{23}) J \mid ((j_1 j_2) J_{12} j_3) J \rangle \tag{8.23}$$

They are related to the Wigner 6-j symbol and the Racah W-coefficient,

$$\frac{U(J_{12}, J_{23})}{\sqrt{(2J_{12} + 1)(2J_{23} + 1)}} = (-1)^{j_1 + j_2 + j_3 + J} \left\{ \begin{matrix} j_1 & j_2 & J_{12} \\ j_3 & J & J_{23} \end{matrix} \right\} = W(j_1 j_2 J j_3; J_{12} J_{23}) \tag{8.24}$$

Given  $U$ , the two Casimirs can be written as matrices in the same basis,

$$C_{12} = \frac{1}{2}J_{12}(J_{12} + 1) \quad C_{23} = U \frac{1}{2}J_{23}(J_{23} + 1) U^t \tag{8.25}$$

Racah's algorithm for the W-coefficient [1] is:

$$\begin{aligned}
W(j_1 j_2 J j_3; J_{12} J_{23}) &= W(abcd; ef) \\
a = j_1 \quad b = j_2 \quad c = J \quad d = j_3 \quad e = J_{12} \quad f = J_{23}
\end{aligned} \tag{8.26}$$

$$W(abcd; ef) = \Delta(a, b, e) \Delta(c, d, e) \Delta(a, c, f) \Delta(b, d, f) w(abcd; ef)$$

$$\Delta(a, b, c) = \left[ \frac{(a + b - c)!(a - b + c)!(-a + b + c)!}{(a + b + c + 1)!} \right]^{1/2} \tag{8.27}$$

$$w(abcd; ef) = \sum_z \frac{(-1)^{z+\beta_1} (z+1)!}{\prod_{i=1}^4 (z - \alpha_i)! \prod_{i=1}^3 (\beta_i - z)!} \quad (8.28)$$

The sum is over integers  $z$  in the range

$$\begin{aligned} \max(\alpha_1, \alpha_2, \alpha_3, \alpha_4) &\leq z \leq \min(\beta_1, \beta_2, \beta_3) \\ \alpha_1 &= a + b + e & \alpha_2 &= c + d + e & \alpha_3 &= a + c + f & \alpha_4 &= b + d + f \\ \beta_1 &= a + b + c + d & \beta_2 &= a + d + e + f & \beta_3 &= b + c + e + f \end{aligned} \quad (8.29)$$

### 8.5 The five $\mathbf{K}(z)$ matrices

The quadratic action is (6.15)

$$\frac{1}{\hbar} S_2 = \frac{1}{\epsilon g^2} \int \text{tr}(\partial_z B_i \partial_z B^i - B_i \mathbf{K} B^i) \sqrt{-\hat{g}} d^3 \hat{x} dz \quad (8.30)$$

with equation of motion

$$\left( \frac{d^2}{dz^2} + \mathbf{K}(z) \right) B_i = 0 \quad (8.31)$$

Equation (6.22) gives  $\mathbf{K}(z)$  as

$$\mathbf{K} = (\Gamma^2 - \Gamma) b^2 + \left( * \hat{\nabla} \Gamma + \Gamma * \hat{\nabla} \right) \epsilon b + [(* \hat{\nabla})^2 + \Gamma] \epsilon^2 \quad (8.32)$$

now expressed in terms of Casimirs,

$$\Gamma = C_{12} - 2 \quad * \hat{\nabla} - \Gamma = 2C_{23} - j_3(j_3 + 1) \quad (8.33)$$

For each irreducible  $(j_L, j_R)$  occuring in the space  $\{B_i\}$  of gauge field perturbations,  $\mathbf{K}(z)$  is an  $N \times N$  matrix acting on  $\mathbb{C}^N$ ,  $N = N(j_L, j_R)$ .

The  $\mathbf{K}(z)$  matrix for **Case 1**  $(j_L, j_R) = (0, 0)$  is calculated by hand below. The  $\mathbf{K}(z)$  matrices for the other four sets of representations listed in Table 2 are calculated in Sagemath in the notebook *K(z) matrices*. For the series of representations indexed by  $j$ , the parameter  $p$  is defined as

$$p^2 = 4\epsilon^2 C_{(j_L, j_R)} = 2\epsilon^2 [j_L(j_L + 1) + j_R(j_R + 1)] \quad (8.34)$$

The representations are indexed by  $(j_L, j_R) = (J, j_3)$ .

#### Case 1

| $j_L$    | $j_R$ | $J_{12}$ | $J_{23} - j_3$ | $N$ | $N_{\text{gauge}}$ | $N_{\text{phys}}$ |
|----------|-------|----------|----------------|-----|--------------------|-------------------|
| <b>1</b> | 0     | 0        | 1              | 1   | 0                  | 1                 |

$$\begin{aligned} C_{12} &= 0 & C_{23} &= 1 & \Gamma &= -2 & * \hat{\nabla} &= 0 \\ \mathbf{K} &= 6b^2 - 2\epsilon^2 \end{aligned} \quad (8.35)$$

**Case 2**

|          | $j_L$         | $j_R$         |  | $J_{12}$ | $J_{23} - j_3$ | $N$ | $N_{\text{gauge}}$ | $N_{\text{phys}}$ |
|----------|---------------|---------------|--|----------|----------------|-----|--------------------|-------------------|
| <b>2</b> | $\frac{1}{2}$ | $\frac{1}{2}$ |  | 0, 1     | 0, 1           | 2   | 1                  | 1                 |

$$\mathbf{K} = \begin{pmatrix} 6 & 0 \\ 0 & 2 \end{pmatrix} b^2 + \begin{pmatrix} 0 & -3\sqrt{2} \\ -3\sqrt{2} & 0 \end{pmatrix} \epsilon b + \begin{pmatrix} 0 & 0 \\ 0 & 1 \end{pmatrix} \epsilon^2 \quad (8.36)$$

**Case 3<sub>j</sub>**

|                      | $j_L$             | $j_R$             |                      | $J_{12}$ | $J_{23} - j_3$ | $N$ | $N_{\text{gauge}}$ | $N_{\text{phys}}$ |
|----------------------|-------------------|-------------------|----------------------|----------|----------------|-----|--------------------|-------------------|
| <b>3<sub>j</sub></b> | $j - \frac{1}{2}$ | $j - \frac{1}{2}$ | $\frac{3}{2} \leq j$ | 0, 1, 2  | -1, 0, 1       | 3   | 1                  | 2                 |

$$\mathbf{K}_2 = \begin{pmatrix} 6 & 0 & 0 \\ 0 & 2 & 0 \\ 0 & 0 & 0 \end{pmatrix} b^2 + \begin{pmatrix} 0 & -6 & 0 \\ -6 & 0 & 0 \\ 0 & 0 & 0 \end{pmatrix} \sigma b + \begin{pmatrix} \alpha^2 & 0 & \alpha \\ 0 & \alpha^2 + 1 & 0 \\ \alpha & 0 & 1 \end{pmatrix} 2\sigma^2 \quad (8.37)$$

$$p^2 = 4\epsilon^2 \left( j^2 - \frac{1}{4} \right) \quad \sigma = \sqrt{\frac{2}{3}} \sqrt{j^2 - \frac{1}{4}} \epsilon = \frac{p}{\sqrt{6}} \quad \alpha = \sqrt{2} \sqrt{\frac{j^2 - 1}{j^2 - \frac{1}{4}}}$$

**Case 2<sub>j</sub>**

|                      | $j_L$    | $j_R$   |                       | $J_{12}$ | $J_{23} - j_3$ | $N$ | $N_{\text{gauge}}$ | $N_{\text{phys}}$ |
|----------------------|----------|---------|-----------------------|----------|----------------|-----|--------------------|-------------------|
| <b>2<sub>j</sub></b> | $j$      | $j - 1$ | $\frac{3}{2} \leq j$  | 1, 2     | 0, 1           | 2   | 1                  | 1                 |
|                      | $-j - 1$ | $-j$    | $j \leq -\frac{3}{2}$ | 1, 2     | -1, 0          | 2   | 1                  | 1                 |

$$\mathbf{K} = \begin{pmatrix} 2 & 0 \\ 0 & 0 \end{pmatrix} b^2 + \begin{pmatrix} -1 & 0 \\ 0 & 1 \end{pmatrix} 2\sigma b + \begin{pmatrix} \alpha^2 & \alpha \\ \alpha & 1 \end{pmatrix} 2\sigma^2 \quad (8.38)$$

$$p^2 = 4\epsilon^2 j^2 \quad \sigma = \epsilon j = \frac{1}{2} p \quad \alpha = \sqrt{1 - \frac{1}{j^2}}$$

**Case 1<sub>j</sub>**

|                      | $j_L$              | $j_R$              |                       | $J_{12}$ | $J_{23} - j_3$ | $N$ | $N_{\text{gauge}}$ | $N_{\text{phys}}$ |
|----------------------|--------------------|--------------------|-----------------------|----------|----------------|-----|--------------------|-------------------|
| <b>1<sub>j</sub></b> | $j + \frac{1}{2}$  | $j - \frac{3}{2}$  | $\frac{3}{2} \leq j$  | 2        | 1              | 1   | 0                  | 1                 |
|                      | $-j - \frac{3}{2}$ | $-j + \frac{1}{2}$ | $j \leq -\frac{3}{2}$ | 2        | -1             | 1   | 0                  | 1                 |

$$\mathbf{K} = 4\sigma b + 4\alpha^2 \sigma^2$$

$$p^2 = 4\epsilon^2 \left( j^2 + \frac{3}{4} \right) \quad \sigma = \epsilon j = \frac{1}{2} \sqrt{p^2 - 3\epsilon^2} \quad \alpha = \sqrt{1 + \frac{1}{4j^2}} \quad (8.39)$$

## 8.6 Gauge symmetries

A gauge variation of the classical solution is a solution of the equation of motion that is first order in  $b(z)$ .

$$w_{\text{gauge}}(z) = w_1 b(z) + w_0 \quad (8.40)$$

Use

$$b'' = 2\epsilon^2 b - 2b^3 \quad (8.41)$$

and write

$$\mathbf{K} = \mathbf{K}_2 b^2 + \mathbf{K}_1 b + \mathbf{K}_0 \quad (8.42)$$

to calculate

$$\begin{aligned} 0 &= \frac{d^2 w}{dz^2} + \mathbf{K}(z)w \\ &= w_1(2\epsilon^2 b - 2b^3) + (\mathbf{K}_2 b^2 + \mathbf{K}_1 b + \mathbf{K}_0)(w_1 b + w_0) \\ &= (\mathbf{K}_2 - 2)w_1 b^3 + (\mathbf{K}_2 w_0 + \mathbf{K}_1 w_1)b^2 \\ &\quad + (2\epsilon^2 w_1 + \mathbf{K}_0 w_1 + \mathbf{K}_1 w_0)b + \mathbf{K}_0 w_0 \end{aligned} \quad (8.43)$$

So the coefficients  $w_0, w_1$  are the solutions of

$$\begin{aligned} 0 &= \mathbf{K}_0 w_0 \\ 0 &= (\mathbf{K}_2 - 2)w_1 \\ 0 &= \mathbf{K}_2 w_0 + \mathbf{K}_1 w_1 \\ 0 &= \mathbf{K}_1 w_0 + (\mathbf{K}_0 + 2\epsilon^2)w_1 \end{aligned} \quad (8.44)$$

**Case 2**

$$\mathbf{K}_2 = \begin{pmatrix} 6 & 0 \\ 0 & 2 \end{pmatrix} \quad \mathbf{K}_1 = \begin{pmatrix} 0 & -3\sqrt{2} \\ -3\sqrt{2} & 0 \end{pmatrix} \epsilon \quad \mathbf{K}_0 = \begin{pmatrix} 0 & 0 \\ 0 & 1 \end{pmatrix} \epsilon^2 \quad (8.45)$$

$$w_1 = B \begin{pmatrix} 0 \\ 1 \end{pmatrix} \quad w_0 = A \begin{pmatrix} 1 \\ 0 \end{pmatrix} \quad 0 = A \begin{pmatrix} 6 \\ 0 \end{pmatrix} + B \begin{pmatrix} -3\sqrt{2} \\ 0 \end{pmatrix} \epsilon \quad (8.46)$$

$$\begin{aligned} A &= \frac{\epsilon}{\sqrt{2}} B \quad 0 = A \begin{pmatrix} 0 \\ -3\sqrt{2} \end{pmatrix} \epsilon + B \begin{pmatrix} 0 \\ 3 \end{pmatrix} \epsilon^2 = 0 \\ w_{\text{gauge}} &= \begin{pmatrix} 0 \\ 1 \end{pmatrix} b + \begin{pmatrix} 1 \\ 0 \end{pmatrix} \frac{\epsilon}{\sqrt{2}} \end{aligned} \quad (8.47)$$

**Case 3<sub>j</sub>**

$$\mathbf{K}_2 = \begin{pmatrix} 6 & 0 & 0 \\ 0 & 2 & 0 \\ 0 & 0 & 0 \end{pmatrix} \quad \mathbf{K}_1 = \begin{pmatrix} 0 & -6 & 0 \\ -6 & 0 & 0 \\ 0 & 0 & 0 \end{pmatrix} \sigma_3 \quad \mathbf{K}_0 = \begin{pmatrix} \alpha_3^2 & 0 & \alpha_3 \\ 0 & \alpha_3^2 + 1 & 0 \\ \alpha_3 & 0 & 1 \end{pmatrix} 2\sigma_3^2$$

$$\sigma_3 = \sqrt{\frac{2}{3}} \sqrt{j^2 - \frac{1}{4}} \epsilon \quad \alpha_3 = \sqrt{2} \sqrt{\frac{j^2 - 1}{j^2 - \frac{1}{4}}} \quad (8.48)$$

$$w_1 = B \begin{pmatrix} 0 \\ 1 \\ 0 \end{pmatrix} \quad w_0 = A \begin{pmatrix} 1 \\ 0 \\ -\alpha_3 \end{pmatrix} \quad (8.49)$$

$$0 = A \begin{pmatrix} 6 \\ 0 \\ 0 \end{pmatrix} + B \begin{pmatrix} -6\sigma_3 \\ 0 \\ 0 \end{pmatrix} \quad A = \sigma_3 B$$

$$0 = A \begin{pmatrix} 0 \\ -6\sigma_3 \\ 0 \end{pmatrix} + B \begin{pmatrix} 0 \\ 2\epsilon^2 + (\alpha_3^2 + 1)2\sigma_3^2 \\ 0 \end{pmatrix} \quad (8.50)$$

$$0 = B [-6\sigma_3^2 + 2\epsilon^2 + 2\sigma_3^2(\alpha_3^2 + 1)] = 2B [\epsilon^2 + \sigma_3(\alpha_3^2 - 2)]$$

$$= 2B\epsilon^2 \left[ 1 + \frac{2}{3} \left( j^2 - \frac{1}{4} \right) 2 \left( \frac{-\frac{3}{4}}{j^2 - \frac{1}{4}} \right) \right] \quad (8.51)$$

$$= 0$$

$$w_{\text{gauge}} = \begin{pmatrix} 0 \\ 1 \\ 0 \end{pmatrix} b + \begin{pmatrix} 1 \\ 0 \\ -\alpha_3 \end{pmatrix} \sigma_3 \quad (8.52)$$

**Case 2<sub>j</sub>**

$$\mathbf{K}_2 = \begin{pmatrix} 2 & 0 \\ 0 & 0 \end{pmatrix} \quad \mathbf{K}_1 = \begin{pmatrix} -1 & 0 \\ 0 & 1 \end{pmatrix} 2\sigma_2 \quad \mathbf{K}_0 = \begin{pmatrix} \alpha_2^2 & \alpha_2 \\ \alpha_2 & 1 \end{pmatrix} 2\sigma_2^2 \quad (8.53)$$

$$\sigma_2 = \epsilon j \quad \alpha_2 = \sqrt{1 - \frac{1}{j^2}}$$

$$w_1 = B \begin{pmatrix} 1 \\ 0 \end{pmatrix} \quad w_0 = A \begin{pmatrix} 1 \\ -\alpha_2 \end{pmatrix}$$

$$0 = A \begin{pmatrix} 2 \\ 0 \end{pmatrix} + 2\sigma_2 \begin{pmatrix} -B \\ 0 \end{pmatrix} \quad A = \sigma_2 B \quad (8.54)$$

$$0 = B \begin{pmatrix} 2\epsilon^2 + 2\alpha_2^2\sigma_2^2 \\ 2\alpha_2\sigma_2^2 \end{pmatrix} + \sigma_2 B \begin{pmatrix} -2\sigma_2 \\ -2\alpha_2\sigma_2 \end{pmatrix} = 2B \begin{pmatrix} \epsilon^2 + \alpha_2^2\sigma_2^2 - \sigma_2^2 \\ 0 \end{pmatrix} = 0$$

$$w_{\text{gauge}} = \begin{pmatrix} 1 \\ 0 \end{pmatrix} b + \begin{pmatrix} 1 \\ -\alpha_2 \end{pmatrix} \sigma_2 \quad (8.55)$$

## 9 Time-translation zero-mode

The zero-mode is written as a free particle in the reparametrized time  $\tilde{z}$  given by

$$\frac{d\tilde{z}}{dz} = \frac{1}{\text{cn}'(z)^2} \quad (9.1)$$

The following calculates the periodicities of  $\tilde{z}(z)$ . The results are not used in the paper, but will be relevant for further investigation of the zero-mode integral.

The identities in section 9.1 below are used to integrate.

$$\begin{aligned}
\tilde{z} &= \int \frac{dz}{\operatorname{sn}(z)^2 \operatorname{dn}(z)^2} = \int \frac{k^2 \operatorname{sn}(z)^2 + \operatorname{dn}(z)^2}{\operatorname{sn}(z)^2 \operatorname{dn}(z)^2} dz \\
&= k^2 \int \operatorname{nd}^2 dz + \int \operatorname{ns}^2 dz \\
&= \frac{k^2}{k'^2} (\mathcal{E} - k^2 \operatorname{sn} \operatorname{cd}) + z - \operatorname{dn} \operatorname{cs} - \mathcal{E} \\
&= \left( \frac{k^2}{k'^2} - 1 \right) \mathcal{E} + z - \frac{k^4}{k'^2} \frac{\operatorname{sn} \operatorname{cn}}{\operatorname{dn}} - \frac{\operatorname{dn} \operatorname{cn}}{\operatorname{sn}} \\
&= \left( \frac{k^2}{k'^2} - 1 \right) \mathcal{E} + z - \frac{\operatorname{cn}}{k'^2 \operatorname{sn} \operatorname{dn}} (k^4 \operatorname{sn}^2 + k'^2 \operatorname{dn}^2)
\end{aligned} \tag{9.2}$$

$$k^4 \operatorname{sn}^2 + k'^2 \operatorname{dn}^2 = k^4 \operatorname{sn}^2 + k'^2 (1 - k^2 \operatorname{sn}^2) = k'^2 + k^2 (k^2 - k'^2) \operatorname{sn}^2 \tag{9.3}$$

$$\begin{aligned}
\tilde{z} &= \left( \frac{k^2}{k'^2} - 1 \right) \mathcal{E} + z - \frac{\operatorname{cn}}{\operatorname{sn} \operatorname{dn}} - \frac{\operatorname{cn}}{k'^2 \operatorname{sn} \operatorname{dn}} k^2 (k^2 - k'^2) \operatorname{sn}^2 \\
&= -\frac{\operatorname{cn}}{\operatorname{sn} \operatorname{dn}} + z + \left( \frac{k^2}{k'^2} - 1 \right) \left( \mathcal{E} - k^2 \frac{\operatorname{cn} \operatorname{sn}}{\operatorname{dn}} \right)
\end{aligned} \tag{9.4}$$

So  $\tilde{z}$  has periodicities

$$\begin{aligned}
\tilde{z}(z + 2K) - \tilde{z}(z) &= 2K + \left( \frac{k^2}{k'^2} - 1 \right) (\mathcal{E}(z + 2K) - \mathcal{E}(z)) \\
&= 2K + \left( \frac{k^2}{k'^2} - 1 \right) 2E
\end{aligned} \tag{9.5}$$

$$\begin{aligned}
\tilde{z}(z + 2K'i) - \tilde{z}(z) &= 2K'i + \left( \frac{k^2}{k'^2} - 1 \right) (\mathcal{E}(z + 2K'i) - \mathcal{E}(z)) \\
&= 2K'i + \left( \frac{k^2}{k'^2} - 1 \right) (2K' - 2E')i
\end{aligned} \tag{9.6}$$

## 9.1 More on Jacobi elliptic functions

These identities are from the DLMF [2, Chapters 22 and 19].

$\operatorname{sn}(z, k)$  **and**  $\operatorname{dn}(z, k)$

$$\begin{aligned}
\operatorname{sn}^2 + \operatorname{cn}^2 &= 1 & k^2 \operatorname{sn}^2 + \operatorname{dn}^2 &= 1 \\
\operatorname{sn}(z) &\sim z + O(z^3) & \operatorname{dn}(z) &\sim 1 + O(z^2)
\end{aligned} \tag{9.7}$$

$$\begin{aligned}
\operatorname{cn}' &= -\operatorname{sn} \operatorname{dn} & \operatorname{dn}' &= -k^2 \operatorname{sn} \operatorname{cn} \\
\operatorname{dn}'' &= (1 + k'^2) \operatorname{dn} - 2 \operatorname{dn}^3 & (\operatorname{dn}')^2 &= (1 - \operatorname{dn}^2)(\operatorname{dn}^2 - k'^2)
\end{aligned} \tag{9.8}$$

### half-periods

$$\begin{aligned} \operatorname{cn}(z + 2K) &= -\operatorname{cn}(z) & \operatorname{sn}(z + 2K) &= -\operatorname{sn}(z) & \operatorname{dn}(z + 2K) &= \operatorname{dn}(z) \\ \operatorname{cn}(z + 2K'i) &= -\operatorname{cn}(z) & \operatorname{sn}(z + 2K'i) &= \operatorname{sn}(z) & \operatorname{dn}(z + 2K'i) &= -\operatorname{dn}(z) \end{aligned} \quad (9.9)$$

### the other Jacobi elliptic functions

$$\operatorname{nc} = \frac{1}{\operatorname{cn}} \quad \operatorname{ns} = \frac{1}{\operatorname{sn}} \quad \operatorname{nd} = \frac{1}{\operatorname{dn}} \quad \operatorname{cd} = \frac{\operatorname{cn}}{\operatorname{dn}} \quad \operatorname{cs} = \frac{\operatorname{cn}}{\operatorname{sn}} \quad (9.10)$$

### Jacobi's amplitude function $\phi = \operatorname{am}(z, k)$

$$\begin{aligned} \phi = \operatorname{am}(z) &= \int_0^z \operatorname{dn} & \operatorname{sn}(z) &= \sin(\phi) & \operatorname{cn}(z) &= \cos(\phi) \\ \operatorname{am}(z + 2K) &= \operatorname{am}(z) + \pi & \operatorname{am}(2K) &= \pi \end{aligned} \quad (9.11)$$

### Jacobi epsilon function $\mathcal{E}(z, k)$ and zeta function $\mathcal{Z}(z, k)$

$$\mathcal{E}(z) = \int_0^z \operatorname{dn}^2 = k^2 \operatorname{sn} \operatorname{cd} + k'^2 \int \operatorname{nd}^2 = z - \operatorname{dn} \operatorname{cs} - \int \operatorname{ns}^2 \quad (9.12)$$

$$\mathcal{Z}(z) = \mathcal{E}(z) - \frac{E(k)}{K(k)} z = \frac{\theta'_0}{\theta_0} \quad (9.13)$$

$E(k)$  is the complete elliptic integral of the second kind,

$$E(k) = \mathcal{E}(K) = E(\pi/2, k) \quad E(\phi, k) = \mathcal{E}(z, k) \quad (9.14)$$

satisfying

$$EK' + E'K - KK' = \frac{\pi}{2} \quad (9.15)$$

$$\mathcal{E}(-z) = -\mathcal{E}(z) \quad \mathcal{E}(z) = z + O(z^3) \quad (9.16)$$

$$\begin{aligned} \mathcal{E}(u + v) &= \mathcal{E}(u) + \mathcal{E}(v) - k^2 \operatorname{sn}(u) \operatorname{sn}(v) \operatorname{sn}(u + v) \\ \mathcal{Z}(u + v) &= \mathcal{Z}(u) + \mathcal{Z}(v) - k^2 \operatorname{sn}(u) \operatorname{sn}(v) \operatorname{sn}(u + v) \end{aligned} \quad (9.17)$$

$$\mathcal{Z}(z + 2K) = \mathcal{Z}(z) \quad \mathcal{Z}(z + 2K'i) = \mathcal{Z}(z) - \frac{\pi}{K} i \quad (9.18)$$

$$\mathcal{E}(z + 2K) = \mathcal{E}(z) + 2E \quad \mathcal{E}(z + 2K'i) = \mathcal{E}(z) + 2(K' - E')i \quad (9.19)$$

$$\begin{aligned} \mathcal{E}(z + 2K'i) &= \mathcal{E}(z) + \mathcal{Z}(z + 2K'i) - \mathcal{Z}(z) + \frac{E}{K} 2K'i \\ &= \mathcal{E}(z) - \frac{\pi}{K} i + \frac{E}{K} 2K'i \\ &= \mathcal{E}(z) + \frac{2i}{K} \left( -\frac{\pi}{2} + EK' \right) \\ &= \mathcal{E}(z) + 2(K' - E')i \end{aligned} \quad (9.20)$$

## 10 Classical mechanics analytic in complex time $z$

$$\mathcal{A}(z) = \begin{pmatrix} 0 & -1 \\ \mathbf{K}(z) & 0 \end{pmatrix} \quad \Omega = i \begin{pmatrix} 0 & 1 \\ -1 & 0 \end{pmatrix} \quad (10.1)$$

$$\begin{aligned} \mathcal{A}(z)^t \Omega + \Omega \mathcal{A}(z) &= \begin{pmatrix} 0 & \mathbf{K}(z)^t \\ -1 & 0 \end{pmatrix} i \begin{pmatrix} 0 & 1 \\ -1 & 0 \end{pmatrix} + i \begin{pmatrix} 0 & 1 \\ -1 & 0 \end{pmatrix} \begin{pmatrix} 0 & -1 \\ \mathbf{K}(z) & 0 \end{pmatrix} \\ &= i \begin{pmatrix} \mathbf{K}(z) - \mathbf{K}(z)^t & 0 \\ 0 & 0 \end{pmatrix} \end{aligned} \quad (10.2)$$

$$\mathbf{K}(z) = \mathbf{K}(z)^t \iff \mathcal{A}(z)^t \Omega + \Omega \mathcal{A}(z) = 0 \quad (10.3)$$

## 11 Quantum mechanics analytic in complex time $z$

Canonical commutation relations

$$\begin{aligned} \mathcal{Q} &= \begin{pmatrix} q \\ p \end{pmatrix} \quad \mathcal{Q}^t = (q^t \ p^t) \quad \mathcal{Q}\mathcal{Q}^t = \begin{pmatrix} qq^t & qp^t \\ pq^t & pp^t \end{pmatrix} \\ (\mathcal{Q}\mathcal{Q}^t)^t - \mathcal{Q}\mathcal{Q}^t &= \begin{pmatrix} (qq^t)^t - qq^t & (pq^t)^t - qp^t \\ (qp^t)^t - pq^t & (pp^t)^t - pp^t \end{pmatrix} \end{aligned} \quad (11.1)$$

$$\begin{aligned} (\mathcal{Q}\mathcal{Q}^t)^t - \mathcal{Q}\mathcal{Q}^t = \Omega &\iff \begin{aligned} (qq^t)^t - qq^t &= 0 \\ (pp^t)^t - pp^t &= 0 \\ (pq^t)^t - qp^t &= i \end{aligned} \end{aligned} \quad (11.2)$$

$$\begin{aligned} [(qq^t)^t - qq^t]^{ab} &= q^b q^a - q^a q^b \quad [(pp^t)^t - pp^t]_{ab} = p_b p_a - p_a p_b \\ [(pq^t)^t - qp^t]_b^a &= p_b q^a - q^a p_b \end{aligned} \quad (11.3)$$

$$\begin{aligned} (\mathcal{Q}\mathcal{Q}^t)^t - \mathcal{Q}\mathcal{Q}^t = \Omega &\iff \begin{aligned} [q^a, q^b] &= 0 \\ [p_a, p_b] &= 0 \\ [p_b, q^a] &= i\delta_b^a \end{aligned} \end{aligned} \quad (11.4)$$

Phase-space action

$$\begin{aligned} \frac{1}{2i} \mathcal{Q}^t \Omega \left( \frac{d}{dz} + \mathcal{A} \right) \mathcal{Q} &= \frac{1}{2} (q^t \ p^t) \begin{pmatrix} 0 & 1 \\ -1 & 0 \end{pmatrix} \left( \frac{d}{dz} + \begin{pmatrix} 0 & -1 \\ \mathbf{K}(z) & 0 \end{pmatrix} \right) \begin{pmatrix} q \\ p \end{pmatrix} \\ &= \frac{1}{2} (q^t \ p^t) \begin{pmatrix} 0 & 1 \\ -1 & 0 \end{pmatrix} \begin{pmatrix} \frac{dq}{dz} - p \\ \frac{dp}{dz} + Kq \end{pmatrix} \\ &= -\frac{1}{2} p^t \frac{dq}{dz} + \frac{1}{2} q^t \frac{dp}{dz} + \frac{1}{2} p^t p + \frac{1}{2} q^t K q \end{aligned} \quad (11.5)$$

## 18 Numerical evidence for Property P

### 18.1 Imaginary period monodromy $\mathcal{M}_i$ at $t = K$

Identities for Jacobi elliptic functions. For  $\tau \in \mathbb{R}$ ,

$$\begin{aligned} \operatorname{cn}(K + \tau i, k) &= -k' \operatorname{sd}(\tau i, k) = -k' \operatorname{sd}(\tau, k')i \\ \operatorname{sd}(\tau, k') &= \overline{\operatorname{sd}(\tau, k')} \\ \operatorname{sd}(-\tau, k') &= -\operatorname{sd}(\tau, k') \quad \operatorname{sd}(\tau + 2K, k') = -\operatorname{sd}(\tau, k') \end{aligned} \quad (18.1)$$

Let  $t = K$  and let  $C_K$  be the vertical path passing through  $K$ .

$$z = K + \tau i \quad b(z) = k \operatorname{cn}(z, k) = -kk' \operatorname{sd}(\tau, k')i = F(\tau)i \quad (18.2)$$

$$F(\tau) = -kk' \operatorname{sd}(\tau, k') \quad \mathbf{K}(z) = -\mathbf{K}_2 F(\tau)^2 + \mathbf{K}_0 + \mathbf{K}_1 F(\tau)i \quad (18.3)$$

$$F(\tau) = \overline{F(\tau)} \quad F(-\tau) = -F(\tau) \quad F(\tau + 2K') = -F(\tau) \quad (18.4)$$

Write the propagator along  $C_K$

$$\mathcal{P}(\tau_2, \tau_1) = \mathcal{P}_{C_K}(K + \tau_2 i, K + \tau_1 i) \quad (18.5)$$

The symmetries of  $F(\tau)$  give

$$\mathcal{P}(4K' - \tau_2, 4K' - \tau_1) = \overline{\mathcal{P}(\tau_2, \tau_1)} \quad \mathcal{P}(2K' - \tau_2, 2K' - \tau_1) = \mathcal{R}\mathcal{P}(\tau_2, \tau_1)\mathcal{R} \quad (18.6)$$

The imaginary period monodromy matrix is

$$\mathcal{M}_i = \mathcal{P}(4K', 0) \quad (18.7)$$

Define

$$\mathcal{M}_{i/4} = \mathcal{P}(K', 0) \quad \mathcal{M}_{i/2} = \mathcal{P}(2K', 0) \quad (18.8)$$

Then

$$\begin{aligned} \mathcal{M}_{i/2} &= \mathcal{P}(2K', K')\mathcal{P}(K', 0) = \mathcal{R}\mathcal{P}(0, K')\mathcal{R}\mathcal{P}(K', 0) \\ &= \mathcal{R}\mathcal{M}_{i/4}^{-1}\mathcal{R}\mathcal{M}_{i/4} = \mathcal{R}\Omega\mathcal{M}_{i/4}^t\Omega\mathcal{R}\mathcal{M}_{i/4} \\ \mathcal{M}_i &= \mathcal{P}(4K', 2K')\mathcal{P}(2K', 0) = \overline{\mathcal{P}(0, 2K')}\mathcal{P}(2K', 0) \\ &= \overline{\mathcal{M}_{i/2}}^{-1}\mathcal{M}_{i/2} = \Omega\mathcal{M}_{i/2}^\dagger\Omega\mathcal{M}_{i/2} \end{aligned} \quad (18.9)$$

so to calculate  $\mathcal{M}_i$  it is enough to calculate  $\mathcal{M}_{i/4}$ . It is enough to integrate the ode from  $K$  to  $K + K'i$ .

## 18.2 $\mathcal{V}_{\text{phys}}(t)$

For an ode with  $N_{\text{gauge}} > 0$ , the gauge solution is  $\mathcal{W}_{\text{gauge}}(z)$ . The physical phase-space  $\mathcal{V}_{\text{phys}}(t)$  is the quotient  $\mathcal{W}_{\text{gauge}}^\perp / \mathbb{C}\mathcal{W}_{\text{gauge}}$  where  $\mathcal{W}_{\text{gauge}}^\perp \mathbb{C}^N$  is the  $\Omega$ -complement of  $\mathcal{W}_{\text{gauge}}(z)$ . For the numerical computations it is useful to represent  $\mathcal{V}_{\text{phys}}(t)$  as a subspace of  $\mathcal{W}_{\text{gauge}}^\perp$ . Write

$$\mathcal{V} = \mathcal{V} \quad \mathcal{V}_{\text{phys}} = \mathcal{V}_{\text{phys}}(t) \quad \mathcal{W}_{\text{gauge}} = \mathcal{W}_{\text{gauge}}(t) \quad (18.10)$$

Define the vector

$$\tilde{\mathcal{W}}_{\text{gauge}} = i\Omega\mathcal{W}_{\text{gauge}} \quad (18.11)$$

satisfying

$$\begin{aligned} \mathcal{W}_{\text{gauge}}^t \tilde{\mathcal{W}}_{\text{gauge}} &= 0 & \mathcal{W}_{\text{gauge}}^t \mathcal{W}_{\text{gauge}} &= \tilde{\mathcal{W}}_{\text{gauge}}^t \tilde{\mathcal{W}}_{\text{gauge}} \\ \mathcal{W}_{\text{gauge}}^t \Omega \tilde{\mathcal{W}}_{\text{gauge}} &= i\mathcal{W}_{\text{gauge}}^t \mathcal{W}_{\text{gauge}} \end{aligned} \quad (18.12)$$

$\mathcal{W}_{\text{gauge}}$  is real so  $\tilde{\mathcal{W}}_{\text{gauge}}$  is also real. The orthogonal complement  $\tilde{\mathcal{W}}_{\text{gauge}}^\perp$  is the  $\Omega$ -orthogonal complement of  $\mathcal{W}_{\text{gauge}}$ .

$$\tilde{\mathcal{W}}_{\text{gauge}}^t \mathcal{W} = 0 \quad \Leftrightarrow \quad \mathcal{W}_{\text{gauge}}^t \Omega \mathcal{W} = 0 \quad (18.13)$$

$\tilde{\mathcal{W}}$  is not a natural vector since  $\Omega$  is a bilinear form on  $\mathcal{V}$ , not a linear operator.  $\tilde{\mathcal{W}}$  depends on a choice of bilinear form on  $\mathcal{V}$ . Choosing  $\tilde{\mathcal{W}}_{\text{gauge}}$  give the decomposition

$$\mathcal{V} = \mathbb{C}\tilde{\mathcal{W}}_{\text{gauge}} \oplus \mathbb{C}\mathcal{W}_{\text{gauge}} \oplus \mathcal{V}_{\text{phys}} \quad (18.14)$$

representing  $\mathcal{V}_{\text{phys}}$  as a codimension two subspace of  $\mathcal{V}$ . Define

$$P = \mathcal{W}_{\text{gauge}}(\mathcal{W}_{\text{gauge}}^t \mathcal{W}_{\text{gauge}})^{-1} \mathcal{W}_{\text{gauge}}^t \quad \tilde{P} = \tilde{\mathcal{W}}_{\text{gauge}}(\tilde{\mathcal{W}}_{\text{gauge}}^t \tilde{\mathcal{W}}_{\text{gauge}})^{-1} \tilde{\mathcal{W}}_{\text{gauge}}^t \quad (18.15)$$

which are commuting projections

$$P^2 = P \quad \tilde{P}^2 = \tilde{P} \quad P\tilde{P} = \tilde{P}P = 0 \quad P^t = P \quad \tilde{P}^t = \tilde{P} \quad (18.16)$$

Then define

$$P_{\text{gauge}} = 1 - \tilde{P} \quad P_{\text{phys}} = P_{\text{gauge}} - P = 1 - \tilde{P} - P \quad (18.17)$$

so

$$\begin{aligned} P_{\text{gauge}} \mathcal{V} &= (W_{\text{gauge}})^\perp & \mathcal{V} &= \mathbb{C}\tilde{\mathcal{W}}_{\text{gauge}} \oplus (W_{\text{gauge}})^\perp \\ P_{\text{phys}} \mathcal{V} &= \mathcal{V}_{\text{phys}} & (W_{\text{gauge}})^\perp &= \mathbb{C}\mathcal{W}_{\text{gauge}} \oplus \mathcal{V}_{\text{phys}} \end{aligned} \quad (18.18)$$

$$\begin{aligned} \mathcal{V} &= \mathbb{C}\tilde{\mathcal{W}}_{\text{gauge}} \oplus \mathbb{C}\mathcal{W}_{\text{gauge}} \oplus \mathcal{V}_{\text{phys}} \\ i\Omega\mathcal{P}(i\Omega)^t &= \tilde{\mathcal{W}}_{\text{gauge}}(\mathcal{W}_{\text{gauge}}^t \mathcal{W}_{\text{gauge}})^{-1} \tilde{\mathcal{W}}_{\text{gauge}}^t = \tilde{\mathcal{P}} \\ \Omega\mathcal{P}\Omega &= \tilde{\mathcal{P}} \quad \Omega\mathcal{P} = \tilde{\mathcal{P}}\Omega \quad \Omega = \tilde{\mathcal{P}}\Omega\mathcal{P} + \mathcal{P}\Omega\tilde{\mathcal{P}} \end{aligned} \quad (18.19)$$

## References

- [1] G. Racah, “Theory of Complex Spectra. II,” *Phys. Rev.* **62** (Nov, 1942) 438–462.
- [2] “NIST Digital Library of Mathematical Functions.” Release 1.1.4 of 2022-01-15, <http://dlmf.nist.gov/>. F. W. J. Olver, A. B. Olde Daalhuis, D. W. Lozier, B. I. Schneider, R. F. Boisvert, C. W. Clark, B. R. Miller, B. V. Saunders, H. S. Cohl, and M. A. McClain, eds.
