# Supplementary material for: Thermodynamic stability of a cosmological SU(2)-weak gauge field
Source: arXiv:2203.12052 ancillary file (2022-03-24)
Supplement: Supplementary file 2 [file K_z__matrices.pdf]

# Calculate $K(z)$ matrices

$$K(z) = K_2 b(z)^2 + K_1 b(z) + K_0$$

## Definitions and declarations

```
In [1]: %display latex
maxima_calculus('algebraic: true;')
def LE(str):
    return(LatexExpr(r'+' + str))
```

## Racah W-coefficient

calculate W(j1,j2,J,j3,J12,J23,jtestmin='False'))

```
    if j3 is a rational number
        use the builtin racah() function
    else
        use the algebraic algorithm
        return an algebraic expression
        test the algebraic expression:
            if jtestmin is a rational number
                substitute in the algebraic expression for W
                jR = jtestmin, jtestmin+1/2, ... 11/2
                and compare to racah()
```

```
In [2]: def W(j1,j2,J,j3,J12,J23,jtestmin='False'):
    if j3 in QQ:
        return(Wnum(j1,j2,J,j3,J12,J23))
    Walgval=Walg(j1,j2,J,j3,J12,J23)
    if jtestmin not in QQ:
        return(Walgval)
    for nn in range(2*jtestmin,12):
        jRval = nn/2
        Wnumval = Wnum(j1,j2,J.subs(jR=jRval),j3.subs(jR=jRval),J12,J23.subs(jR=jRval))
        Walgnumval=Walgval.subs(jR=jRval)
        if Walgnumval not in QQ:
            Walgnumval=Walgnumval.canonicalize_radical()
        if Walgnumval != Wnumval:
            print('RACAH DISCREPANCY', 'jR=',jRval, 'Wnum=',Wnumval, 'Walgnum=',\
                Walgnumval, 'Walg=',Walgval)
    return(Walgval)
```

```
In [3]: def Wnum(j1,j2,J,j3,J12,J23):
    Wnumval = racah(j1,j2,J,j3,J12,J23)
    if Wnumval not in QQ:
        Wnumval=Wnumval.canonicalize_radical()
    return(Wnumval)
```

```
In [4]: def Δsq(a,b,c):
    val = factorial(a+b-c)*factorial(a-b+c)*factorial(-a+b+c)/factorial(a+b+c+1)
    return val
def Walg(j1,j2,J,j3,J12,J23):
    # jR=var('jR', latex_name="j_{R}")
    assume(jR > 2)
    a=j1
    b=j2
    c=J
    d=j3
    e=J12
    f=J23
    α1 = a+b+e
    α2 = c+d+e
```

```

 $\alpha_3$  = a+c+f
 $\alpha_4$  = b+d+f
 $\beta_1$  = a+b+c+d
 $\beta_2$  = a+d+e+f
 $\beta_3$  = b+c+e+f
max $\alpha$  = max([ $\alpha_1$ , $\alpha_2$ , $\alpha_3$ , $\alpha_4$ ])
min $\beta$  = min([ $\beta_1$ , $\beta_2$ , $\beta_3$ ])
w=0
zrange=min $\beta$  - max $\alpha$  + 1
for zm in range(0,zrange):
    z=zm+max $\alpha$ 
    s = (-1)^(zm)*factorial(z+1)
    s = s/(factorial(z- $\alpha_1$ )*factorial(z- $\alpha_2$ )*factorial(z- $\alpha_3$ )*factorial(z- $\alpha_4$ ))
    s = s/(factorial( $\beta_1$ -z)*factorial( $\beta_2$ -z)*factorial( $\beta_3$ -z))
    w+=s
d =  $\Delta$ sq(a,b,e)* $\Delta$ sq(c,d,e)* $\Delta$ sq(a,c,f)* $\Delta$ sq(b,d,f)
d = d.full_simplify()
Wval = w* sqrt(d)
Wval = (((-1)^( $\beta_1$ +max $\alpha$ )*Wval).full_simplify()).subs((-1)^(4*jR)==1)
Wval = Wval.canonicalize_radical()
return(Wval)

```

```

In [5]: def recoupling(j1,j2,J,j3,J12,J23,jtestmin='FALSE'):
        Wval= W(j1,j2,J,j3,J12,J23,jtestmin)
        recouplingval= sqrt((2*J12+1)*(2*J23+1))*Wval
        # recouplingval= recouplingval.canonicalize_radical()
        return(recouplingval)

```

## Construct the matrices K\_2, K\_1, K\_0

N, J12list, J23list, jL, jtestmin global variables

```

In [6]: def constr_K_matrices():
        U = Matrix(SR,N,N)
        for ii in range(N):
            J12 = J12list[ii]
            for jj in range(N):
                J23 = J23list[jj]
                U[ii,jj] = recoupling(1,1,jR,jL,J12,J23,jtestmin)
        C12 = diagonal_matrix(SR, N, map(lambda x: x*(x+1)/2,J12list))
        C23diag = diagonal_matrix(SR, N, map(lambda x: x*(x+1)/2,J23list))
        C23 = U * C23diag * U.transpose()
        Gam = C12-2
        stard = 2*(C23- jR*(jR+1)/2)
        stardpG = stard+Gam
        K_2 = Gam^2-Gam
        K_1 = (stardpG*Gam+Gam*stardpG).canonicalize_radical()
        K_0 = (stardpG^2+Gam).canonicalize_radical()
        K_1 = K_1.subs(jR=jRsub).canonicalize_radical()
        K_0 = K_0.subs(jR=jRsub).canonicalize_radical()
        return(K_2,K_1,K_0)

```

```

In [7]: epsb=var('epsb',latex_name="\\epsilon")
        alpha=var('alpha',latex_name="\\alpha")
        sigma=var('sigma',latex_name="\\sigma")
        j = var('j')
        odes={}

```

## ode 2

```

In [8]: N=2
        J12list = [0,1]
        J23list = [1/2,3/2]
        jR=1/2
        jL = 1/2
        jtestmin=1/2
        jRsub=j
        (K_2,K_1,K_0) = constr_K_matrices()
        pretty_print(LE('K_2 = '),K_2,LE('\\qquad K_1 = '),K_1,LE('\\epsilon_{b}'),\\
                    LE('\\qquad K_0 = '),K_0,LE('\\epsilon_{b}^{2}'))
        #
        print("\\n")
        alphaexp = 0

```

```

sigmaexp = epsb/sqrt(2)
K2mat = K_2
K1mat = K_1*sqrt(2)
K0mat = K_0*2
w1mat = Matrix([[0],[1]])
w0mat = Matrix([[1],[0]])
w0coeff = sigma/sqrt(2)
F= var('F')
Kmat= (K2mat*F^2+K1mat*sigma*F+K0mat*sigma^2).subs(alpha=alphaexp,sigma=sigmaexp)
wvec = (w1mat*F + w0mat*sigma).subs(alpha=alphaexp,sigma=sigmaexp)
#wvec = w1mat*F + w0mat*w0coeff
diff = w1mat *(2*epsb^2*F-2*F^3)+ Kmat*wvec
#diff = diff.canonicalize_radical()
#diff = diff.simplify_full()
#pretty_print(diff)
wconf = (diff == 0)
pretty_print(alpha,LE(' = '),alphaexp,LE('\qquad'),sigma,LE(' = '),sigmaexp)
print("\n")
pretty_print(LE('K_2 = '),K2mat,LE('\qquad K_1 = '),K1mat,\
sigma,LE('\qquad K_0 = '),K0mat,sigma^2)
print("\n")
#
#
print("\n")
pretty_print(LE('w_1 = '),w1mat,LE('\qquad w_0 = '),w0mat,sigma,LE('\qquad'),wconf)
#
ode={}
ode['K2mat']=K2mat
ode['K1mat']=K1mat
ode['K0mat']=K0mat
ode['alphaexp']=alphaexp
ode['sigmaexp']=sigmaexp
ode['w1mat']=w1mat
ode['w0mat']=w0mat
ode['gauged']=True
odes['2'] = ode

```

$$K_2 = \begin{pmatrix} 6 & 0 \\ 0 & 2 \end{pmatrix} \quad K_1 = \begin{pmatrix} 0 & -3\sqrt{2} \\ -3\sqrt{2} & 0 \end{pmatrix} \epsilon_b \quad K_0 = \begin{pmatrix} 0 & 0 \\ 0 & 1 \end{pmatrix} \epsilon_b^2$$

$$\alpha = 0 \quad \sigma = \frac{1}{2} \sqrt{2} \epsilon$$

$$K_2 = \begin{pmatrix} 6 & 0 \\ 0 & 2 \end{pmatrix} \quad K_1 = \begin{pmatrix} 0 & -6 \\ -6 & 0 \end{pmatrix} \sigma \quad K_0 = \begin{pmatrix} 0 & 0 \\ 0 & 2 \end{pmatrix} \sigma^2$$

$$w_1 = \begin{pmatrix} 0 \\ 1 \end{pmatrix} \quad w_0 = \begin{pmatrix} 1 \\ 0 \end{pmatrix} \sigma \quad \text{True}$$

## ode 3<sub>j</sub>

In [9]:

```

jR=var('jR',latex_name="j_{R}")
N=3
J12list = [0,1,2]
J23list = [jR-1,jR,jR+1]
jL = jR
jtestmin=1
jRsub = j-1/2
(K_2,K_1,K_0) = constr_K_matrices()
pretty_print(LE('K_2 = '),K_2)
print("\n")
pretty_print(LE('K_1 = '),K_1,LE('\epsilon_{b}'))
print("\n")
pretty_print(LE('K_0 = '),K_0,LE('\epsilon_{b}^2'))
print("\n\n")
#
alphaexp = sqrt(2)* sqrt((j^2-1)/(j^2-1/4))

```

```

sigmaexp = sqrt(2/3)*sqrt(j^2-1/4)*epsb
#
K2mat = K_2
K1mat = -6*Matrix([[0,1,0],[1,0,0],[0,0,0]])
K0mat = 2*Matrix([[alpha^2,0,alpha],[0,alpha^2+1,0],[alpha,0,1]])
#
K1test = (sigma*K1mat).subs(alpha=alphaexp,sigma=sigmaexp)
K1test = K1test.canonicalize_radical()
K1eps = (K_1*epsb).canonicalize_radical()
conf1 = (K_1*epsb == K1test)
K0test = (sigma^2*K0mat).subs(alpha=alphaexp,sigma=sigmaexp)
K0test = K0test.canonicalize_radical()
K0eps = (K_0*epsb^2).canonicalize_radical()
conf0 = (K0eps == K0test)
F= var('F')
K = K_2 *F^2 + K_1*epsb*F +K_0*epsb^2
Kmat = (K2mat*F^2+K1mat*sigma*F+K0mat*sigma^2).subs(alpha=alphaexp,sigma=sigmaexp)
diff = (K-Kmat).canonicalize_radical()
conf = (diff == 0)
#
pretty_print(alpha,LE(' = '),alphaexp,LE('\qquad'),sigma,LE(' = '),sigmaexp)
print("\n")
pretty_print(LE('K_2 = '),K2mat,LE('\qquad K_1 = '),K1mat,sigma,LE('\qquad K_0 = '),\
K0mat,sigma^2,LE('\qquad'),conf0 and conf1 and conf)
print("\n")
#
w1mat = Matrix([[0],[1],[0]])
w0mat = Matrix([[1],[0],[-alpha]])
wvec = (w1mat*F + w0mat*sigma).subs(alpha=alphaexp,sigma=sigmaexp)
diff = w1mat *(2*epsb^2*F-2*F^3)+ K*wvec
diff = diff.canonicalize_radical()
#diff = diff.simplify_full()
#pretty_print(diff)
wconf = (diff == 0)
pretty_print(LE('w_1 = '),w1mat,LE('\qquad w_0 = '),w0mat,sigma,LE('\qquad'),wconf)
#
#
ode={}
ode['K2mat']=K2mat
ode['K1mat']=K1mat
ode['K0mat']=K0mat
ode['alphaexp']=alphaexp
ode['sigmaexp']=sigmaexp
ode['w1mat']=w1mat
ode['w0mat']=w0mat
ode['gauged']=True
odes['3j'] = ode

```

$$K_2 = \begin{pmatrix} 6 & 0 & 0 \\ 0 & 2 & 0 \\ 0 & 0 & 0 \end{pmatrix}$$

$$K_1 = \begin{pmatrix} 0 & -\sqrt{3}\sqrt{2}\sqrt{2j+1}\sqrt{2j-1} & 0 \\ -\sqrt{3}\sqrt{2}\sqrt{2j+1}\sqrt{2j-1} & 0 & 0 \\ 0 & 0 & 0 \end{pmatrix} \epsilon_b$$

$$K_0 = \begin{pmatrix} \frac{8}{3}j^2 - \frac{8}{3} & 0 & \frac{2}{3}\sqrt{2}\sqrt{2j+1}\sqrt{2j-1}\sqrt{j+1}\sqrt{j-1} \\ 0 & 4j^2 - 3 & 0 \\ \frac{2}{3}\sqrt{2}\sqrt{2j+1}\sqrt{2j-1}\sqrt{j+1}\sqrt{j-1} & 0 & \frac{4}{3}j^2 - \frac{1}{3} \end{pmatrix} \epsilon_b^2$$

$$\alpha = 2\sqrt{2}\sqrt{\frac{j^2-1}{4j^2-1}} \quad \sigma = \frac{1}{2}\sqrt{\frac{2}{3}}\sqrt{4j^2-1}\epsilon$$

$$K_2 = \begin{pmatrix} 6 & 0 & 0 \\ 0 & 2 & 0 \\ 0 & 0 & 0 \end{pmatrix} \quad K_1 = \begin{pmatrix} 0 & -6 & 0 \\ -6 & 0 & 0 \\ 0 & 0 & 0 \end{pmatrix} \sigma \quad K_0 = \begin{pmatrix} 2\alpha^2 & 0 & 2\alpha \\ 0 & 2\alpha^2 + 2 & 0 \\ 2\alpha & 0 & 2 \end{pmatrix} \sigma^2 \quad \text{True}$$

$$w_1 = \begin{pmatrix} 0 \\ 1 \\ 0 \end{pmatrix} \quad w_0 = \begin{pmatrix} 1 \\ 0 \\ -\alpha \end{pmatrix} \sigma \quad \text{True}$$

## ode 2<sub>j</sub>

In [10]:

```
jR=var('jR', latex_name="j_{R}")
j = var('j')
N=2
J12list = [1,2]
J23list = [jR,jR+1]
jL = jR+1
jtestmin=1/2
jRsub=j-1
(K_2,K_1,K_0) = constr_K_matrices()
pretty_print(LE('K_2 = '),K_2,LE('\qquad K_1 = '),K_1,LE('\epsilon_{b}'),\
LE('\qquad K_0 = '),K_0,LE('\epsilon_{b}^2'))
print("\n\n")
#
alphaexp = sqrt(1-1/j^2)
sigmaexp = j*epsb
K2mat=K_2
K1mat = 2*Matrix([[ -1,0],[0,1]])
K0mat = 2*Matrix([[alpha^2,alpha],[alpha,1]])
#
Kltest = (sigma*K1mat).subs(alpha=alphaexp,sigma=sigmaexp)
Kltest = Kltest.canonicalize_radical()
K1eps = (K_1*epsb).canonicalize_radical()
conf1 = (K_1*epsb == Kltest)
K0test = (sigma^2*K0mat).subs(alpha=alphaexp,sigma=sigmaexp)
K0test = K0test.canonicalize_radical()
K0eps = (K_0*epsb^2).canonicalize_radical()
conf0 = (K0eps == K0test)
#
K = K_2 *F^2 + K_1*epsb*F +K_0*epsb^2
Kmat = (K2mat*F^2+K1mat*sigma*F+K0mat*sigma^2).subs(alpha=alphaexp,sigma=sigmaexp)
diff = (K-Kmat).canonicalize_radical()
conf = (diff == 0)
#
pretty_print(alpha,LE(' = '),alphaexp,LE('\qquad'),sigma,LE(' = '),sigmaexp)
print("\n")
pretty_print(LE('K_2 = '),K2mat,LE('\qquad K_1 = '),K1mat,sigma,LE('\qquad K_0 = '),\
K0mat,sigma^2,LE('\qquad'),conf1 and conf0 and conf)
print("\n")
#
#
w1mat = Matrix([[1],[0]])
w0mat = Matrix([[1],[-alpha]])
Kmat= K_2*F^2+K_1*epsb*F+K_0*epsb^2
wvec = (w1mat*F + w0mat*sigma).subs(alpha=alphaexp,sigma=sigmaexp)
diff = w1mat *(2*epsb^2*F-2*F^3)+ Kmat*wvec
diff = diff.canonicalize_radical()
#diff = diff.simplify_full()
#pretty_print(diff)
wconf = (diff == 0)
pretty_print(LE('w_1 = '),w1mat,LE('\qquad w_0 = '),w0mat,sigma,LE('\qquad'),wconf)
#
ode={}
ode['K2mat']=K2mat
ode['K1mat']=K1mat
ode['K0mat']=K0mat
ode['alphaexp']=alphaexp
ode['sigmaexp']=sigmaexp
ode['w1mat']=w1mat
ode['w0mat']=w0mat
ode['gauged']=True
odes['2j'] = ode
```

$$K_2 = \begin{pmatrix} 2 & 0 \\ 0 & 0 \end{pmatrix} \quad K_1 = \begin{pmatrix} -2j & 0 \\ 0 & 2j \end{pmatrix} \epsilon_b \quad K_0 = \begin{pmatrix} 2j^2 - 2 & 2\sqrt{j+1}\sqrt{j-1}j \\ 2\sqrt{j+1}\sqrt{j-1}j & 2j^2 \end{pmatrix} \epsilon_b^2$$

$$\alpha = \sqrt{-\frac{1}{j^2} + 1} \quad \sigma = \epsilon j$$

$$K_2 = \begin{pmatrix} 2 & 0 \\ 0 & 0 \end{pmatrix} \quad K_1 = \begin{pmatrix} -2 & 0 \\ 0 & 2 \end{pmatrix} \sigma \quad K_0 = \begin{pmatrix} 2\alpha^2 & 2\alpha \\ 2\alpha & 2 \end{pmatrix} \sigma^2 \quad \text{True}$$

$$w_1 = \begin{pmatrix} 1 \\ 0 \end{pmatrix} \quad w_0 = \begin{pmatrix} 1 \\ -\alpha \end{pmatrix} \sigma \quad \text{True}$$

## ode 1<sub>j</sub>

In [11]:

```
jR=var('jR', latex_name="j_{R}")
j = var('j')
N=1
J12list = [2]
J23list = [jR+1]
jL=jR+2
jtestmin=1/2
jRsub=j-3/2
(K_2,K_1,K_0) = constr_K_matrices()
pretty_print(LE('K_2 ='),K_2,LE('\qquad K_1 ='),K_1,LE('\epsilon_{b}'),\
               LE('\qquad K_0 ='),K_0,LE('\epsilon_{b}^2'))
print("\n")
#
sigmaexp = j*epsb
alphaexp = sqrt(1+1/(4*j^2))
K2mat = K_2
K1mat = 4 *Matrix([1])
K0mat = 4*Matrix([alpha^2])
#
Kltest = (sigma*K1mat).subs(sigma=sigmaexp,alpha=alphaexp)
Kltest = Kltest.canonicalize_radical()
K1eps = (K_1*epsb).canonicalize_radical()
conf1 = (K_1*epsb == Kltest)
K0test = (sigma^2*K0mat).subs(sigma=sigmaexp,alpha=alphaexp)
K0test = K0test.canonicalize_radical()
K0eps = (K_0*epsb^2).canonicalize_radical()
conf0 = (K0eps == K0test)
#
K = K_2 *F^2 + K_1*epsb*F +K_0*epsb^2
Kmat = (K2mat*F^2+K1mat*sigma*F+K0mat*sigma^2).subs(alpha=alphaexp,sigma=sigmaexp)
diff = (K-Kmat).canonicalize_radical()
conf = (diff == 0)
#
pretty_print(alpha,LE(' = '),alphaexp,LE('\qquad'),sigma,LE(' = '),sigmaexp)
print("\n")
pretty_print(LE('K_2 ='),K2mat,LE('\quad K_1 = '),K1mat,sigma,LE('\qquad K_0 = '),\
              K0mat,sigma^2,LE('\qquad'),conf0 and conf1 and conf)
#
ode={}
ode['K2mat']=K2mat
ode['K1mat']=K1mat
ode['K0mat']=K0mat
ode['alphaexp']=alphaexp
ode['sigmaexp']=sigmaexp
ode['gauged']=False
odes['1j'] = ode
```

$$K_2 = (0) \quad K_1 = (4j) \epsilon_b \quad K_0 = (4j^2 + 1) \epsilon_b^2$$

$$\alpha = \frac{1}{2} \sqrt{\frac{1}{j^2} + 4} \quad \sigma = \epsilon j$$

$$K_2 = (0) \quad K_1 = (4) \sigma \quad K_0 = (4 \alpha^2) \sigma^2 \quad \text{True}$$

```
In [12]: save(odes,'odes') # load with odes=load('odes')
```

```
In [13]: odes =load('odes')
```

```
In [25]: for ode_key in ['2','3j','2j','1j']:
          print('\n')
          pretty_print(LE(r"\mathbf{ODE}\;";"),ode_key)
          for (key,value) in odes[ode_key].items():
              pretty_print(key,' = ',value)
```

### ODE 2

$$\mathbf{K2mat} = \begin{pmatrix} 6 & 0 \\ 0 & 2 \end{pmatrix}$$

$$\mathbf{K1mat} = \begin{pmatrix} 0 & -6 \\ -6 & 0 \end{pmatrix}$$

$$\mathbf{K0mat} = \begin{pmatrix} 0 & 0 \\ 0 & 2 \end{pmatrix}$$

$$\text{alphaexp} = 0$$

$$\text{sigmaexp} = \frac{1}{2} \sqrt{2} \epsilon$$

$$\mathbf{w1mat} = \begin{pmatrix} 0 \\ 1 \end{pmatrix}$$

$$\mathbf{w0mat} = \begin{pmatrix} 1 \\ 0 \end{pmatrix}$$

$$\text{gauged} = \text{True}$$

### ODE 3j

$$\mathbf{K2mat} = \begin{pmatrix} 6 & 0 & 0 \\ 0 & 2 & 0 \\ 0 & 0 & 0 \end{pmatrix}$$

$$\mathbf{K1mat} = \begin{pmatrix} 0 & -6 & 0 \\ -6 & 0 & 0 \\ 0 & 0 & 0 \end{pmatrix}$$

$$\mathbf{K0mat} = \begin{pmatrix} 2 \alpha^2 & 0 & 2 \alpha \\ 0 & 2 \alpha^2 + 2 & 0 \\ 2 \alpha & 0 & 2 \end{pmatrix}$$

$$\text{alphaexp} = 2 \sqrt{2} \sqrt{\frac{j^2 - 1}{4 j^2 - 1}}$$

$$\text{sigmaexp} = \frac{1}{2} \sqrt{\frac{2}{3}} \sqrt{4 j^2 - 1} \epsilon$$

$$\text{w1mat} = \begin{pmatrix} 0 \\ 1 \\ 0 \end{pmatrix}$$

$$\text{w0mat} = \begin{pmatrix} 1 \\ 0 \\ -\alpha \end{pmatrix}$$

$$\text{gauged} = \text{True}$$

$$\text{ODE } 2j$$

$$\text{K2mat} = \begin{pmatrix} 2 & 0 \\ 0 & 0 \end{pmatrix}$$

$$\text{K1mat} = \begin{pmatrix} -2 & 0 \\ 0 & 2 \end{pmatrix}$$

$$\text{K0mat} = \begin{pmatrix} 2 \alpha^2 & 2 \alpha \\ 2 \alpha & 2 \end{pmatrix}$$

$$\text{alphaexp} = \sqrt{-\frac{1}{j^2} + 1}$$

$$\text{sigmaexp} = \epsilon j$$

$$\text{w1mat} = \begin{pmatrix} 1 \\ 0 \end{pmatrix}$$

$$\text{w0mat} = \begin{pmatrix} 1 \\ -\alpha \end{pmatrix}$$

$$\text{gauged} = \text{True}$$

$$\text{ODE } 1j$$

$$\text{K2mat} = (0)$$

$$\text{K1mat} = (4)$$

$$\text{K0mat} = (4 \alpha^2)$$

$$\text{alphaexp} = \frac{1}{2} \sqrt{\frac{1}{j^2} + 4}$$

$$\text{sigmaexp} = \epsilon j$$



gauged =False

In [26]: `#pretty_print(odes['2'])`

In [27]: `#pretty_print(odes['3j'])`

In [28]: `#pretty_print(odes['2j'])`

In [29]: `#pretty_print(odes['1j'])`

In [ ]:
