# Supplementary material for: Thermodynamic stability of a cosmological SU(2)-weak gauge field
Source: arXiv:2203.12052 ancillary file (2022-03-24)

# Integrate the odes to check property P

## Imports

```
In [1]: from mpmath import mp
        from mpmath import mpf, mpc
        import sage.libs.mpmath.all as a
        mp.pretty = True
        from timeit import default_timer as timer
        # start=timer()
        # end=timer()
```

## Functions to analyze the odes over a range of parameters

Each ode is parametrized by two numbers,  $\sigma$  and  $\alpha$  which are functions of

- $j$  and  $\epsilon$  for odes  $3_j$ ,  $2_j$ , and  $1_j$
- $\epsilon$  for ode 2.

function to analyze ode  $3_j$ ,  $2_j$ , or  $1_j$  at  $j = \infty$  for list of  $\sigma$  values

The limit  $j \rightarrow \infty$  is taken with  $\sigma$  fixed.

```
In [2]: def process_sigma_list():
        global jval, epsilonb, sigma_val, alpha_val
        global data_asymp
        set_precision()
        initialize_ode()
        for sigma_arg in sigma_list:
            epsilonb=0.0
            set_Jacobi_parameters()
            sigma_val=myR(sigma_arg)
            jval=Infinity
            alpha_val = myR(limit(alpha_exp, j=jval))
            #
            analyze_monodromy()
            if GOOD:
                data[ode_name]['asymp'][sigma_val]=data_dict
```

function to analyze ode  $3_j$ ,  $2_j$ , or  $1_j$  for list of  $j$  values given  $\epsilon$

```
In [3]: def process_j_list():
        global jval, sigma_val, alpha_val
        global data_j
        set_precision()
        initialize_ode()
        set_Jacobi_parameters()
        eps_string = epsilonb.str(digits=4, skip_zeroes=True)
        for j_arg in j_list:
            jval = j_arg
            alpha_val = myR(alpha_exp.subs(j=jval))
            sigma_val = myR(sigma_exp.subs(j=jval, epsb=myR(epsilonb)))
            #
            analyze_monodromy()
            if GOOD:
                if eps_string not in data[ode_name]['finite']:
                    data[ode_name]['finite'][eps_string]={}
                    data[ode_name]['finite'][eps_string][jval]=data_dict
```

Function to analyze ode 2 for list of  $\epsilon$  values

```
In [4]: def process_ode2_epsilonb_list():
        global jval, epsilonb, sigma_val, alpha_val, ode_decimal_precision
        global data_small_j
        set_precision()
        initialize_ode()
        jval=None
```

```

for epsilonb_arg in epsilonb_list:
    epsilonb=epsilonb_arg
    eps_string = epsilonb.str(digits=4,skip_zeroes=True)
    set_Jacobi_parameters()
    alphaval = myR(alphaexp)
    sigmaaval = myR(sigmaexp.subs(epsb=myR(epsilonb)))
    #
    analyze_monodromy()
    if GOOD:
        data[ode_name][eps_string]=data_dict

```

## Function to analyze imaginary period monodromy matrix

```

In [5]: def analyze_monodromy():
    global data_dict,GOOD
    start = timer()
    GOOD=True
    if gauged:
        construct_gauge()
    mp.dps=ode_decimal_precision
    create_ode()
    start_ode=timer()
    calculate_Mi()
    end_ode=timer();
    ode_time = end_ode-start_ode
    mp.dps=high_decimal_precision
    check_Mi()
    if gauged:
        check_gauge_invariance()
        construct_Vphys()
    construct_Mi_phys()
    check_property_P()
    if property_P:
        calculate_frequencies()
        end=timer()
        total_time = end-start
        eps_string = epsilonb.str(digits=4,skip_zeroes=True)
        pretty_print(LE('\epsilon ='), eps_string,LE('\quad j ='), jval,\
                     LE('\quad\sigma ='), n(sigmaaval,digits=3), LE('\quad\omega/\sigma^2='), mpstr(f\
                     ' (', ode_decimal_precision,', ', decimal_tol, ')', \
                     ' ode time = ', n(ode_time,digits=5), ' other time = ', n(total_time-ode_
    if GOOD:
        data_dict = dictify_vars('jval','sigmaaval','epsilonb','fs_ratio','Mi','Mi_phys','H','Vmat',\
                                'ode_decimal_precision','high_decimal_precision',\
                                'N','gauged','H_eigenvalues','min_H_eigenvalue','positive_frequencies','negative_
                                'MiR','Mi_eigenvalues')

```

## subroutines

```

In [6]: def calculate_Mi():
    global Mi4,Mi2,Mi
    Mi4 = cP(Jac_Kp)
    Mi2 = cR*Omega*Mi4.transpose()*Omega*cR*Mi4
    Mi = Omega*Mi2.transpose_conj()*Omega*Mi2

```

```

In [7]: def check_Mi():
    global GOOD
    if not aeq(mp.det(Mi),1):
        GOOD=False
        print ('FAIL: Mi does not have det 1')
    if not aeq(Mi.transpose()*Omega*Mi,Omega):
        GOOD=False
        print ('FAIL: Mi is not symplectic')

```

```

In [8]: def check_gauge_invariance():
    global GOOD
    if not aeq(Wgauge,Mi*Wgauge):
        GOOD = False
        print('Mi FAILS gauge invariance check')

```

```

In [9]: def construct_Vphys():
    global Vmat,GOOD

```

```

Proj_rem = Proj_phys
Nphys = N-1
vlist=[]
vplist=[]
for ii in range(Nphys):
    v = mp.matrix(int(Crank),int(1))
    v[ii]=1
    vphys = Proj_rem*v
    vphys = (1/mp.norm(vphys))*vphys
    vpphys = mp.j*Omega*vphys
    vlist.append(vphys)
    vplist.append(vpphys)
    Proj_rem = Proj_rem - vphys*vphys.transpose()- vpphys*vpphys.transpose()
Vmat = mp.matrix(int(Crank),int(0))
for ii in range(Nphys):
    Vmat=mp.extend(Vmat,vlist[ii])
for ii in range(Nphys):
    Vmat=mp.extend(Vmat,vplist[ii])
if not aeq(Vmat.transpose()*Vmat,mp.eye(int(2*Nphys))):
    GOOD=False
    print('FAIL Vmat^t Vmat not = 1')

```

In [10]:

```

def construct_Mi_phys():
    global Mi_phys, Omega_phys,GOOD
    if gauged:
        Mi_phys = Vmat.transpose()*Mi*Vmat
        Omega_phys = Vmat.transpose()*Omega*Vmat
        if not aeq(mp.det(Mi_phys),1):
            GOOD=False
            print('FAIL Mi_phys not det 1')
        if not aeq(Mi_phys.transpose()*Omega_phys*Mi_phys,Omega_phys):
            GOOD=False
            print('FAIL Mi_phys not symplectic')
    else:
        Mi_phys = Mi
        Omega_phys = Omega

```

In [11]:

```

def check_property_P():
    global H,H_eigenvalues,property_P,min_H_eigenvalue,HR,GOOD
    H=Omega_phys*Mi_phys-Omega_phys
    H_eigenvalues_complex,HR = mp.eig(H)
    property_P = False
    if not aeq(H,H.transpose_conj()):
        GOOD=False
        print('H FAILS to be hermitian')
        return
    H_eigenvalues=[]
    for x in H_eigenvalues_complex:
        if a0(mp.im(x)):
            H_eigenvalues.append(mp.re(x))
        else:
            GOOD=False
            print('H FAILS with non-real eigenvalue')
    H_eigenvalues.sort()
    min_H_eigenvalue = H_eigenvalues[0]
    if min_H_eigenvalue > 0:
        property_P = True
    else:
        GOOD=False
        print('FAILS Property P')
    return

```

In [12]:

```

def calculate_frequencies():
    global Mi_phys,Mi_eigenvalues,positive_frequencies,negative_frequencies,min_frequency,MiR,GOOD,f
    if not aeq(Mi_phys.transpose_conj()*H, H*Mi_phys):
        GOOD=False
        print('FAIL Mi_phys is not H-hermitian')
    Mi_eigenvalues_complex,MiR = mp.eig(Mi_phys)
    Mi_eigenvalues=[]
    for x in Mi_eigenvalues_complex:
        if a0(mp.im(x)):
            Mi_eigenvalues.append(mp.re(x))
        else:
            GOOD=False
            pretty_print('Mi FAILS: non-real eigenvalue')
    positive_frequencies =[]

```

```

negative_frequencies = []
for x in Mi_eigenvalues:
    if x < 0:
        GOOD=False
        print('FAIL: Mi_phys negative eigenvalue')
    else:
        freq = mp.ln(x)/(4*Jac_Kp)
        if freq == 0:
            GOOD=False
            print('FAIL zero frequency')
        if freq < 0:
            negative_frequencies.append(freq)
        else:
            positive_frequencies.append(freq)
if(len(negative_frequencies) != len(positive_frequencies)):
    GOOD=False
    print('FAIL Mi_phys number of positive and negative frequencies differ')
negative_frequencies.sort(reverse=True)
positive_frequencies.sort()
for neg,pos in zip(negative_frequencies,positive_frequencies):
    if not aeq(-neg,pos):
        GOOD=False
        print('FAIL frequencies not in +- pairs')
min_frequency = positive_frequencies[0]
fs_ratio= (min_frequency/sigmaval)^2
if N == 3:
    if not aeq(positive_frequencies[0],positive_frequencies[1]):
        print('DEGENERACY BROKEN')

```

## subroutines for the ode solver

- initial condition at  $\tau = 0$  is  $y_0 = 1$  the identity matrix
- K2mat, K1mat, K0mat are numerical matrices provided by Sagemath
- $y\_deriv(\tau,y)$  calculates  $\partial_\tau y = -iA(\tau)y$
- for the ode solver, the complex matrix  $y$  is converted to a flat list of real numbers
- the solution  $mp.odefun(y\_deriv,0,y\_init)$  is function of  $\tau$  that returns a flat list.
- The propagator  $P(\tau)$  is extracted from the solution function.

```

In [13]: def create_ode():
    global cPlist,K0,K1,K2
    K0matval = K0mat.subs(alpha=alphaval)
    K2 = mpify_matrix(K2mat)
    K1 = mpify_matrix(K1mat*sigmaval)
    K0 = mpify_matrix(K0matval*sigmaval^2)
    # create ode
    cPlist = mp.odefun(y_deriv ,0,y_init,tol=ode_tol,degree=ode_degree)

```

```

In [14]: def construct_gauge():
    global Wgauge, Wpgauge, Proj_gauge, Proj_phys
    w0matval = w0mat.subs(alpha=alphaval)
    w1 = w1mat.change_ring(myC)
    w0 = (w0matval * sigmaval).change_ring(myC)
    zeroNvector = matrix(N,1)
    W0 = mpify_matrix(block_matrix(2,1,[w0,zeroNvector]))
    W1 = mpify_matrix(block_matrix(2,1,[w1,zeroNvector]))
    Wlp = mpify_matrix(block_matrix(2,1,[zeroNvector,w1]))
    Wgauge = W0 + W1*F_at_K+ Wlp*Fp_at_K
    Wpgauge = mp.j*Omega*Wgauge
    Proj_gauge = mp.eye(int(Crank)) - Wpgauge * mp.inverse(Wpgauge.transpose()*Wpgauge) * Wpgauge.tr
    Proj_phys = Proj_gauge - Wgauge* mp.inverse(Wgauge.transpose()*Wgauge) * Wgauge.transpose()

```

```

In [15]: def y_deriv(tau,y):
    # y is a list of length 4N * Crank
    #     representing wr, wr', wi, wi'
    #
    Fi = -Jac_k * Jac_kp * mp.ellipfun('sd',u=tau,m=Jac_mp)
    Kr = K2*Fi^2 - K0
    Ny_4= N*Crank
    Ny_2= 2* Ny_4
    y1 = y[:Ny_2]
    y2 = y[Ny_2:]
    wr = matrixify_list(y1[:Ny_4],N,Crank)
    wpr = matrixify_list(y1[Ny_4:],N,Crank)

```

```

wi = matrixify_list(y2[:Ny_4],N,Crank)
wpi = matrixify_list(y2[Ny_4:],N,Crank)
dwr = -wpi
dwi = wpr
dwpr = -Kr*wi+ Fi*(K1*wr)
dwpi = Kr*wr + Fi*(K1*wi)
dylist = listify_matrix(dwr) + listify_matrix(dwpr) + listify_matrix(dwi) + listify_matrix(dwpi)
return dylist

```

```

In [16]: def cP(tau):
cPl = cPlist(tau)
cPreal = mp.matrix([cPl[nn:nn+Crank] for nn in range(0,Crank*Crank,Crank)])
cPimag = mp.matrix([cPl[nn:nn+Crank] for nn in range(Crank*Crank,Crank*Rrank,Crank)])
cP_mp = cPreal+mp.j*cPimag
return (cP_mp)

```

## Initialization functions

```

In [17]: def set_ranks():
global Crank, Rrank, IN, ZN, Z2N, Omega, cR, y_init
Crank = 2*N
Rrank = 2*Crank
IN = identity_matrix(Reals,N)
ZN = matrix(Reals,N,N)
I2N = identity_matrix(Reals,2*N)
Z2N = matrix(Reals,2*N,2*N)
Omega_sage = I*block_matrix([[ZN,IN],[-IN,ZN]])
cR_sage= block_matrix([[IN,ZN],[ZN,-IN]])
Omega = mpify_matrix(Omega_sage)
cR = mpify_matrix(cR_sage)
y_init_matrix_sage = block_matrix([[I2N],[Z2N]])
y_init_matrix = mpify_matrix(y_init_matrix_sage)
y_init = listify_matrix(y_init_matrix)

```

```

In [18]: def initialize_ode():
global ode,K2mat,K1mat,K0mat,K1coeff,K0coeff,alphaexp,sigmaexp,gauged,w1mat,w0mat,w0coeff,N
ode = odes[ode_name]
K2mat = ode['K2mat']
K1mat = ode['K1mat']
K0mat = ode['K0mat']
alphaexp = ode['alphaexp']
sigmaexp = ode['sigmaexp']
gauged = ode['gauged']
if gauged:
w1mat = ode['w1mat']
w0mat = ode['w0mat']
N=K2mat.nrows()
set_ranks()

```

## Set precision and tolerances

- mp.dps and decimal\_tol are set in the main code
- mp.dps is the decimal precision for mpmath.
- $10^{-\text{decimal\_tol}}$  is the tolerance for approximate numerical equality.

The precision of Sagemath real and complex numbers is set to match the mpmath precision

```

In [19]: def set_precision():
global binary_precision,Reals, RealNumber, myR, Complexes, ComplexNumber, myC, I, J
global mptol, ode_tol,ode_degree
# mp.dps = decimal_precision
# binary_precision = mp.prec
#
binary_precision=mp.prec
Reals = RealField(binary_precision)
RealNumber = Reals
myR = Reals
Complexes = ComplexField(binary_precision)
ComplexNumber = Complexes
myC = Complexes
I = myC(I)
# set_tolerances

```

```

mptol = mpf(10^(-decimal_tol))
ode_tol = None
ode_degree = None
# print ('mp decimal precision =', decimal_precision, '      mp binary precision = sage binary prec

```

## Set Jacobi parameters

In [20]:

```

def set_Jacobi_parameters():
    global epsilonb, Jac_m, Jac_mp, Jac_k, Jac_kp, Jac_K, Jac_Kp, F_at_K, Fp_at_K
    Jac_m = mpf(1/2) + mpf(epsilonb)^2
    Jac_mp = mpf(1)-Jac_m
    Jac_k = mp.sqrt(Jac_m)
    Jac_kp = mp.sqrt(Jac_mp)
    Jac_K = mp.ellipk(Jac_m)
    Jac_Kp = mp.ellipk(Jac_mp)
    F_at_K = 0.0
    Fp_at_K = - Jac_k* Jac_kp

```

## Utilities

In [21]:

```

%display latex
def LE(str):
    return(LatexExpr(r''+ str))

def flatten_list(L):
    return [val for sublist in L for val in sublist]

def mpify_matrix(matrix_sage):
    return mp.matrix(list(map(list, list(matrix_sage))))

def sagify(x):
    return a.mpmath_to_sage(x, binary_precision)

def sagify_matrix(matrix_mp):
    return matrix([list(map(sagify, sublist)) for sublist in matrix_mp.tolist()])

def matrixify_list(ylist, nrows, ncols):
    return mp.matrix([[ylist[ii+jj] for jj in range(ncols)] for ii in range(0, nrows*ncols, ncols)])

def listify_matrix(mp_matrix):
    return flatten_list(mp_matrix.tolist())

print_digits = 20
def mpstr(x):
    if type(x) is list:
        return list(map(mpstr, x))
    return mp.nstr(x, print_digits)

dictify_vars = lambda *args: {i:eval(i) for i in args}

multby = lambda n, x: [n*item for item in x]

```

## Numerical closeness utilities

$mptol$  = approximate equality tolerance  $z \approx 0 \equiv |z| < mptol$

$a0(x)$  iff  $x.norm() < tol^2$

$aeq(x,y)$  iff  $(x - y).norm() < tol^2$

$clean(x)$

- if  $x$  real, if  $a0(x)$  set  $x=0$
- if  $x$  complex, set real and imaginary parts to 0 if  $a0$
- otherwise assume  $x$  is a matrix and clean its entries

In [22]:

```

def almosteq(x,y):
    return(mp.almosteq(x,y,mptol))
#
def aeq(x,y):
    if isinstance(x, mp.mpf) or isinstance(x, mp.mpc):
        return(almosteq(x,y))

```

```

if isinstance(x,mp.matrix):
    return(almosteq(mp.norm(x-y),0))
def a0(x):
    if isinstance(x,mp.mpf) or isinstance(x,mp.mpc):
        return(almosteq(x,0))
    if isinstance(x,mp.matrix):
        return(almosteq(mp.norm(x),0))
def clean(x):
    if isinstance(x,mpf):
        y=x
        if a0(y):
            y = mpf(0)
        if aeq(y,1.0):
            y = mpf(1.0)
        if aeq(y,-1.0):
            y = mpf(-1.0)
        return y
    if isinstance(x,mpc):
        xRe=clean(mp.re(x))
        xIm=clean(mp.im(x))
        if xIm == mpf(0):
            return(xRe)
        elif xRe == mpf(0):
            return(mp.j*xIm)
        else:
            return (xRe + mp.j* xIm)
    if type(x) is list:
        return(list(map(clean,x)))
    if isinstance(x,mp.matrix):
        xrows=x.rows
        xcols=x.cols
        y = mp.matrix(xrows,xcols)
        for i in range(xrows):
            for j in range(xcols):
                y[i,j]= clean(x[i,j])
        return y

```

## Global variables

In [23]:

```

#      global Crank, Rrank, IN, ZN, Z2N, Omega, cR, y_init
#      global ode,K2mat,K1mat,K0mat,K1coeff,K0coeff,alphaexp,sigmaexp,gauged,wlmat,w0mat,w0coeff,N
#      global alpha_asymp, K0mat_asymp, w0mat_asymp
#      global binary_precision,Reals, RealNumber, myR, Complexes, ComplexNumber, myC, I, J
#      global epsilonb,Jac_m,Jac_mp,Jac_k,Jac_kp,Jac_K,Jac_Kp,F_at_t,Fp_at_t
#      global mptol, ode_tol,ode_degree
#      global cPlist,K0,K1,K2, Wgauge, Wpgauge, Proj_gauge, Proj_phys
#      global Mi4,Mi2,Mi
#      global GOOD
#      global Vmat,GOOD
#      global Mi_phys, Omega_phys,GOOD
#      global H,H_eigenvalues,property_P,min_H_eigenvalue,HR,GOOD
#      global Mi_phys,Mi_eigenvalues,positive_frequencies,negative_frequencies,min_frequency,MiR,GOOD

```

## Check gauge invariance of $P(\tau)$

This can be used after a run, i.e. after an ode solution is found.

In [24]:

```

def F(tau):
    return(Jac_k* mp.ellipfun('cn',u=Jac_K+mp.j*tau,m=Jac_m))
def Fp(tau):
    return(- Jac_k* mp.ellipfun('sn',u=Jac_K+mp.j*tau,m=Jac_m)* mp.ellipfun('dn',u=Jac_K+mp.j*tau,m=Jac_m))
def Fi(tau):
    return(-Jac_k * Jac_kp * mp.ellipfun('sd',u=tau,m=Jac_mp))
def Wg(tau):
    w0matval = w0mat.subs(alpha=alphaval)
    w1 = wlmat.change_ring(myC)
    w0 = (w0matval * w0coeff.subs(sigma=sigmaeval)).change_ring(myC)
    zeroNvector = matrix(N,1)
    W0 = mpify_matrix(block_matrix(2,1,[w0,zeroNvector]))
    W1 = mpify_matrix(block_matrix(2,1,[w1,zeroNvector]))
    W1p = mpify_matrix(block_matrix(2,1,[zeroNvector,w1]))
    return(W0 + W1*F(tau)+ W1p*Fp(tau))

```

# Run the analyses

Integrating the ode requires a certain decimal precision in the ode solver.

For each calculation below the decimal precision has been set by trial and error.

Various consistency checks were made on each calculation.

The decimal precision was raised until all the consistency checks were passed.

## load the odes, set precision and tolerance

```
In [25]: odes=load('odes')
high_decimal_precision=300
mp.dps= high_decimal_precision
decimal_tol = 20
data = {}
```

## Ode 2

```
In [26]: ode_name='2'
data[ode_name]={}
```

```
In [27]: ode_decimal_precision = 30
epsilon_list = [0.001,0.002,0.003,0.004,0.005,0.01,0.02,0.03,0.04,0.05,0.1,0.2,0.3,0.4,0.5,0.6,0.70]
process_ode2_epsilon_list()
```

|                    |                   |                     |                           |         |                  |                     |
|--------------------|-------------------|---------------------|---------------------------|---------|------------------|---------------------|
| $\epsilon = 0.001$ | $j = \text{None}$ | $\sigma = 0.000707$ | $(\omega/\sigma)^2 = 2.0$ | (30,20) | ode time =4.6006 | other time =0.76988 |
| $\epsilon = 0.002$ | $j = \text{None}$ | $\sigma = 0.00141$  | $(\omega/\sigma)^2 = 2.0$ | (30,20) | ode time =4.4197 | other time =0.27256 |
| $\epsilon = 0.003$ | $j = \text{None}$ | $\sigma = 0.00212$  | $(\omega/\sigma)^2 = 2.0$ | (30,20) | ode time =4.3831 | other time =0.27702 |
| $\epsilon = 0.004$ | $j = \text{None}$ | $\sigma = 0.00283$  | $(\omega/\sigma)^2 = 2.0$ | (30,20) | ode time =4.3885 | other time =0.27746 |
| $\epsilon = 0.005$ | $j = \text{None}$ | $\sigma = 0.00354$  | $(\omega/\sigma)^2 = 2.0$ | (30,20) | ode time =4.3839 | other time =0.27714 |
| $\epsilon = 0.01$  | $j = \text{None}$ | $\sigma = 0.00707$  | $(\omega/\sigma)^2 = 2.0$ | (30,20) | ode time =4.3782 | other time =0.27009 |
| $\epsilon = 0.02$  | $j = \text{None}$ | $\sigma = 0.0141$   | $(\omega/\sigma)^2 = 2.0$ | (30,20) | ode time =4.3872 | other time =0.26741 |
| $\epsilon = 0.03$  | $j = \text{None}$ | $\sigma = 0.0212$   | $(\omega/\sigma)^2 = 2.0$ | (30,20) | ode time =4.3786 | other time =0.26892 |
| $\epsilon = 0.04$  | $j = \text{None}$ | $\sigma = 0.0283$   | $(\omega/\sigma)^2 = 2.0$ | (30,20) | ode time =4.3819 | other time =0.26734 |
| $\epsilon = 0.05$  | $j = \text{None}$ | $\sigma = 0.0354$   | $(\omega/\sigma)^2 = 2.0$ | (30,20) | ode time =4.3894 | other time =0.26634 |
| $\epsilon = 0.1$   | $j = \text{None}$ | $\sigma = 0.0707$   | $(\omega/\sigma)^2 = 2.0$ | (30,20) | ode time =4.3721 | other time =0.26822 |
| $\epsilon = 0.2$   | $j = \text{None}$ | $\sigma = 0.141$    | $(\omega/\sigma)^2 = 2.0$ | (30,20) | ode time =3.9470 | other time =0.26340 |
| $\epsilon = 0.3$   | $j = \text{None}$ | $\sigma = 0.212$    | $(\omega/\sigma)^2 = 2.0$ | (30,20) | ode time =3.8780 | other time =0.26140 |
| $\epsilon = 0.4$   | $j = \text{None}$ | $\sigma = 0.283$    | $(\omega/\sigma)^2 = 2.0$ | (30,20) | ode time =3.8319 | other time =0.25747 |
| $\epsilon = 0.5$   | $j = \text{None}$ | $\sigma = 0.354$    | $(\omega/\sigma)^2 = 2.0$ | (30,20) | ode time =3.3270 | other time =0.25333 |
| $\epsilon = 0.6$   | $j = \text{None}$ | $\sigma = 0.424$    | $(\omega/\sigma)^2 = 2.0$ | (30,20) | ode time =2.8495 | other time =0.24138 |



$\epsilon = 0.7071$   $j = \text{None}$   $\sigma = 0.500$   $(\omega/\sigma)^2 = 2.0$  (30,20) ode time =1.0870 other time =0.19430

## Ode 3<sub>j</sub>

In [28]:

```
ode_name='3j'  
data[ode_name]={}  
data[ode_name]['asympt']={}  
data[ode_name]['finite']={}
```

### j finite

In [29]:

```
epsilonb = 0.7071  
  
ode_decimal_precision = 30  
j_list = [3/2]  
process_j_list()  
  
ode_decimal_precision = 40  
j_list = [2,5/2]  
process_j_list()  
  
ode_decimal_precision = 50  
j_list = [3,7/2,4]  
process_j_list()  
  
ode_decimal_precision = 60  
j_list = [9/2,5]  
process_j_list()
```

$\epsilon = 0.7071$   $j = \frac{3}{2}$   $\sigma = 0.816$   $(\omega/\sigma)^2 = 4.4999834016824557022$  (30,20) ode time =1.3931 other time :

$\epsilon = 0.7071$   $j = 2$   $\sigma = 1.12$   $(\omega/\sigma)^2 = 5.1999897704981085583$  (40,20) ode time =3.3838 other time =0

$\epsilon = 0.7071$   $j = \frac{5}{2}$   $\sigma = 1.41$   $(\omega/\sigma)^2 = 5.4999932868850748519$  (40,20) ode time =3.3771 other time =

$\epsilon = 0.7071$   $j = 3$   $\sigma = 1.71$   $(\omega/\sigma)^2 = 5.6571381458966265831$  (50,20) ode time =7.4176 other time =1

$\epsilon = 0.7071$   $j = \frac{7}{2}$   $\sigma = 2.00$   $(\omega/\sigma)^2 = 5.749996519696881626$  (50,20) ode time =7.4287 other time =1

$\epsilon = 0.7071$   $j = 4$   $\sigma = 2.29$   $(\omega/\sigma)^2 = 5.8095211363058142583$  (50,20) ode time =7.4138 other time =1

$\epsilon = 0.7071$   $j = \frac{9}{2}$   $\sigma = 2.58$   $(\omega/\sigma)^2 = 5.849997883443329219$  (60,20) ode time =14.721 other time =2

$\epsilon = 0.7071$   $j = 5$   $\sigma = 2.87$   $(\omega/\sigma)^2 = 5.8787861619461414304$  (60,20) ode time =14.702 other time =2

In [30]:

```
epsilonb = 0.55  
  
ode_decimal_precision = 30  
j_list = [3/2,2]  
process_j_list()  
  
ode_decimal_precision = 40  
j_list = [5/2,3,7/2]  
process_j_list()
```

$\epsilon = 0.55$   $j = \frac{3}{2}$   $\sigma = 0.635$   $(\omega/\sigma)^2 = 4.0119140651818690656$  (30,20) ode time =3.5293 other time =0

$\epsilon = 0.55$   $j = 2$   $\sigma = 0.870$   $(\omega/\sigma)^2 = 4.8782922295280631875$  (30,20) ode time =3.5297 other time =0.3

$\epsilon = 0.55$   $j = \frac{5}{2}$   $\sigma = 1.10$   $(\omega/\sigma)^2 = 5.284176568320185352$  (40,20) ode time =9.1205 other time =0.81

$\epsilon = 0.55$   $j = 3$   $\sigma = 1.33$   $(\omega/\sigma)^2 = 5.5041350396067247139$  (40,20) ode time =9.1109 other time =0.82

$\epsilon = 0.55$   $j = \frac{7}{2}$   $\sigma = 1.56$   $(\omega/\sigma)^2 = 5.6363382785629739775$  (40,20) ode time =9.1179 other time =0.8

In [31]:

```
epsilonb = 0.4

ode_decimal_precision = 30
j_list = [3/2, 2, 5/2]
process_j_list()

ode_decimal_precision = 40
j_list = [3, 7/2]
process_j_list()
```

$\epsilon = 0.4$   $j = \frac{3}{2}$   $\sigma = 0.462$   $(\omega/\sigma)^2 = 3.3043168365709716246$  (30,20) ode time =4.5847 other time =0.3

$\epsilon = 0.4$   $j = 2$   $\sigma = 0.632$   $(\omega/\sigma)^2 = 4.2926629349963078598$  (30,20) ode time =4.5846 other time =0.34

$\epsilon = 0.4$   $j = \frac{5}{2}$   $\sigma = 0.800$   $(\omega/\sigma)^2 = 4.8595368961520156711$  (30,20) ode time =4.5844 other time =0.3

$\epsilon = 0.4$   $j = 3$   $\sigma = 0.966$   $(\omega/\sigma)^2 = 5.192260255551817162$  (40,20) ode time =10.749 other time =0.845

$\epsilon = 0.4$   $j = \frac{7}{2}$   $\sigma = 1.13$   $(\omega/\sigma)^2 = 5.4001919850822057902$  (40,20) ode time =10.755 other time =0.85

In [32]:

```
epsilonb = 0.3

ode_decimal_precision = 30
j_list = [3/2, 2, 5/2, 3]
process_j_list()

ode_decimal_precision = 40
j_list = [7/2]
process_j_list()
```

$\epsilon = 0.3$   $j = \frac{3}{2}$   $\sigma = 0.346$   $(\omega/\sigma)^2 = 2.7500646261884110787$  (30,20) ode time =4.6443 other time =0.3

$\epsilon = 0.3$   $j = 2$   $\sigma = 0.474$   $(\omega/\sigma)^2 = 3.6234231561114523133$  (30,20) ode time =4.6397 other time =0.34

$\epsilon = 0.3$   $j = \frac{5}{2}$   $\sigma = 0.600$   $(\omega/\sigma)^2 = 4.2932101870569633592$  (30,20) ode time =4.6422 other time =0.3

$\epsilon = 0.3$   $j = 3$   $\sigma = 0.725$   $(\omega/\sigma)^2 = 4.7452772824302272425$  (30,20) ode time =4.6379 other time =0.34

$\epsilon = 0.3$   $j = \frac{7}{2}$   $\sigma = 0.849$   $(\omega/\sigma)^2 = 5.0484406379829194185$  (40,20) ode time =12.154 other time =0.8

In [33]:

```
epsilonb = 0.01

ode_decimal_precision = 30
j_list = [3/2, 2, 5/2, 3, 7/2, 5, 10, 15, 20, 30, 40, 50, 60, 70, 80, 90]
process_j_list()

ode_decimal_precision = 40
j_list = [100, 120, 140, 160]
process_j_list()

ode_decimal_precision = 50
j_list = [180, 200, 230]
process_j_list()

ode_decimal_precision = 70
j_list = [260, 290, 320, 350]
process_j_list()
```

$\epsilon = 0.01$   $j = \frac{3}{2}$   $\sigma = 0.0115$   $(\omega/\sigma)^2 = 2.0006096917743312498$  (30,20) ode time =5.2208 other time =0.3

$\epsilon = 0.01$   $j = 2$   $\sigma = 0.0158$   $(\omega/\sigma)^2 = 2.001464161862771762$  (30,20) ode time =5.2136 other time =0.3

$\epsilon = 0.01$   $j = \frac{5}{2}$   $\sigma = 0.0200$   $(\omega/\sigma)^2 = 2.0025643102199197761$  (30,20) ode time =5.2110 other time =0.3

$\epsilon = 0.01$   $j = 3$   $\sigma = 0.0242$   $(\omega/\sigma)^2 = 2.0039112915562727295$  (30,20) ode time =5.2180 other time =0

$\epsilon = 0.01$   $j = \frac{7}{2}$   $\sigma = 0.0283$   $(\omega/\sigma)^2 = 2.005506513527785117$  (30,20) ode time =5.2142 other time =0

$\epsilon = 0.01$   $j = 5$   $\sigma = 0.0406$   $(\omega/\sigma)^2 = 2.0117994436223473306$  (30,20) ode time =5.2140 other time =0

$\epsilon = 0.01$   $j = 10$   $\sigma = 0.0816$   $(\omega/\sigma)^2 = 2.049915088956064386$  (30,20) ode time =5.2188 other time =0

$\epsilon = 0.01$   $j = 15$   $\sigma = 0.122$   $(\omega/\sigma)^2 = 2.1173874742746105617$  (30,20) ode time =5.2201 other time =0

$\epsilon = 0.01$   $j = 20$   $\sigma = 0.163$   $(\omega/\sigma)^2 = 2.2191564847884813161$  (30,20) ode time =5.2160 other time =0

$\epsilon = 0.01$   $j = 30$   $\sigma = 0.245$   $(\omega/\sigma)^2 = 2.5408502878760358795$  (30,20) ode time =5.2151 other time =0

$\epsilon = 0.01$   $j = 40$   $\sigma = 0.327$   $(\omega/\sigma)^2 = 3.0023297892601524571$  (30,20) ode time =5.2159 other time =0

$\epsilon = 0.01$   $j = 50$   $\sigma = 0.408$   $(\omega/\sigma)^2 = 3.5145618548029226805$  (30,20) ode time =5.2127 other time =0

|                   |           |                  |                                             |         |                  |                 |
|-------------------|-----------|------------------|---------------------------------------------|---------|------------------|-----------------|
| $\epsilon = 0.01$ | $j = 60$  | $\sigma = 0.490$ | $(\omega/\sigma)^2 = 3.9836417374816104468$ | (30,20) | ode time =5.2192 | other time =0   |
| $\epsilon = 0.01$ | $j = 70$  | $\sigma = 0.572$ | $(\omega/\sigma)^2 = 4.3691189358253653385$ | (30,20) | ode time =5.2169 | other time =0   |
| $\epsilon = 0.01$ | $j = 80$  | $\sigma = 0.653$ | $(\omega/\sigma)^2 = 4.6713878684154581544$ | (30,20) | ode time =5.2242 | other time =0   |
| $\epsilon = 0.01$ | $j = 90$  | $\sigma = 0.735$ | $(\omega/\sigma)^2 = 4.905275304219552021$  | (30,20) | ode time =5.2145 | other time =0.5 |
| $\epsilon = 0.01$ | $j = 100$ | $\sigma = 0.816$ | $(\omega/\sigma)^2 = 5.086722917739205928$  | (40,20) | ode time =12.503 | other time =0   |
| $\epsilon = 0.01$ | $j = 120$ | $\sigma = 0.980$ | $(\omega/\sigma)^2 = 5.3414664711113240511$ | (40,20) | ode time =12.492 | other time =0   |
| $\epsilon = 0.01$ | $j = 140$ | $\sigma = 1.14$  | $(\omega/\sigma)^2 = 5.5053424306333022703$ | (40,20) | ode time =13.734 | other time =0   |
| $\epsilon = 0.01$ | $j = 160$ | $\sigma = 1.31$  | $(\omega/\sigma)^2 = 5.615886790683154156$  | (40,20) | ode time =13.737 | other time =0.8 |
| $\epsilon = 0.01$ | $j = 180$ | $\sigma = 1.47$  | $(\omega/\sigma)^2 = 5.6935841252232656642$ | (50,20) | ode time =29.015 | other time =2   |
| $\epsilon = 0.01$ | $j = 200$ | $\sigma = 1.63$  | $(\omega/\sigma)^2 = 5.7501133827543736513$ | (50,20) | ode time =28.999 | other time =2   |
| $\epsilon = 0.01$ | $j = 230$ | $\sigma = 1.88$  | $(\omega/\sigma)^2 = 5.8097230117170114877$ | (50,20) | ode time =31.901 | other time =2   |
| $\epsilon = 0.01$ | $j = 260$ | $\sigma = 2.12$  | $(\omega/\sigma)^2 = 5.8504005667678360068$ | (70,20) | ode time =109.08 | other time =8   |
| $\epsilon = 0.01$ | $j = 290$ | $\sigma = 2.37$  | $(\omega/\sigma)^2 = 5.8793547844855359812$ | (70,20) | ode time =109.11 | other time =8   |
| $\epsilon = 0.01$ | $j = 320$ | $\sigma = 2.61$  | $(\omega/\sigma)^2 = 5.9006771964032691039$ | (70,20) | ode time =109.09 | other time =8   |
| $\epsilon = 0.01$ | $j = 350$ | $\sigma = 2.86$  | $(\omega/\sigma)^2 = 5.9168241864476698865$ | (70,20) | ode time =109.09 | other time =8   |
| $j = \infty$      |           |                  |                                             |         |                  |                 |

In [34]:

```
ode_decimal_precision = 30
sigma_list = [0.02,0.04,.06,.08,.10,0.15,0.2,0.25,0.3,0.35,0.4,0.45,0.5,0.55,.6,0.65,0.7,0.75]
process_sigma_list()

ode_decimal_precision = 40
sigma_list = [0.8,0.85,0.9,0.95,1,1.2]
process_sigma_list()

ode_decimal_precision = 50
sigma_list = [1.4,1.6,1.8]
process_sigma_list()

ode_decimal_precision = 60
sigma_list = [2.0,2.2,2.4,2.6]
process_sigma_list()

ode_decimal_precision = 70
```

```
sigma_list = [2.8,3.0]
process_sigma_list()
```

|                 |               |                   |                                             |         |                  |                  |
|-----------------|---------------|-------------------|---------------------------------------------|---------|------------------|------------------|
| $\epsilon = 0.$ | $j = +\infty$ | $\sigma = 0.0200$ | $(\omega/\sigma)^2 = 2.0029306396589592143$ | (30,20) | ode time =5.2236 | other time =0.   |
| $\epsilon = 0.$ | $j = +\infty$ | $\sigma = 0.0400$ | $(\omega/\sigma)^2 = 2.01179637058130815$   | (30,20) | ode time =5.2160 | other time =0.35 |
| $\epsilon = 0.$ | $j = +\infty$ | $\sigma = 0.0600$ | $(\omega/\sigma)^2 = 2.026815783726084496$  | (30,20) | ode time =5.2137 | other time =0.3  |
| $\epsilon = 0.$ | $j = +\infty$ | $\sigma = 0.0800$ | $(\omega/\sigma)^2 = 2.0483431301388165799$ | (30,20) | ode time =5.2211 | other time =0.   |
| $\epsilon = 0.$ | $j = +\infty$ | $\sigma = 0.100$  | $(\omega/\sigma)^2 = 2.0768512508711160382$ | (30,20) | ode time =5.2145 | other time =0.3  |
| $\epsilon = 0.$ | $j = +\infty$ | $\sigma = 0.150$  | $(\omega/\sigma)^2 = 2.1824734440870033519$ | (30,20) | ode time =5.2211 | other time =0.3  |
| $\epsilon = 0.$ | $j = +\infty$ | $\sigma = 0.200$  | $(\omega/\sigma)^2 = 2.3443219375813765233$ | (30,20) | ode time =5.2149 | other time =0.3  |
| $\epsilon = 0.$ | $j = +\infty$ | $\sigma = 0.250$  | $(\omega/\sigma)^2 = 2.5665348899140685796$ | (30,20) | ode time =5.2161 | other time =0.3  |
| $\epsilon = 0.$ | $j = +\infty$ | $\sigma = 0.300$  | $(\omega/\sigma)^2 = 2.8416258944066673457$ | (30,20) | ode time =5.2152 | other time =0.3  |
| $\epsilon = 0.$ | $j = +\infty$ | $\sigma = 0.350$  | $(\omega/\sigma)^2 = 3.1493685608081772441$ | (30,20) | ode time =5.2148 | other time =0.3  |
| $\epsilon = 0.$ | $j = +\infty$ | $\sigma = 0.400$  | $(\omega/\sigma)^2 = 3.4640786507796314538$ | (30,20) | ode time =5.2180 | other time =0.3  |
| $\epsilon = 0.$ | $j = +\infty$ | $\sigma = 0.450$  | $(\omega/\sigma)^2 = 3.7641093098968960934$ | (30,20) | ode time =5.2153 | other time =0.3  |
| $\epsilon = 0.$ | $j = +\infty$ | $\sigma = 0.500$  | $(\omega/\sigma)^2 = 4.0364870439793698411$ | (30,20) | ode time =5.2225 | other time =0.3  |
| $\epsilon = 0.$ | $j = +\infty$ | $\sigma = 0.550$  | $(\omega/\sigma)^2 = 4.2762245862832203116$ | (30,20) | ode time =5.2150 | other time =0.3  |
| $\epsilon = 0.$ | $j = +\infty$ | $\sigma = 0.600$  | $(\omega/\sigma)^2 = 4.4835179731049804094$ | (30,20) | ode time =5.2173 | other time =0.3  |
| $\epsilon = 0.$ | $j = +\infty$ | $\sigma = 0.650$  | $(\omega/\sigma)^2 = 4.6611734256132470388$ | (30,20) | ode time =5.2189 | other time =0.3  |
| $\epsilon = 0.$ | $j = +\infty$ | $\sigma = 0.700$  | $(\omega/\sigma)^2 = 4.8129437327005195409$ | (30,20) | ode time =5.2228 | other time =0.3  |
| $\epsilon = 0.$ | $j = +\infty$ | $\sigma = 0.750$  | $(\omega/\sigma)^2 = 4.9426438397638722761$ | (30,20) | ode time =5.2159 | other time =0.3  |
| $\epsilon = 0.$ | $j = +\infty$ | $\sigma = 0.800$  | $(\omega/\sigma)^2 = 5.0537551161551944156$ | (40,20) | ode time =12.484 | other time =0.8  |

|                 |               |                  |                                             |         |                  |                   |
|-----------------|---------------|------------------|---------------------------------------------|---------|------------------|-------------------|
| $\epsilon = 0.$ | $j = +\infty$ | $\sigma = 0.850$ | $(\omega/\sigma)^2 = 5.1492920034437529415$ | (40,20) | ode time =12.465 | other time =0.8   |
|                 |               |                  |                                             |         |                  |                   |
| $\epsilon = 0.$ | $j = +\infty$ | $\sigma = 0.900$ | $(\omega/\sigma)^2 = 5.2317943046322504194$ | (40,20) | ode time =12.489 | other time =0.8   |
|                 |               |                  |                                             |         |                  |                   |
| $\epsilon = 0.$ | $j = +\infty$ | $\sigma = 0.950$ | $(\omega/\sigma)^2 = 5.3033719781498695124$ | (40,20) | ode time =12.477 | other time =0.8   |
|                 |               |                  |                                             |         |                  |                   |
| $\epsilon = 0.$ | $j = +\infty$ | $\sigma = 1.00$  | $(\omega/\sigma)^2 = 5.3657663950167112016$ | (40,20) | ode time =13.708 | other time =0.88  |
|                 |               |                  |                                             |         |                  |                   |
| $\epsilon = 0.$ | $j = +\infty$ | $\sigma = 1.20$  | $(\omega/\sigma)^2 = 5.5486814297827637433$ | (40,20) | ode time =13.738 | other time =0.88  |
|                 |               |                  |                                             |         |                  |                   |
| $\epsilon = 0.$ | $j = +\infty$ | $\sigma = 1.40$  | $(\omega/\sigma)^2 = 5.6635970315408634098$ | (50,20) | ode time =29.013 | other time =2.07  |
|                 |               |                  |                                             |         |                  |                   |
| $\epsilon = 0.$ | $j = +\infty$ | $\sigma = 1.60$  | $(\omega/\sigma)^2 = 5.7400474766166610879$ | (50,20) | ode time =29.027 | other time =2.08  |
|                 |               |                  |                                             |         |                  |                   |
| $\epsilon = 0.$ | $j = +\infty$ | $\sigma = 1.80$  | $(\omega/\sigma)^2 = 5.793310029131846546$  | (50,20) | ode time =31.963 | other time =2.075 |
|                 |               |                  |                                             |         |                  |                   |
| $\epsilon = 0.$ | $j = +\infty$ | $\sigma = 2.00$  | $(\omega/\sigma)^2 = 5.831831372906549483$  | (60,20) | ode time =59.779 | other time =4.433 |
|                 |               |                  |                                             |         |                  |                   |
| $\epsilon = 0.$ | $j = +\infty$ | $\sigma = 2.20$  | $(\omega/\sigma)^2 = 5.8605596139979826243$ | (60,20) | ode time =59.829 | other time =4.44  |
|                 |               |                  |                                             |         |                  |                   |
| $\epsilon = 0.$ | $j = +\infty$ | $\sigma = 2.40$  | $(\omega/\sigma)^2 = 5.8825388177663555004$ | (60,20) | ode time =65.649 | other time =4.46  |
|                 |               |                  |                                             |         |                  |                   |
| $\epsilon = 0.$ | $j = +\infty$ | $\sigma = 2.60$  | $(\omega/\sigma)^2 = 5.8997208734549874499$ | (60,20) | ode time =65.545 | other time =4.42  |
|                 |               |                  |                                             |         |                  |                   |
| $\epsilon = 0.$ | $j = +\infty$ | $\sigma = 2.80$  | $(\omega/\sigma)^2 = 5.9134022698348587444$ | (70,20) | ode time =108.59 | other time =8.31  |
|                 |               |                  |                                             |         |                  |                   |
| $\epsilon = 0.$ | $j = +\infty$ | $\sigma = 3.00$  | $(\omega/\sigma)^2 = 5.9244706315060858988$ | (70,20) | ode time =108.56 | other time =8.31  |
|                 |               |                  |                                             |         |                  |                   |

## Ode 2<sub>j</sub>

In [35]:

```
ode_name='2j'
data[ode_name]={}
data[ode_name]['asympt']={}
data[ode_name]['finite']={}

```

## j finite

In [36]:

```
epsilon_b = 0.7071

ode_decimal_precision = 30
j_list = [3/2]
process_j_list()

ode_decimal_precision = 40
j_list = [2,5/2]
process_j_list()

ode_decimal_precision = 50
j_list = [3,7/2,4]

```

```
process_j_list()

ode_decimal_precision = 60
j_list = [9/2,5]
process_j_list()

ode_decimal_precision = 70
j_list = [11/2]
process_j_list()
```

$\epsilon = 0.7071$   $j = \frac{3}{2}$   $\sigma = 1.06$   $(\omega/\sigma)^2 = 3.111105996386973974$  (30,20) ode time =1.1663 other time =0.

$\epsilon = 0.7071$   $j = 2$   $\sigma = 1.41$   $(\omega/\sigma)^2 = 3.4999961970124620313$  (40,20) ode time =3.0246 other time =0

$\epsilon = 0.7071$   $j = \frac{5}{2}$   $\sigma = 1.77$   $(\omega/\sigma)^2 = 3.6799973229185163812$  (40,20) ode time =3.0261 other time =

$\epsilon = 0.7071$   $j = 3$   $\sigma = 2.12$   $(\omega/\sigma)^2 = 3.7777758319480891792$  (50,20) ode time =6.9061 other time =1

$\epsilon = 0.7071$   $j = \frac{7}{2}$   $\sigma = 2.47$   $(\omega/\sigma)^2 = 3.8367332270254066081$  (50,20) ode time =6.9043 other time =

$\epsilon = 0.7071$   $j = 4$   $\sigma = 2.83$   $(\omega/\sigma)^2 = 3.8749988587702415691$  (50,20) ode time =6.9113 other time =1

$\epsilon = 0.7071$   $j = \frac{9}{2}$   $\sigma = 3.18$   $(\omega/\sigma)^2 = 3.9012336564667336$  (60,20) ode time =14.025 other time =2.56

$\epsilon = 0.7071$   $j = 5$   $\sigma = 3.54$   $(\omega/\sigma)^2 = 3.9199992561534346762$  (60,20) ode time =14.014 other time =2

$\epsilon = 0.7071$   $j = \frac{11}{2}$   $\sigma = 3.89$   $(\omega/\sigma)^2 = 3.9338836793777357288$  (70,20) ode time =25.137 other time :

In [37]:

```
epsilonb = 0.6

ode_decimal_precision = 30
j_list = [3/2]
process_j_list()

ode_decimal_precision = 40
j_list = [2,5/2,3]
process_j_list()

ode_decimal_precision = 50
j_list = [7/2]
process_j_list()

ode_decimal_precision = 50
j_list = [4]
process_j_list()
```

$\epsilon = 0.6$   $j = \frac{3}{2}$   $\sigma = 0.900$   $(\omega/\sigma)^2 = 3.0219757580714899217$  (30,20) ode time =2.6289 other time =0.2

$\epsilon = 0.6$   $j = 2$   $\sigma = 1.20$   $(\omega/\sigma)^2 = 3.4289121173565929182$  (40,20) ode time =7.1452 other time =0.700

$\epsilon = 0.6$   $j = \frac{5}{2}$   $\sigma = 1.50$   $(\omega/\sigma)^2 = 3.628680571286386956$  (40,20) ode time =7.1397 other time =0.698

$\epsilon = 0.6$   $j = 3$   $\sigma = 1.80$   $(\omega/\sigma)^2 = 3.7400155842771586464$  (40,20) ode time =7.1452 other time =0.695

$\epsilon = 0.6$   $j = \frac{7}{2}$   $\sigma = 2.10$   $(\omega/\sigma)^2 = 3.8080686609021688663$  (50,20) ode time =16.961 other time =1.67

$\epsilon = 0.6$   $j = 4$   $\sigma = 2.40$   $(\omega/\sigma)^2 = 3.8525999135959532319$  (50,20) ode time =16.974 other time =1.681

In [38]:

```
epsilonb = 0.5

ode_decimal_precision = 30
j_list = [3/2,2]
process_j_list()

ode_decimal_precision = 40
j_list = [5/2,3,7/2]
process_j_list()

ode_decimal_precision = 50
j_list = [9/2]
process_j_list()

ode_decimal_precision = 60
j_list = [6]
process_j_list()

ode_decimal_precision = 70
j_list = [8]
process_j_list()
```

$\epsilon = 0.5$   $j = \frac{3}{2}$   $\sigma = 0.750$   $(\omega/\sigma)^2 = 2.9252106564059074814$  (30,20) ode time =3.1117 other time =0.2

$\epsilon = 0.5$   $j = 2$   $\sigma = 1.00$   $(\omega/\sigma)^2 = 3.336509692956312181$  (30,20) ode time =3.1070 other time =0.2637

$\epsilon = 0.5$   $j = \frac{5}{2}$   $\sigma = 1.25$   $(\omega/\sigma)^2 = 3.5574871095526227098$  (40,20) ode time =8.5732 other time =0.72

$\epsilon = 0.5$   $j = 3$   $\sigma = 1.50$   $(\omega/\sigma)^2 = 3.6859375596307213748$  (40,20) ode time =8.5624 other time =0.725

$\epsilon = 0.5$   $j = \frac{7}{2}$   $\sigma = 1.75$   $(\omega/\sigma)^2 = 3.766268941358884203$  (40,20) ode time =8.5670 other time =0.722

$\epsilon = 0.5$   $j = \frac{9}{2}$   $\sigma = 2.25$   $(\omega/\sigma)^2 = 3.8566326173765722934$  (50,20) ode time =20.328 other time =1.77

$\epsilon = 0.5$   $j = 6$   $\sigma = 3.00$   $(\omega/\sigma)^2 = 3.9186142347692286407$  (60,20) ode time =42.169 other time =3.865

$\epsilon = 0.5$   $j = 8$   $\sigma = 4.00$   $(\omega/\sigma)^2 = 3.953986459962055927$  (70,20) ode time =77.547 other time =7.3441

In [39]:

```
epsilonb = 0.4
```



```
ode_decimal_precision = 30
j_list = [3/2,2,5/2]
process_j_list()

ode_decimal_precision = 40
j_list = [3,7/2,9/2]
process_j_list()

ode_decimal_precision = 50
j_list = [11/2]
process_j_list()
```

$\epsilon = 0.4$   $j = \frac{3}{2}$   $\sigma = 0.600$   $(\omega/\sigma)^2 = 2.8260860543995007448$  (30,20) ode time =3.6120 other time =0.2

$\epsilon = 0.4$   $j = 2$   $\sigma = 0.800$   $(\omega/\sigma)^2 = 3.2095538197436441631$  (30,20) ode time =3.6121 other time =0.27

$\epsilon = 0.4$   $j = \frac{5}{2}$   $\sigma = 1.00$   $(\omega/\sigma)^2 = 3.448496411453397044$  (30,20) ode time =3.6040 other time =0.271

$\epsilon = 0.4$   $j = 3$   $\sigma = 1.20$   $(\omega/\sigma)^2 = 3.5985568104045214463$  (40,20) ode time =9.9381 other time =0.746

$\epsilon = 0.4$   $j = \frac{7}{2}$   $\sigma = 1.40$   $(\omega/\sigma)^2 = 3.6966042108267113169$  (40,20) ode time =9.9436 other time =0.74

$\epsilon = 0.4$   $j = \frac{9}{2}$   $\sigma = 1.80$   $(\omega/\sigma)^2 = 3.8107346628228260028$  (40,20) ode time =9.9419 other time =0.74

$\epsilon = 0.4$   $j = \frac{11}{2}$   $\sigma = 2.20$   $(\omega/\sigma)^2 = 3.8713285468249709094$  (50,20) ode time =23.727 other time =1.8

In [40]:

```
epsilon_b = 0.325

ode_decimal_precision = 30
j_list = [3/2,2,5/2]
process_j_list()

ode_decimal_precision = 40
j_list = [3,7/2]
process_j_list()
```

$\epsilon = 0.325$   $j = \frac{3}{2}$   $\sigma = 0.487$   $(\omega/\sigma)^2 = 2.7686172645363766041$  (30,20) ode time =3.6586 other time =

$\epsilon = 0.325$   $j = 2$   $\sigma = 0.650$   $(\omega/\sigma)^2 = 3.0910012237972445732$  (30,20) ode time =3.6586 other time =0

$\epsilon = 0.325$   $j = \frac{5}{2}$   $\sigma = 0.812$   $(\omega/\sigma)^2 = 3.3289994780980640365$  (30,20) ode time =3.6567 other time =

$\epsilon = 0.325$   $j = 3$   $\sigma = 0.975$   $(\omega/\sigma)^2 = 3.4945400530890411016$  (40,20) ode time =10.106 other time =0

$\epsilon = 0.325$   $j = \frac{7}{2}$   $\sigma = 1.14$   $(\omega/\sigma)^2 = 3.6096034560197983957$  (40,20) ode time =10.097 other time =0

In [41]:

```
epsilonb = 0.25

ode_decimal_precision = 30
j_list = [3/2, 2, 5/2, 3, 7/2]
process_j_list()

ode_decimal_precision = 40
j_list = [9/2, 13/2]
process_j_list()

ode_decimal_precision = 50
j_list = [8, 10]
process_j_list()

ode_decimal_precision = 70
j_list = [23/2, 13, 29/2]
process_j_list()

ode_decimal_precision = 70
j_list = [16]
process_j_list()
```

$\epsilon = 0.25$   $j = \frac{3}{2}$   $\sigma = 0.375$   $(\omega/\sigma)^2 = 2.7548735658800374599$  (30,20) ode time =4.2099 other time =0

$\epsilon = 0.25$   $j = 2$   $\sigma = 0.500$   $(\omega/\sigma)^2 = 2.9695797955370071617$  (30,20) ode time =4.1040 other time =0.2

$\epsilon = 0.25$   $j = \frac{5}{2}$   $\sigma = 0.625$   $(\omega/\sigma)^2 = 3.1718000990866994758$  (30,20) ode time =4.1106 other time =0

$\epsilon = 0.25$   $j = 3$   $\sigma = 0.750$   $(\omega/\sigma)^2 = 3.3384548001964306367$  (30,20) ode time =4.1044 other time =0.2

$\epsilon = 0.25$   $j = \frac{7}{2}$   $\sigma = 0.875$   $(\omega/\sigma)^2 = 3.4682100918407403594$  (30,20) ode time =4.1099 other time =0

$\epsilon = 0.25$   $j = \frac{9}{2}$   $\sigma = 1.12$   $(\omega/\sigma)^2 = 3.6434974763842416896$  (40,20) ode time =10.253 other time =0.7

$\epsilon = 0.25$   $j = \frac{13}{2}$   $\sigma = 1.62$   $(\omega/\sigma)^2 = 3.814084315501186252$  (40,20) ode time =11.384 other time =0.7

$\epsilon = 0.25$   $j = 8$   $\sigma = 2.00$   $(\omega/\sigma)^2 = 3.8739450433276470651$  (50,20) ode time =24.435 other time =1.87

$\epsilon = 0.25$   $j = 10$   $\sigma = 2.50$   $(\omega/\sigma)^2 = 3.917799937383960746$  (50,20) ode time =27.144 other time =1.88

$\epsilon = 0.25$   $j = \frac{23}{2}$   $\sigma = 2.88$   $(\omega/\sigma)^2 = 3.937337767536398566$  (70,20) ode time =93.658 other time =7.9

$\epsilon = 0.25$   $j = 13$   $\sigma = 3.25$   $(\omega/\sigma)^2 = 3.9506944761876452264$  (70,20) ode time =93.619 other time =7.9

$\epsilon = 0.25$   $j = \frac{29}{2}$   $\sigma = 3.62$   $(\omega/\sigma)^2 = 3.96021425385399209$  (70,20) ode time =104.05 other time =7.93

$\epsilon = 0.25$   $j = 16$   $\sigma = 4.00$   $(\omega/\sigma)^2 = 3.9672316450013068105$  (70,20) ode time =104.01 other time =7.9

In [42]:

```
epsilonb = 0.2
ode_decimal_precision = 30
j_list = [3/2, 2, 5/2, 3, 7/2]
process_j_list()
```

$\epsilon = 0.2$   $j = \frac{3}{2}$   $\sigma = 0.300$   $(\omega/\sigma)^2 = 2.7900223637150635907$  (30,20) ode time =4.1372 other time =0.2

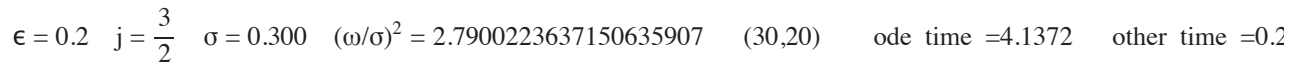

$\epsilon = 0.2$   $j = 2$   $\sigma = 0.400$   $(\omega/\sigma)^2 = 2.911889776281244591$  (30,20) ode time =4.1461 other time =0.277

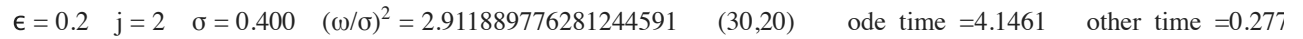

$\epsilon = 0.2$   $j = \frac{5}{2}$   $\sigma = 0.500$   $(\omega/\sigma)^2 = 3.0584348766204516843$  (30,20) ode time =4.1318 other time =0.2

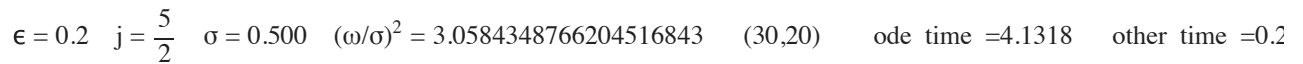

$\epsilon = 0.2$   $j = 3$   $\sigma = 0.600$   $(\omega/\sigma)^2 = 3.2022972174391099247$  (30,20) ode time =4.1413 other time =0.28

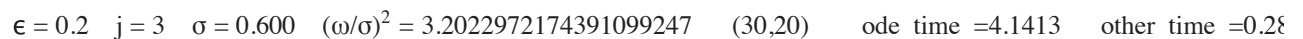

$\epsilon = 0.2$   $j = \frac{7}{2}$   $\sigma = 0.700$   $(\omega/\sigma)^2 = 3.3295574084657802527$  (30,20) ode time =4.1351 other time =0.2

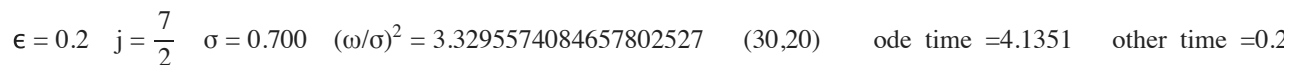

In [43]:

```
epsilonb = 0.15
ode_decimal_precision = 30
j_list = [3/2, 2, 5/2, 3, 7/2]
process_j_list()
```

$\epsilon = 0.15$   $j = \frac{3}{2}$   $\sigma = 0.225$   $(\omega/\sigma)^2 = 2.8767082020777589107$  (30,20) ode time =4.1428 other time =0

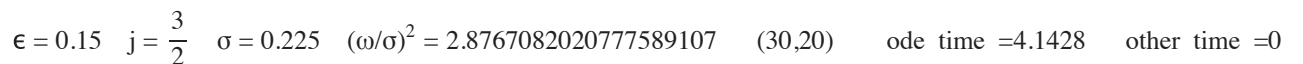

$\epsilon = 0.15$   $j = 2$   $\sigma = 0.300$   $(\omega/\sigma)^2 = 2.9060034398802915749$  (30,20) ode time =4.1402 other time =0.2

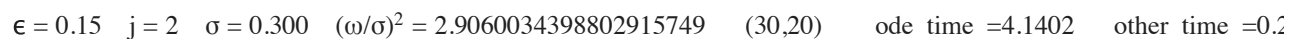

$\epsilon = 0.15$   $j = \frac{5}{2}$   $\sigma = 0.375$   $(\omega/\sigma)^2 = 2.9730112551102726957$  (30,20) ode time =4.1373 other time =0.

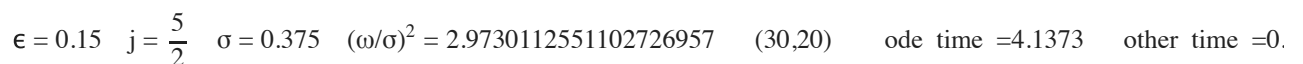

$\epsilon = 0.15$   $j = 3$   $\sigma = 0.450$   $(\omega/\sigma)^2 = 3.0622401264067358881$  (30,20) ode time =4.1603 other time =0.2

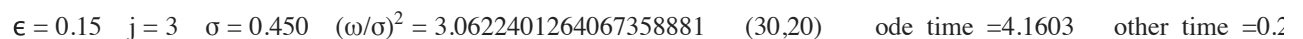

$\epsilon = 0.15$   $j = \frac{7}{2}$   $\sigma = 0.525$   $(\omega/\sigma)^2 = 3.1595334734424986648$  (30,20) ode time =4.1475 other time =0

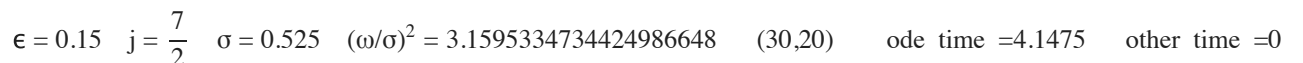

In [44]:

```
epsilonb = 0.125
ode_decimal_precision = 30
j_list = [3/2, 2, 5/2, 3, 7/2]
process_j_list()
```

$\epsilon = 0.125$   $j = \frac{3}{2}$   $\sigma = 0.188$   $(\omega/\sigma)^2 = 2.9419804646675092648$  (30,20) ode time =4.1639 other time =

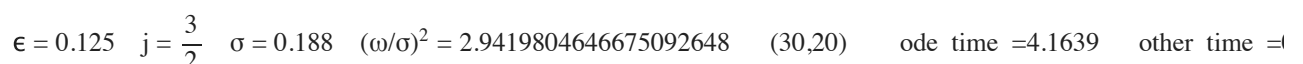

$\epsilon = 0.125$   $j = 2$   $\sigma = 0.250$   $(\omega/\sigma)^2 = 2.933976756786076842$  (30,20) ode time =4.1609 other time =0.2

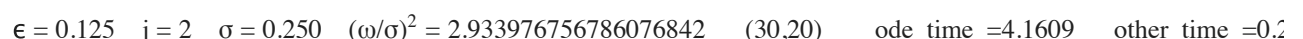

$\epsilon = 0.125$   $j = \frac{5}{2}$   $\sigma = 0.312$   $(\omega/\sigma)^2 = 2.9591701577989723021$  (30,20) ode time =4.1634 other time =

$\epsilon = 0.125$   $j = 3$   $\sigma = 0.375$   $(\omega/\sigma)^2 = 3.0103722063219255875$  (30,20) ode time =4.1644 other time =0

$\epsilon = 0.125$   $j = \frac{7}{2}$   $\sigma = 0.438$   $(\omega/\sigma)^2 = 3.0780823512890894891$  (30,20) ode time =4.1616 other time =

In [45]:

```
epsilonb = 0.1
ode_decimal_precision = 30
j_list = [3/2, 2, 5/2, 3, 7/2, 4]
process_j_list()
```

$\epsilon = 0.1$   $j = \frac{3}{2}$   $\sigma = 0.150$   $(\omega/\sigma)^2 = 3.0202372938491234705$  (30,20) ode time =4.1767 other time =0.2

$\epsilon = 0.1$   $j = 2$   $\sigma = 0.200$   $(\omega/\sigma)^2 = 2.9874597291297524231$  (30,20) ode time =4.1706 other time =0.28

$\epsilon = 0.1$   $j = \frac{5}{2}$   $\sigma = 0.250$   $(\omega/\sigma)^2 = 2.9771606541773666915$  (30,20) ode time =4.1698 other time =0.2

$\epsilon = 0.1$   $j = 3$   $\sigma = 0.300$   $(\omega/\sigma)^2 = 2.9892814480213505723$  (30,20) ode time =4.1694 other time =0.28

$\epsilon = 0.1$   $j = \frac{7}{2}$   $\sigma = 0.350$   $(\omega/\sigma)^2 = 3.0200780860474762668$  (30,20) ode time =4.1726 other time =0.2

$\epsilon = 0.1$   $j = 4$   $\sigma = 0.400$   $(\omega/\sigma)^2 = 3.0645544106568858882$  (30,20) ode time =4.1752 other time =0.28

In [46]:

```
epsilonb = 0.08
ode_decimal_precision = 30
j_list = [3/2, 2, 5/2, 3, 7/2, 4]
process_j_list()
```

$\epsilon = 0.08$   $j = \frac{3}{2}$   $\sigma = 0.120$   $(\omega/\sigma)^2 = 3.0885824003150966159$  (30,20) ode time =4.1877 other time =0

$\epsilon = 0.08$   $j = 2$   $\sigma = 0.160$   $(\omega/\sigma)^2 = 3.0482652232348396391$  (30,20) ode time =4.1732 other time =0.2

$\epsilon = 0.08$   $j = \frac{5}{2}$   $\sigma = 0.200$   $(\omega/\sigma)^2 = 3.0195927817201708685$  (30,20) ode time =4.1777 other time =0

$\epsilon = 0.08$   $j = 3$   $\sigma = 0.240$   $(\omega/\sigma)^2 = 3.0059180001580421244$  (30,20) ode time =4.1736 other time =0.2

$\epsilon = 0.08$   $j = \frac{7}{2}$   $\sigma = 0.280$   $(\omega/\sigma)^2 = 3.0073934028957272796$  (30,20) ode time =4.1771 other time =0

$\epsilon = 0.08$   $j = 4$   $\sigma = 0.320$   $(\omega/\sigma)^2 = 3.022377590477805206$  (30,20) ode time =4.1732 other time =0.28

```
In [47]: epsilonb = 0.01

ode_decimal_precision = 30
j_list = [3/2,2,5/2,3,7/2]+[m/2 for m in range(12,32,5)]+[m/2 for m in range(32,122,10)]
process_j_list()

j_list = [m/2 for m in range(122,182,20)]
process_j_list()

ode_decimal_precision = 40
j_list = [m/2 for m in range(182,342,20)]
process_j_list()

ode_decimal_precision = 50
j_list = [m/2 for m in range(342,502,40)]
process_j_list()

ode_decimal_precision = 60
j_list = [m/2 for m in range(500,660,80)]
process_j_list()

ode_decimal_precision = 80
j_list = [m/2 for m in range(660,820,80)]
process_j_list()
```

|                   |                    |                   |                                             |         |                  |               |
|-------------------|--------------------|-------------------|---------------------------------------------|---------|------------------|---------------|
| $\epsilon = 0.01$ | $j = \frac{3}{2}$  | $\sigma = 0.0150$ | $(\omega/\sigma)^2 = 3.2672043864311006399$ | (30,20) | ode time =4.1767 | other time =0 |
| $\epsilon = 0.01$ | $j = 2$            | $\sigma = 0.0200$ | $(\omega/\sigma)^2 = 3.2654202519516805471$ | (30,20) | ode time =4.1784 | other time =0 |
| $\epsilon = 0.01$ | $j = \frac{5}{2}$  | $\sigma = 0.0250$ | $(\omega/\sigma)^2 = 3.263148361992893767$  | (30,20) | ode time =4.1756 | other time =0 |
| $\epsilon = 0.01$ | $j = 3$            | $\sigma = 0.0300$ | $(\omega/\sigma)^2 = 3.2604047479759726416$ | (30,20) | ode time =4.1721 | other time =0 |
| $\epsilon = 0.01$ | $j = \frac{7}{2}$  | $\sigma = 0.0350$ | $(\omega/\sigma)^2 = 3.2572085030256455228$ | (30,20) | ode time =4.1723 | other time =0 |
| $\epsilon = 0.01$ | $j = 6$            | $\sigma = 0.0600$ | $(\omega/\sigma)^2 = 3.2352832046354860316$ | (30,20) | ode time =4.1708 | other time =0 |
| $\epsilon = 0.01$ | $j = \frac{17}{2}$ | $\sigma = 0.0850$ | $(\omega/\sigma)^2 = 3.206121949782006774$  | (30,20) | ode time =4.1733 | other time =0 |
| $\epsilon = 0.01$ | $j = 11$           | $\sigma = 0.110$  | $(\omega/\sigma)^2 = 3.1736417351061720374$ | (30,20) | ode time =4.1783 | other time =0 |
| $\epsilon = 0.01$ | $j = \frac{27}{2}$ | $\sigma = 0.135$  | $(\omega/\sigma)^2 = 3.1414236275692625523$ | (30,20) | ode time =4.1814 | other time =0 |
| $\epsilon = 0.01$ | $j = 16$           | $\sigma = 0.160$  | $(\omega/\sigma)^2 = 3.1122487572175275056$ | (30,20) | ode time =4.1751 | other time =0 |
| $\epsilon = 0.01$ | $j = 21$           | $\sigma = 0.210$  | $(\omega/\sigma)^2 = 3.0696875586792866563$ | (30,20) | ode time =4.1778 | other time =0 |
| $\epsilon = 0.01$ | $j = 26$           | $\sigma = 0.260$  | $(\omega/\sigma)^2 = 3.0521943360032247625$ | (30,20) | ode time =4.1736 | other time =0 |
| $\epsilon = 0.01$ | $j = 31$           | $\sigma = 0.310$  | $(\omega/\sigma)^2 = 3.0584974343907985133$ | (30,20) | ode time =4.1752 | other time =0 |

|                   |           |                  |                                             |         |                  |                 |
|-------------------|-----------|------------------|---------------------------------------------|---------|------------------|-----------------|
| $\epsilon = 0.01$ | $j = 36$  | $\sigma = 0.360$ | $(\omega/\sigma)^2 = 3.084063345537294108$  | (30,20) | ode time =4.1753 | other time =0.2 |
| $\epsilon = 0.01$ | $j = 41$  | $\sigma = 0.410$ | $(\omega/\sigma)^2 = 3.1235085639426417268$ | (30,20) | ode time =4.1712 | other time =0   |
| $\epsilon = 0.01$ | $j = 46$  | $\sigma = 0.460$ | $(\omega/\sigma)^2 = 3.1717877497744656857$ | (30,20) | ode time =4.1730 | other time =0   |
| $\epsilon = 0.01$ | $j = 51$  | $\sigma = 0.510$ | $(\omega/\sigma)^2 = 3.2247105184655556095$ | (30,20) | ode time =4.1740 | other time =0   |
| $\epsilon = 0.01$ | $j = 56$  | $\sigma = 0.560$ | $(\omega/\sigma)^2 = 3.2790876124698933971$ | (30,20) | ode time =4.1738 | other time =0   |
| $\epsilon = 0.01$ | $j = 61$  | $\sigma = 0.610$ | $(\omega/\sigma)^2 = 3.3326732310851522941$ | (30,20) | ode time =4.1720 | other time =0   |
| $\epsilon = 0.01$ | $j = 71$  | $\sigma = 0.710$ | $(\omega/\sigma)^2 = 3.4322462691108951995$ | (30,20) | ode time =4.1708 | other time =0   |
| $\epsilon = 0.01$ | $j = 81$  | $\sigma = 0.810$ | $(\omega/\sigma)^2 = 3.5180450475770610144$ | (30,20) | ode time =4.1753 | other time =0   |
| $\epsilon = 0.01$ | $j = 91$  | $\sigma = 0.910$ | $(\omega/\sigma)^2 = 3.5896614240309616849$ | (40,20) | ode time =11.596 | other time =0   |
| $\epsilon = 0.01$ | $j = 101$ | $\sigma = 1.01$  | $(\omega/\sigma)^2 = 3.6486648274752725845$ | (40,20) | ode time =11.601 | other time =0   |
| $\epsilon = 0.01$ | $j = 111$ | $\sigma = 1.11$  | $(\omega/\sigma)^2 = 3.6971296260447738647$ | (40,20) | ode time =11.588 | other time =0.  |
| $\epsilon = 0.01$ | $j = 121$ | $\sigma = 1.21$  | $(\omega/\sigma)^2 = 3.7370310384526100958$ | (40,20) | ode time =11.585 | other time =0   |
| $\epsilon = 0.01$ | $j = 131$ | $\sigma = 1.31$  | $(\omega/\sigma)^2 = 3.7700511363266407975$ | (40,20) | ode time =11.586 | other time =0   |
| $\epsilon = 0.01$ | $j = 141$ | $\sigma = 1.41$  | $(\omega/\sigma)^2 = 3.7975548447115829331$ | (40,20) | ode time =11.595 | other time =0   |
| $\epsilon = 0.01$ | $j = 151$ | $\sigma = 1.51$  | $(\omega/\sigma)^2 = 3.820626139695773359$  | (40,20) | ode time =11.589 | other time =0.7 |
| $\epsilon = 0.01$ | $j = 161$ | $\sigma = 1.61$  | $(\omega/\sigma)^2 = 3.8401187078847102487$ | (40,20) | ode time =11.588 | other time =0   |
| $\epsilon = 0.01$ | $j = 171$ | $\sigma = 1.71$  | $(\omega/\sigma)^2 = 3.8567039682251523216$ | (50,20) | ode time =27.688 | other time =1   |
| $\epsilon = 0.01$ | $j = 191$ | $\sigma = 1.91$  | $(\omega/\sigma)^2 = 3.8831601923182423238$ | (50,20) | ode time =27.697 | other time =1   |
| $\epsilon = 0.01$ | $j = 211$ | $\sigma = 2.11$  | $(\omega/\sigma)^2 = 3.9030531012025266795$ | (50,20) | ode time =27.699 | other time =1   |
| $\epsilon = 0.01$ | $j = 231$ | $\sigma = 2.31$  | $(\omega/\sigma)^2 = 3.9183462616756493358$ | (50,20) | ode time =27.693 | other time =1   |

---

$\epsilon = 0.01$   $j = 250$   $\sigma = 2.50$   $(\omega/\sigma)^2 = 3.929798561076493345$  (60,20) ode time =57.953 other time =4.2

---

$\epsilon = 0.01$   $j = 290$   $\sigma = 2.90$   $(\omega/\sigma)^2 = 3.9472798590403610717$  (60,20) ode time =57.990 other time =4

---

$\epsilon = 0.01$   $j = 330$   $\sigma = 3.30$   $(\omega/\sigma)^2 = 3.9590035760635018684$  (80,20) ode time =190.91 other time =1

---

$\epsilon = 0.01$   $j = 370$   $\sigma = 3.70$   $(\omega/\sigma)^2 = 3.9672316604535058991$  (80,20) ode time =190.33 other time =1

---

$j \rightarrow \infty$

In [48]:

```
ode_decimal_precision = 30
sigma_list = [0.02,0.04,.06,.08,.10,0.15,0.2,0.25,0.3,0.35,0.4,0.45,0.5,0.55,.6,0.65,0.7,0.75,0.8,0.9]
process_sigma_list()

ode_decimal_precision = 40
sigma_list = [0.95,1,1.15,1.3,1.45,1.6]
process_sigma_list()

ode_decimal_precision = 50
sigma_list = [1.85,2.1]
process_sigma_list()

ode_decimal_precision = 60
sigma_list = [2.35,2.65,3.0]
process_sigma_list()

ode_decimal_precision = 70
sigma_list = [3.35,3.7]
process_sigma_list()

ode_decimal_precision = 80
sigma_list = [4.0]
process_sigma_list()
```

---

$\epsilon = 0.$   $j = +\infty$   $\sigma = 0.0200$   $(\omega/\sigma)^2 = 3.2668296476156010782$  (30,20) ode time =4.1716 other time =0.

---

$\epsilon = 0.$   $j = +\infty$   $\sigma = 0.0400$   $(\omega/\sigma)^2 = 3.2549624194185527516$  (30,20) ode time =4.1589 other time =0.

---

$\epsilon = 0.$   $j = +\infty$   $\sigma = 0.0600$   $(\omega/\sigma)^2 = 3.2366200733195958741$  (30,20) ode time =4.1549 other time =0.

---

$\epsilon = 0.$   $j = +\infty$   $\sigma = 0.0800$   $(\omega/\sigma)^2 = 3.2136259717282729338$  (30,20) ode time =4.1632 other time =0.

---

$\epsilon = 0.$   $j = +\infty$   $\sigma = 0.100$   $(\omega/\sigma)^2 = 3.1880069613841409911$  (30,20) ode time =4.1581 other time =0.2

---

$\epsilon = 0.$   $j = +\infty$   $\sigma = 0.150$   $(\omega/\sigma)^2 = 3.1244685863857124095$  (30,20) ode time =4.1562 other time =0.2

---

$\epsilon = 0.$   $j = +\infty$   $\sigma = 0.200$   $(\omega/\sigma)^2 = 3.0771560571495292472$  (30,20) ode time =4.1551 other time =0.2

---

$\epsilon = 0.$   $j = +\infty$   $\sigma = 0.250$   $(\omega/\sigma)^2 = 3.0544570413357088867$  (30,20) ode time =4.1496 other time =0.2

---

$\epsilon = 0.$   $j = +\infty$   $\sigma = 0.300$   $(\omega/\sigma)^2 = 3.0561983284001380199$  (30,20) ode time =4.1643 other time =0.2

---

|                 |               |                  |                                             |         |                  |                  |
|-----------------|---------------|------------------|---------------------------------------------|---------|------------------|------------------|
| $\epsilon = 0.$ | $j = +\infty$ | $\sigma = 0.350$ | $(\omega/\sigma)^2 = 3.0782494102199292586$ | (30,20) | ode time =4.1518 | other time =0.2  |
| $\epsilon = 0.$ | $j = +\infty$ | $\sigma = 0.400$ | $(\omega/\sigma)^2 = 3.115268631675504591$  | (30,20) | ode time =4.1571 | other time =0.28 |
| $\epsilon = 0.$ | $j = +\infty$ | $\sigma = 0.450$ | $(\omega/\sigma)^2 = 3.1620831000589164024$ | (30,20) | ode time =4.1531 | other time =0.2  |
| $\epsilon = 0.$ | $j = +\infty$ | $\sigma = 0.500$ | $(\omega/\sigma)^2 = 3.2143090210928620561$ | (30,20) | ode time =4.1573 | other time =0.2  |
| $\epsilon = 0.$ | $j = +\infty$ | $\sigma = 0.550$ | $(\omega/\sigma)^2 = 3.2685555230236133845$ | (30,20) | ode time =4.1517 | other time =0.2  |
| $\epsilon = 0.$ | $j = +\infty$ | $\sigma = 0.600$ | $(\omega/\sigma)^2 = 3.322397590023560884$  | (30,20) | ode time =4.1528 | other time =0.28 |
| $\epsilon = 0.$ | $j = +\infty$ | $\sigma = 0.650$ | $(\omega/\sigma)^2 = 3.3742337839221701029$ | (30,20) | ode time =4.1558 | other time =0.2  |
| $\epsilon = 0.$ | $j = +\infty$ | $\sigma = 0.700$ | $(\omega/\sigma)^2 = 3.4231048786692838874$ | (30,20) | ode time =4.1519 | other time =0.2  |
| $\epsilon = 0.$ | $j = +\infty$ | $\sigma = 0.750$ | $(\omega/\sigma)^2 = 3.4685188101731642574$ | (30,20) | ode time =4.1529 | other time =0.2  |
| $\epsilon = 0.$ | $j = +\infty$ | $\sigma = 0.800$ | $(\omega/\sigma)^2 = 3.5103035433550040559$ | (30,20) | ode time =4.1540 | other time =0.2  |
| $\epsilon = 0.$ | $j = +\infty$ | $\sigma = 0.850$ | $(\omega/\sigma)^2 = 3.5484937597379243632$ | (30,20) | ode time =4.1566 | other time =0.2  |
| $\epsilon = 0.$ | $j = +\infty$ | $\sigma = 0.900$ | $(\omega/\sigma)^2 = 3.5832488584938412583$ | (30,20) | ode time =4.1546 | other time =0.2  |
| $\epsilon = 0.$ | $j = +\infty$ | $\sigma = 0.950$ | $(\omega/\sigma)^2 = 3.614796434544753421$  | (40,20) | ode time =11.568 | other time =0.78 |
| $\epsilon = 0.$ | $j = +\infty$ | $\sigma = 1.00$  | $(\omega/\sigma)^2 = 3.6433949315513066236$ | (40,20) | ode time =11.550 | other time =0.77 |
| $\epsilon = 0.$ | $j = +\infty$ | $\sigma = 1.15$  | $(\omega/\sigma)^2 = 3.7141090034650305173$ | (40,20) | ode time =11.561 | other time =0.77 |
| $\epsilon = 0.$ | $j = +\infty$ | $\sigma = 1.30$  | $(\omega/\sigma)^2 = 3.7670902207074880688$ | (40,20) | ode time =11.556 | other time =0.78 |
| $\epsilon = 0.$ | $j = +\infty$ | $\sigma = 1.45$  | $(\omega/\sigma)^2 = 3.8073212784009466351$ | (40,20) | ode time =11.559 | other time =0.77 |
| $\epsilon = 0.$ | $j = +\infty$ | $\sigma = 1.60$  | $(\omega/\sigma)^2 = 3.8383580870573511167$ | (40,20) | ode time =11.565 | other time =0.78 |
| $\epsilon = 0.$ | $j = +\infty$ | $\sigma = 1.85$  | $(\omega/\sigma)^2 = 3.8760613017121425409$ | (50,20) | ode time =27.643 | other time =1.92 |
| $\epsilon = 0.$ | $j = +\infty$ | $\sigma = 2.10$  | $(\omega/\sigma)^2 = 3.9022085114187509892$ | (50,20) | ode time =27.642 | other time =1.92 |



$\epsilon = 0.$   $j = +\infty$   $\sigma = 2.35$   $(\omega/\sigma)^2 = 3.920997493443859379$  (60,20) ode time =57.962 other time =4.229

$\epsilon = 0.$   $j = +\infty$   $\sigma = 2.65$   $(\omega/\sigma)^2 = 3.9372577317750071412$  (60,20) ode time =57.927 other time =4.24

$\epsilon = 0.$   $j = +\infty$   $\sigma = 3.00$   $(\omega/\sigma)^2 = 3.9506514252909105507$  (60,20) ode time =57.910 other time =4.23

$\epsilon = 0.$   $j = +\infty$   $\sigma = 3.35$   $(\omega/\sigma)^2 = 3.9602013952518077806$  (70,20) ode time =106.41 other time =8.17

$\epsilon = 0.$   $j = +\infty$   $\sigma = 3.70$   $(\omega/\sigma)^2 = 3.9672405307184597691$  (70,20) ode time =106.42 other time =8.09

$\epsilon = 0.$   $j = +\infty$   $\sigma = 4.00$   $(\omega/\sigma)^2 = 3.9718944720574996035$  (80,20) ode time =190.40 other time =14.5

## Ode 1<sub>j</sub>

In [49]:

```
ode_name='1j'  
data[ode_name]={}  
data[ode_name]['asympt']={}  
data[ode_name]['finite']={}
```

## j finite

In [50]:

```
data['1j']['finite']={}
```

In [51]:

```
epsilonb = 0.7071  
  
ode_decimal_precision = 40  
j_list = [3/2]  
process_j_list()  
  
ode_decimal_precision = 40  
j_list = [2,5/2]  
process_j_list()  
  
ode_decimal_precision = 50  
j_list = [3,7/2,4]  
process_j_list()
```

$\epsilon = 0.7071$   $j = \frac{3}{2}$   $\sigma = 1.06$   $(\omega/\sigma)^2 = 4.4444480978367223919$  (40,20) ode time =2.5378 other time =

$\epsilon = 0.7071$   $j = 2$   $\sigma = 1.41$   $(\omega/\sigma)^2 = 4.2500021920368275213$  (40,20) ode time =2.5364 other time =0

$\epsilon = 0.7071$   $j = \frac{5}{2}$   $\sigma = 1.77$   $(\omega/\sigma)^2 = 4.1600014475720327977$  (40,20) ode time =2.5336 other time =

$\epsilon = 0.7071$   $j = 3$   $\sigma = 2.12$   $(\omega/\sigma)^2 = 4.1111121340622449649$  (50,20) ode time =6.0651 other time =1.

$\epsilon = 0.7071$   $j = \frac{7}{2}$   $\sigma = 2.47$   $(\omega/\sigma)^2 = 4.0816334126785126723$  (50,20) ode time =6.0601 other time =

$\epsilon = 0.7071$   $j = 4$   $\sigma = 2.83$   $(\omega/\sigma)^2 = 4.0625005856591875058$  (50,20) ode time =6.0614 other time =1

In [52]:

```
epsilonb = 0.5

ode_decimal_precision = 30
j_list = [3/2]
process_j_list()

ode_decimal_precision = 40
j_list = [2,5/2,3,7/2]
process_j_list()
```

$\epsilon = 0.5$   $j = \frac{3}{2}$   $\sigma = 0.750$   $(\omega/\sigma)^2 = 4.6133268717304487007$  (30,20) ode time =2.6206 other time =0.2

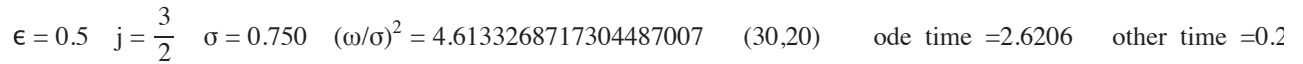

$\epsilon = 0.5$   $j = 2$   $\sigma = 1.00$   $(\omega/\sigma)^2 = 4.3542164025695802042$  (40,20) ode time =7.6163 other time =0.613

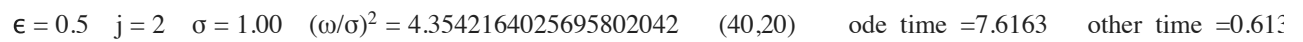

$\epsilon = 0.5$   $j = \frac{5}{2}$   $\sigma = 1.25$   $(\omega/\sigma)^2 = 4.2299812085082966298$  (40,20) ode time =7.6104 other time =0.61

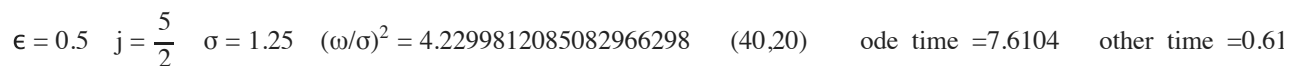

$\epsilon = 0.5$   $j = 3$   $\sigma = 1.50$   $(\omega/\sigma)^2 = 4.1610829215236342351$  (40,20) ode time =7.6011 other time =0.611

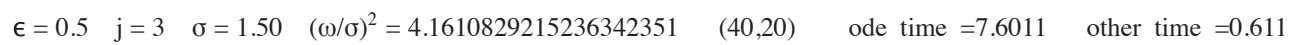

$\epsilon = 0.5$   $j = \frac{7}{2}$   $\sigma = 1.75$   $(\omega/\sigma)^2 = 4.1189953689480166178$  (40,20) ode time =7.6033 other time =0.61

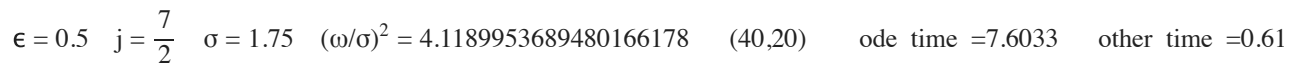

In [53]:

```
epsilonb = 0.35

ode_decimal_precision = 30
j_list = [3/2,2,5/2]
process_j_list()

ode_decimal_precision = 40
j_list = [3,7/2]
process_j_list()
```

$\epsilon = 0.35$   $j = \frac{3}{2}$   $\sigma = 0.525$   $(\omega/\sigma)^2 = 4.8909684915731806421$  (30,20) ode time =2.7455 other time =0

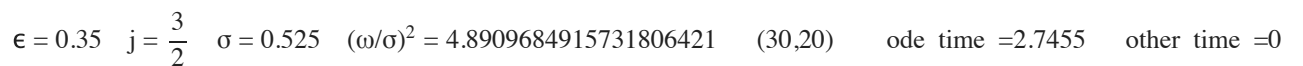

$\epsilon = 0.35$   $j = 2$   $\sigma = 0.700$   $(\omega/\sigma)^2 = 4.5358855153537569218$  (30,20) ode time =3.0874 other time =0.2

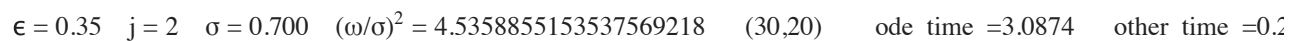

$\epsilon = 0.35$   $j = \frac{5}{2}$   $\sigma = 0.875$   $(\omega/\sigma)^2 = 4.356661399443839756$  (30,20) ode time =3.0889 other time =0.2

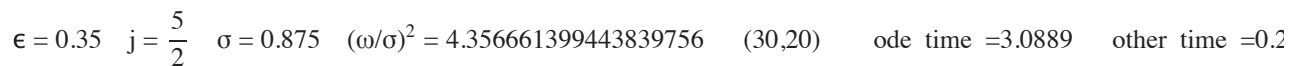

$\epsilon = 0.35$   $j = 3$   $\sigma = 1.05$   $(\omega/\sigma)^2 = 4.2538454972933859456$  (40,20) ode time =8.9799 other time =0.64

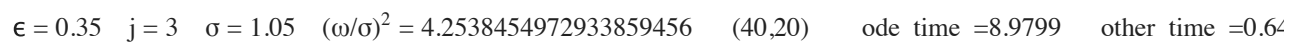

$\epsilon = 0.35$   $j = \frac{7}{2}$   $\sigma = 1.22$   $(\omega/\sigma)^2 = 4.1895656797028750557$  (40,20) ode time =8.9825 other time =0.6

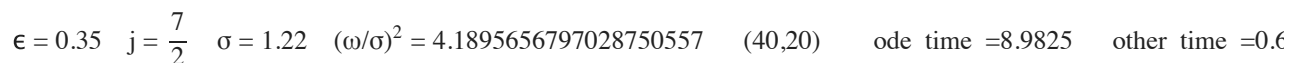

In [54]:

```
epsilonb = 0.25

ode_decimal_precision = 30
j_list = [3/2,2,5/2,3,7/2]
process_j_list()
```

$\epsilon = 0.25$   $j = \frac{3}{2}$   $\sigma = 0.375$   $(\omega/\sigma)^2 = 5.2882102889748398006$  (30,20) ode time =3.1448 other time =0

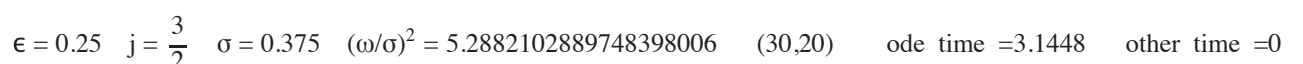

---

$\epsilon = 0.25$   $j = 2$   $\sigma = 0.500$   $(\omega/\sigma)^2 = 4.8130021114066852972$  (30,20) ode time =3.1451 other time =0.2

---

$\epsilon = 0.25$   $j = \frac{5}{2}$   $\sigma = 0.625$   $(\omega/\sigma)^2 = 4.5586215534658206707$  (30,20) ode time =3.1446 other time =0

---

$\epsilon = 0.25$   $j = 3$   $\sigma = 0.750$   $(\omega/\sigma)^2 = 4.406506287046373958$  (30,20) ode time =3.1437 other time =0.21

---

$\epsilon = 0.25$   $j = \frac{7}{2}$   $\sigma = 0.875$   $(\omega/\sigma)^2 = 4.3084606397713180209$  (30,20) ode time =3.1405 other time =0

---

In [55]:

```
epsilonb = 0.15  
  
ode_decimal_precision = 30  
j_list = [3/2, 2, 5/2, 3, 7/2, 4]  
process_j_list()
```

$\epsilon = 0.15$   $j = \frac{3}{2}$   $\sigma = 0.225$   $(\omega/\sigma)^2 = 6.1901268599450224521$  (30,20) ode time =3.1731 other time =0

---

$\epsilon = 0.15$   $j = 2$   $\sigma = 0.300$   $(\omega/\sigma)^2 = 5.5073555959279322088$  (30,20) ode time =3.1742 other time =0.2

---

$\epsilon = 0.15$   $j = \frac{5}{2}$   $\sigma = 0.375$   $(\omega/\sigma)^2 = 5.0997668285842154872$  (30,20) ode time =3.1732 other time =0

---

$\epsilon = 0.15$   $j = 3$   $\sigma = 0.450$   $(\omega/\sigma)^2 = 4.8363596374252251442$  (30,20) ode time =3.1694 other time =0.2

---

$\epsilon = 0.15$   $j = \frac{7}{2}$   $\sigma = 0.525$   $(\omega/\sigma)^2 = 4.6563688999228258291$  (30,20) ode time =3.1696 other time =0

---

$\epsilon = 0.15$   $j = 4$   $\sigma = 0.600$   $(\omega/\sigma)^2 = 4.5280529556201950957$  (30,20) ode time =3.1775 other time =0.2

---

In [56]:

```
epsilonb = 0.01  
  
ode_decimal_precision = 30  
j_list = [3/2, 2, 5/2, 3, 7/2] + [m/2 for m in range(12, 32, 5)] + [m/2 for m in range(32, 122, 10)]  
process_j_list()  
  
j_list = [m/2 for m in range(122, 182, 20)]  
process_j_list()  
  
ode_decimal_precision = 40  
j_list = [m/2 for m in range(182, 342, 20)]  
process_j_list()  
  
ode_decimal_precision = 50  
j_list = [m/2 for m in range(342, 502, 40)]  
process_j_list()  
  
ode_decimal_precision = 60  
j_list = [m/2 for m in range(500, 660, 80)]  
process_j_list()
```

$\epsilon = 0.01$   $j = \frac{3}{2}$   $\sigma = 0.0150$   $(\omega/\sigma)^2 = 9.4738902559517118445$  (30,20) ode time =2.8419 other time =

---

|                                                                                      |                    |                   |                                             |         |                  |                  |
|--------------------------------------------------------------------------------------|--------------------|-------------------|---------------------------------------------|---------|------------------|------------------|
| $\epsilon = 0.01$                                                                    | $j = 2$            | $\sigma = 0.0200$ | $(\omega/\sigma)^2 = 9.2413505144763454294$ | (30,20) | ode time =2.8459 | other time =0    |
| 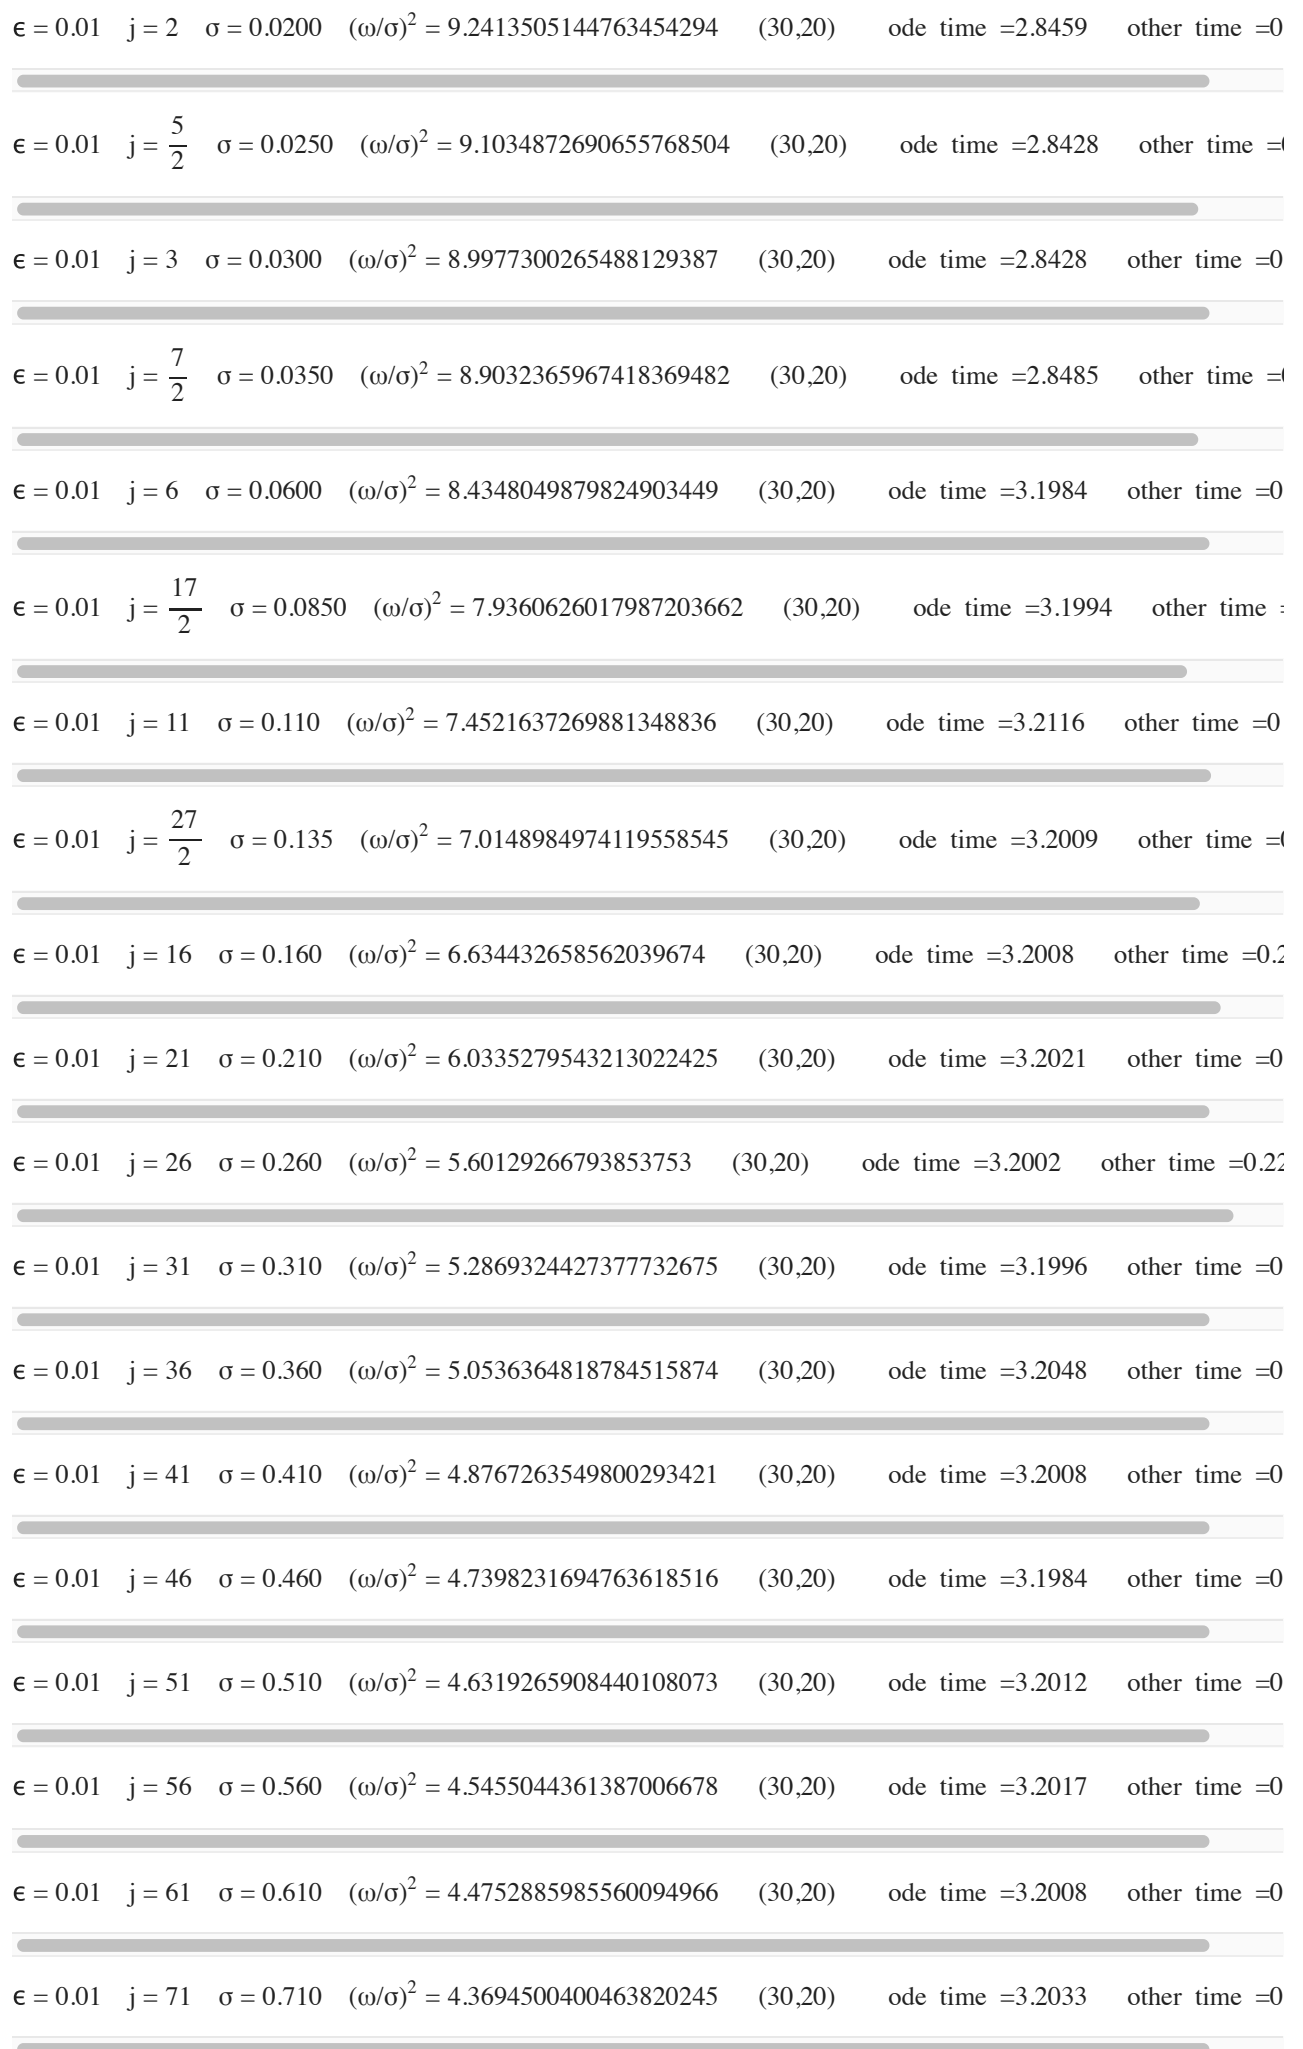   |                    |                   |                                             |         |                  |                  |
| $\epsilon = 0.01$                                                                    | $j = \frac{5}{2}$  | $\sigma = 0.0250$ | $(\omega/\sigma)^2 = 9.1034872690655768504$ | (30,20) | ode time =2.8428 | other time =0    |
| 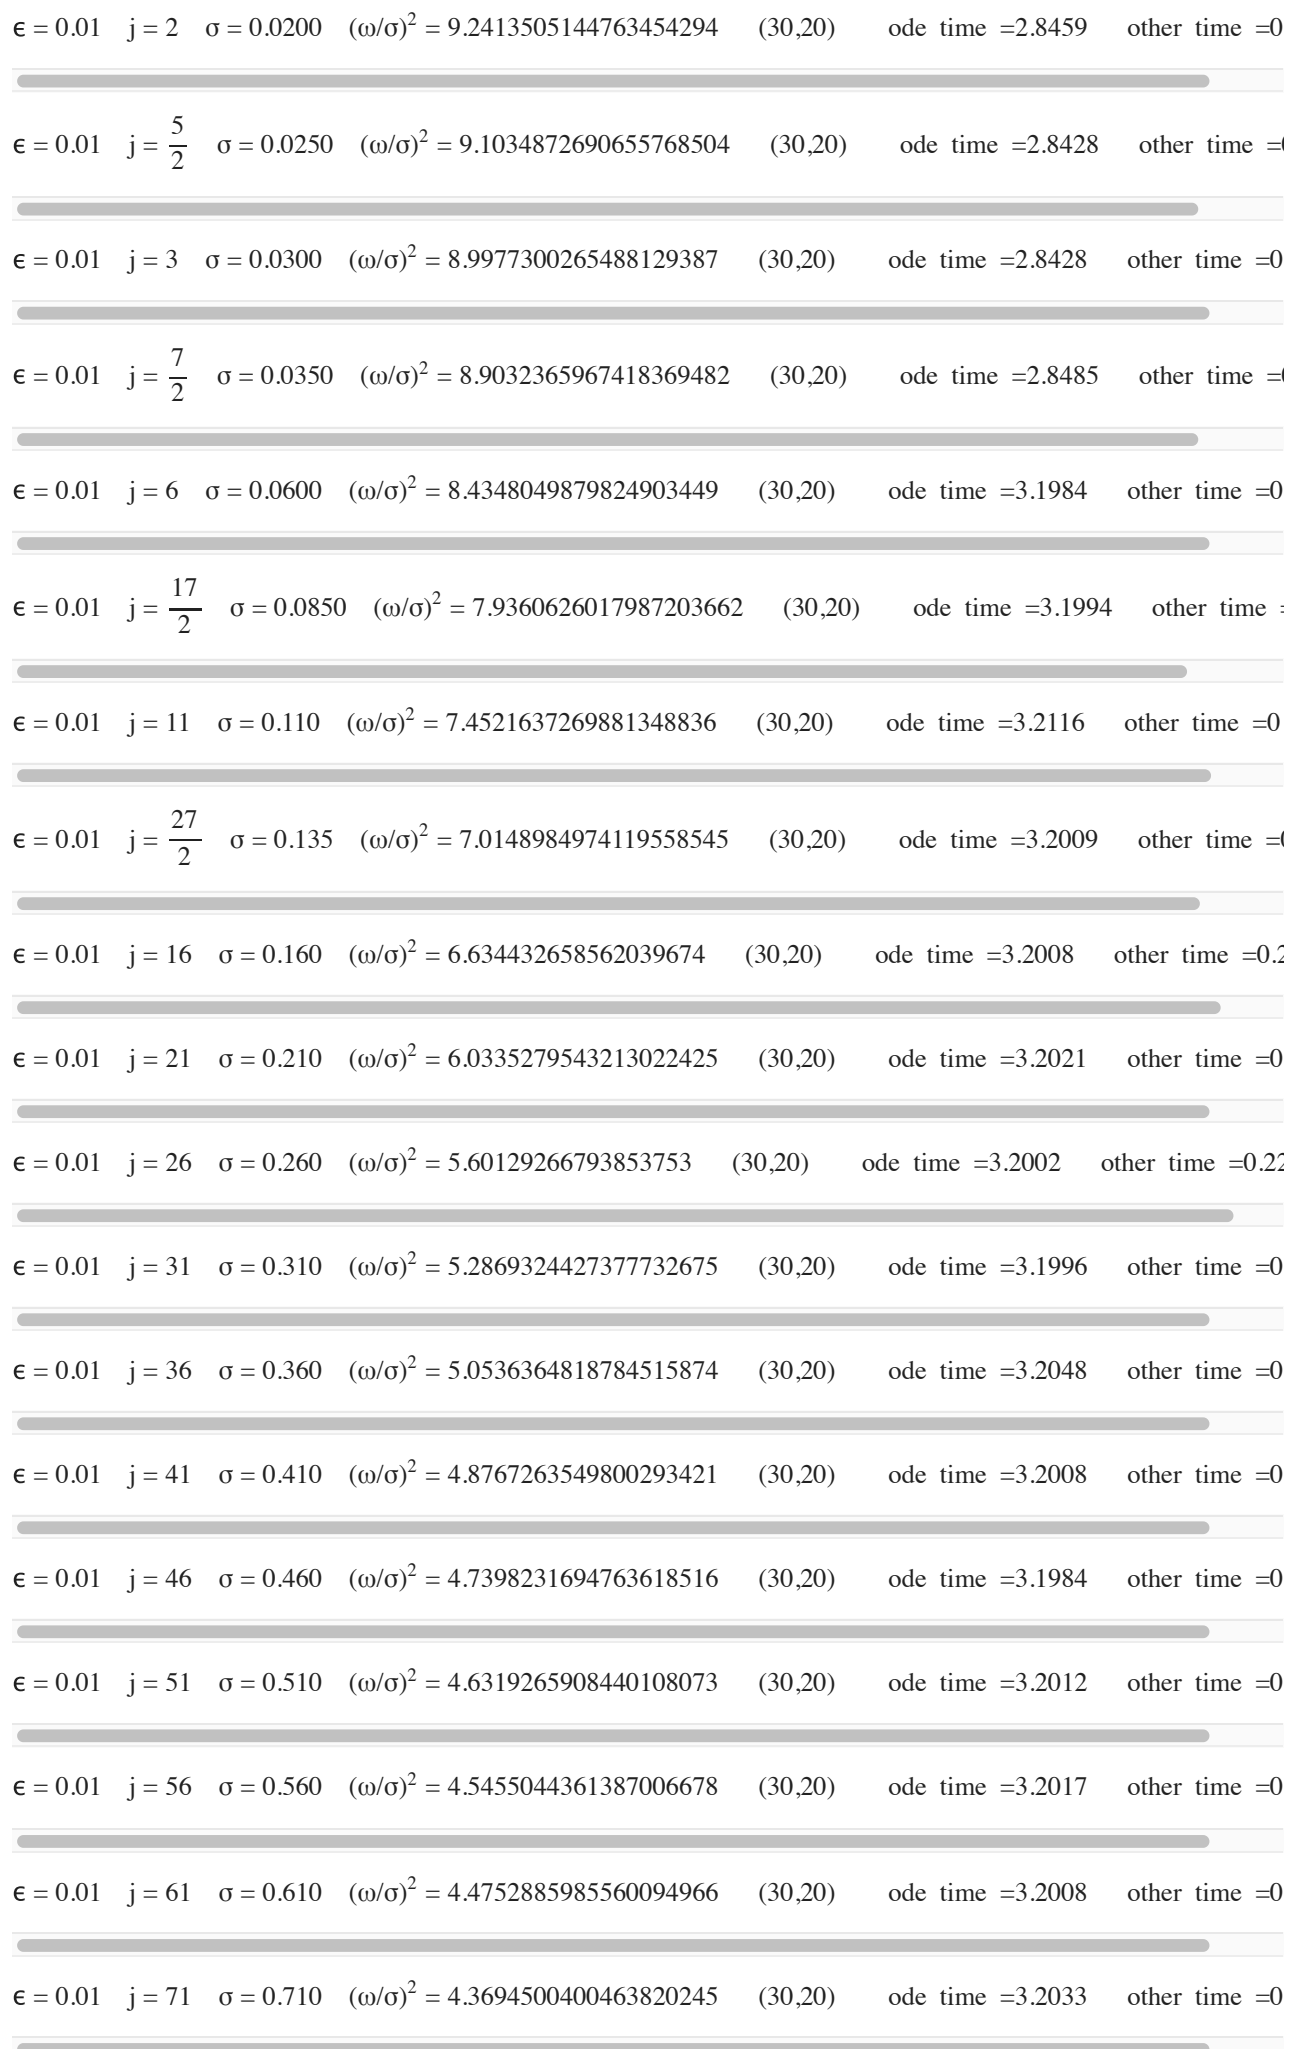   |                    |                   |                                             |         |                  |                  |
| $\epsilon = 0.01$                                                                    | $j = 3$            | $\sigma = 0.0300$ | $(\omega/\sigma)^2 = 8.9977300265488129387$ | (30,20) | ode time =2.8428 | other time =0    |
| 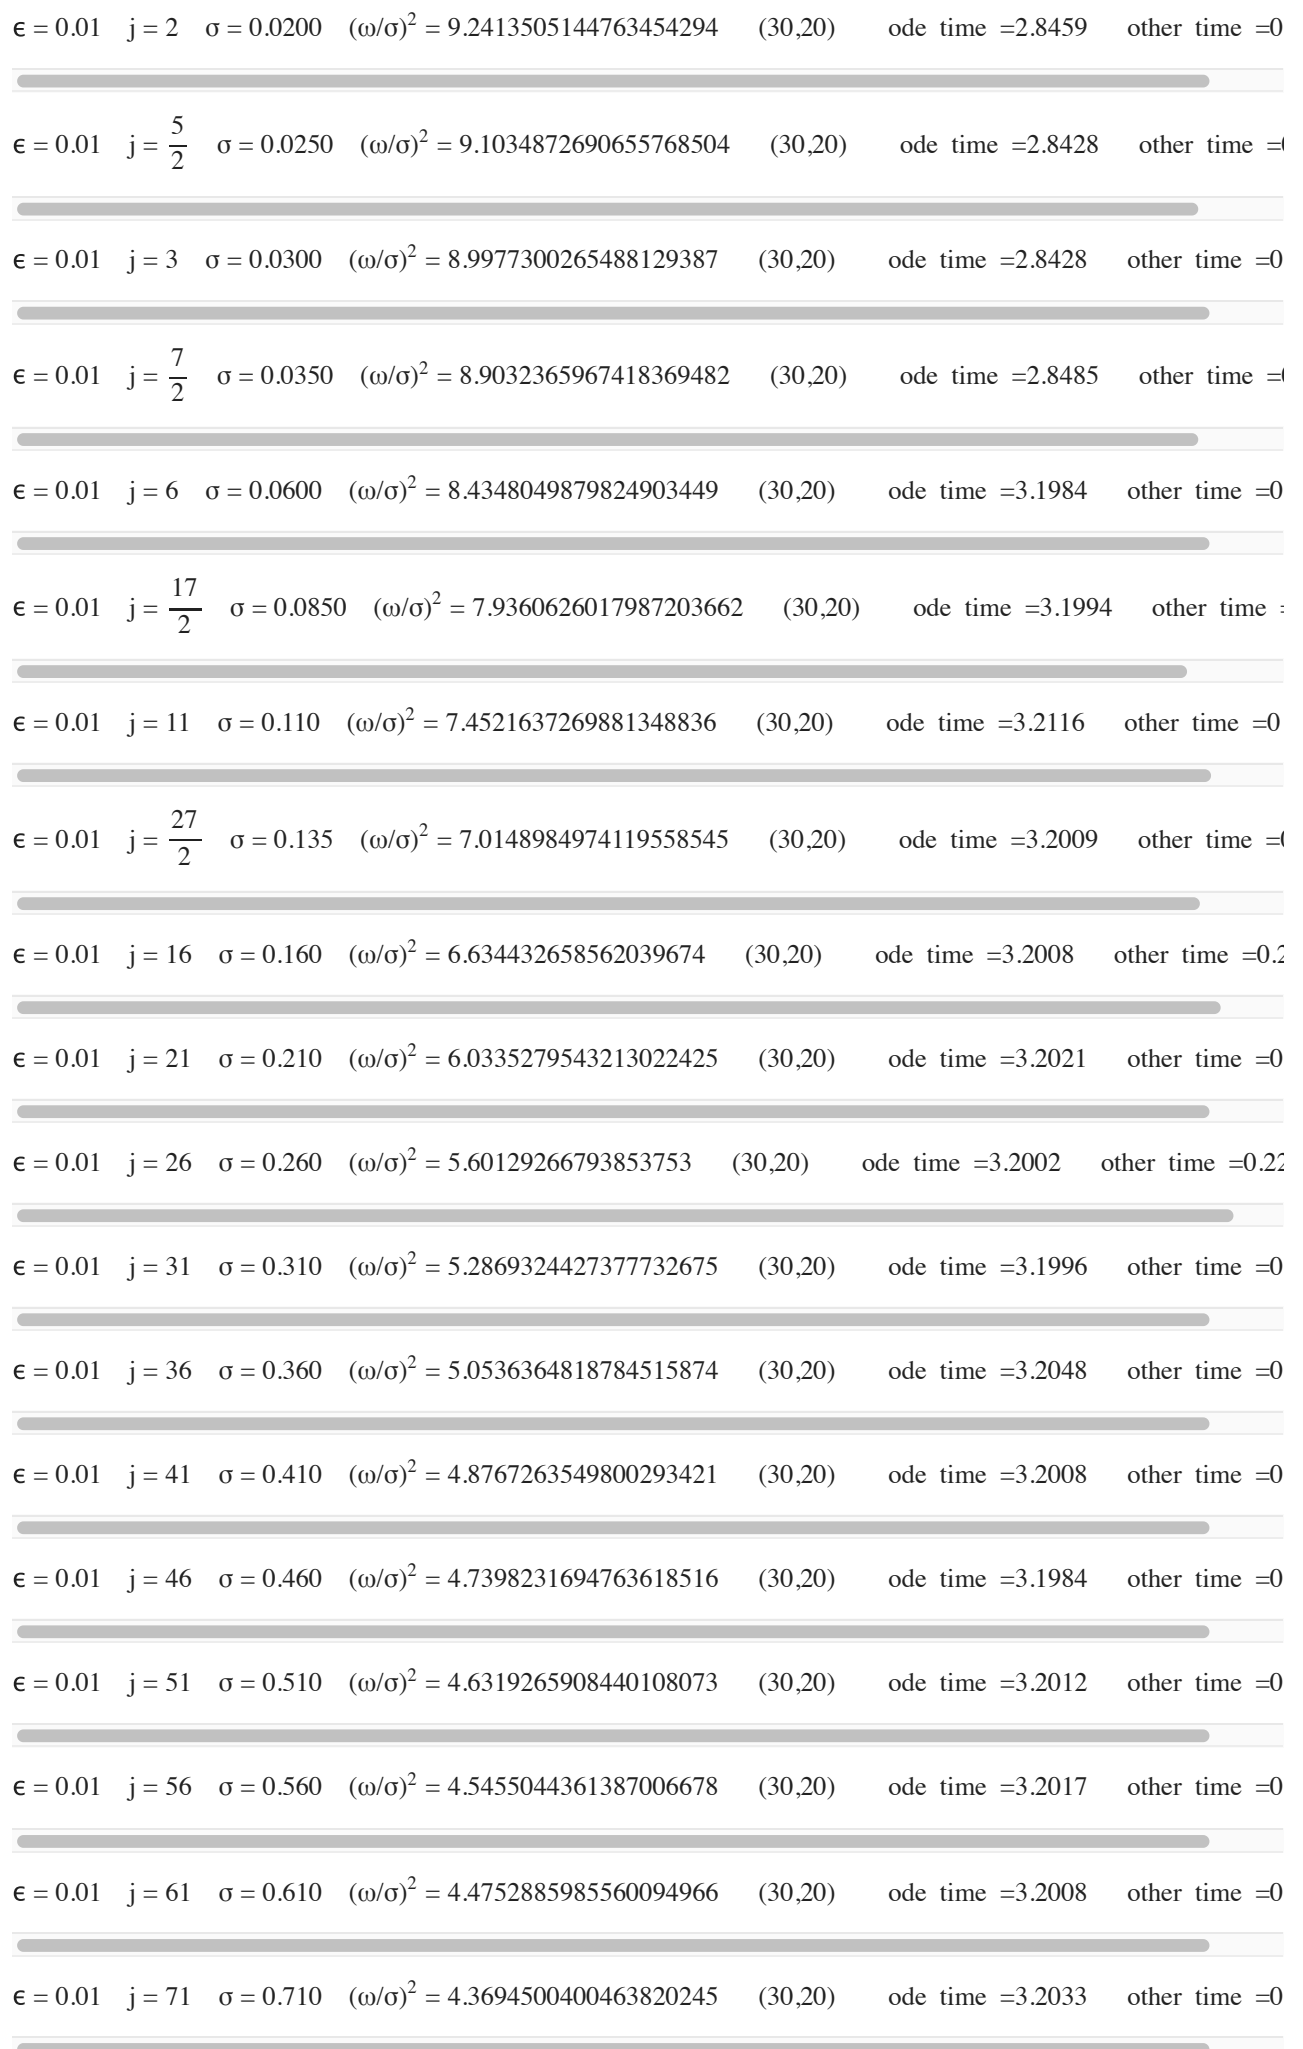   |                    |                   |                                             |         |                  |                  |
| $\epsilon = 0.01$                                                                    | $j = \frac{7}{2}$  | $\sigma = 0.0350$ | $(\omega/\sigma)^2 = 8.9032365967418369482$ | (30,20) | ode time =2.8485 | other time =0    |
| 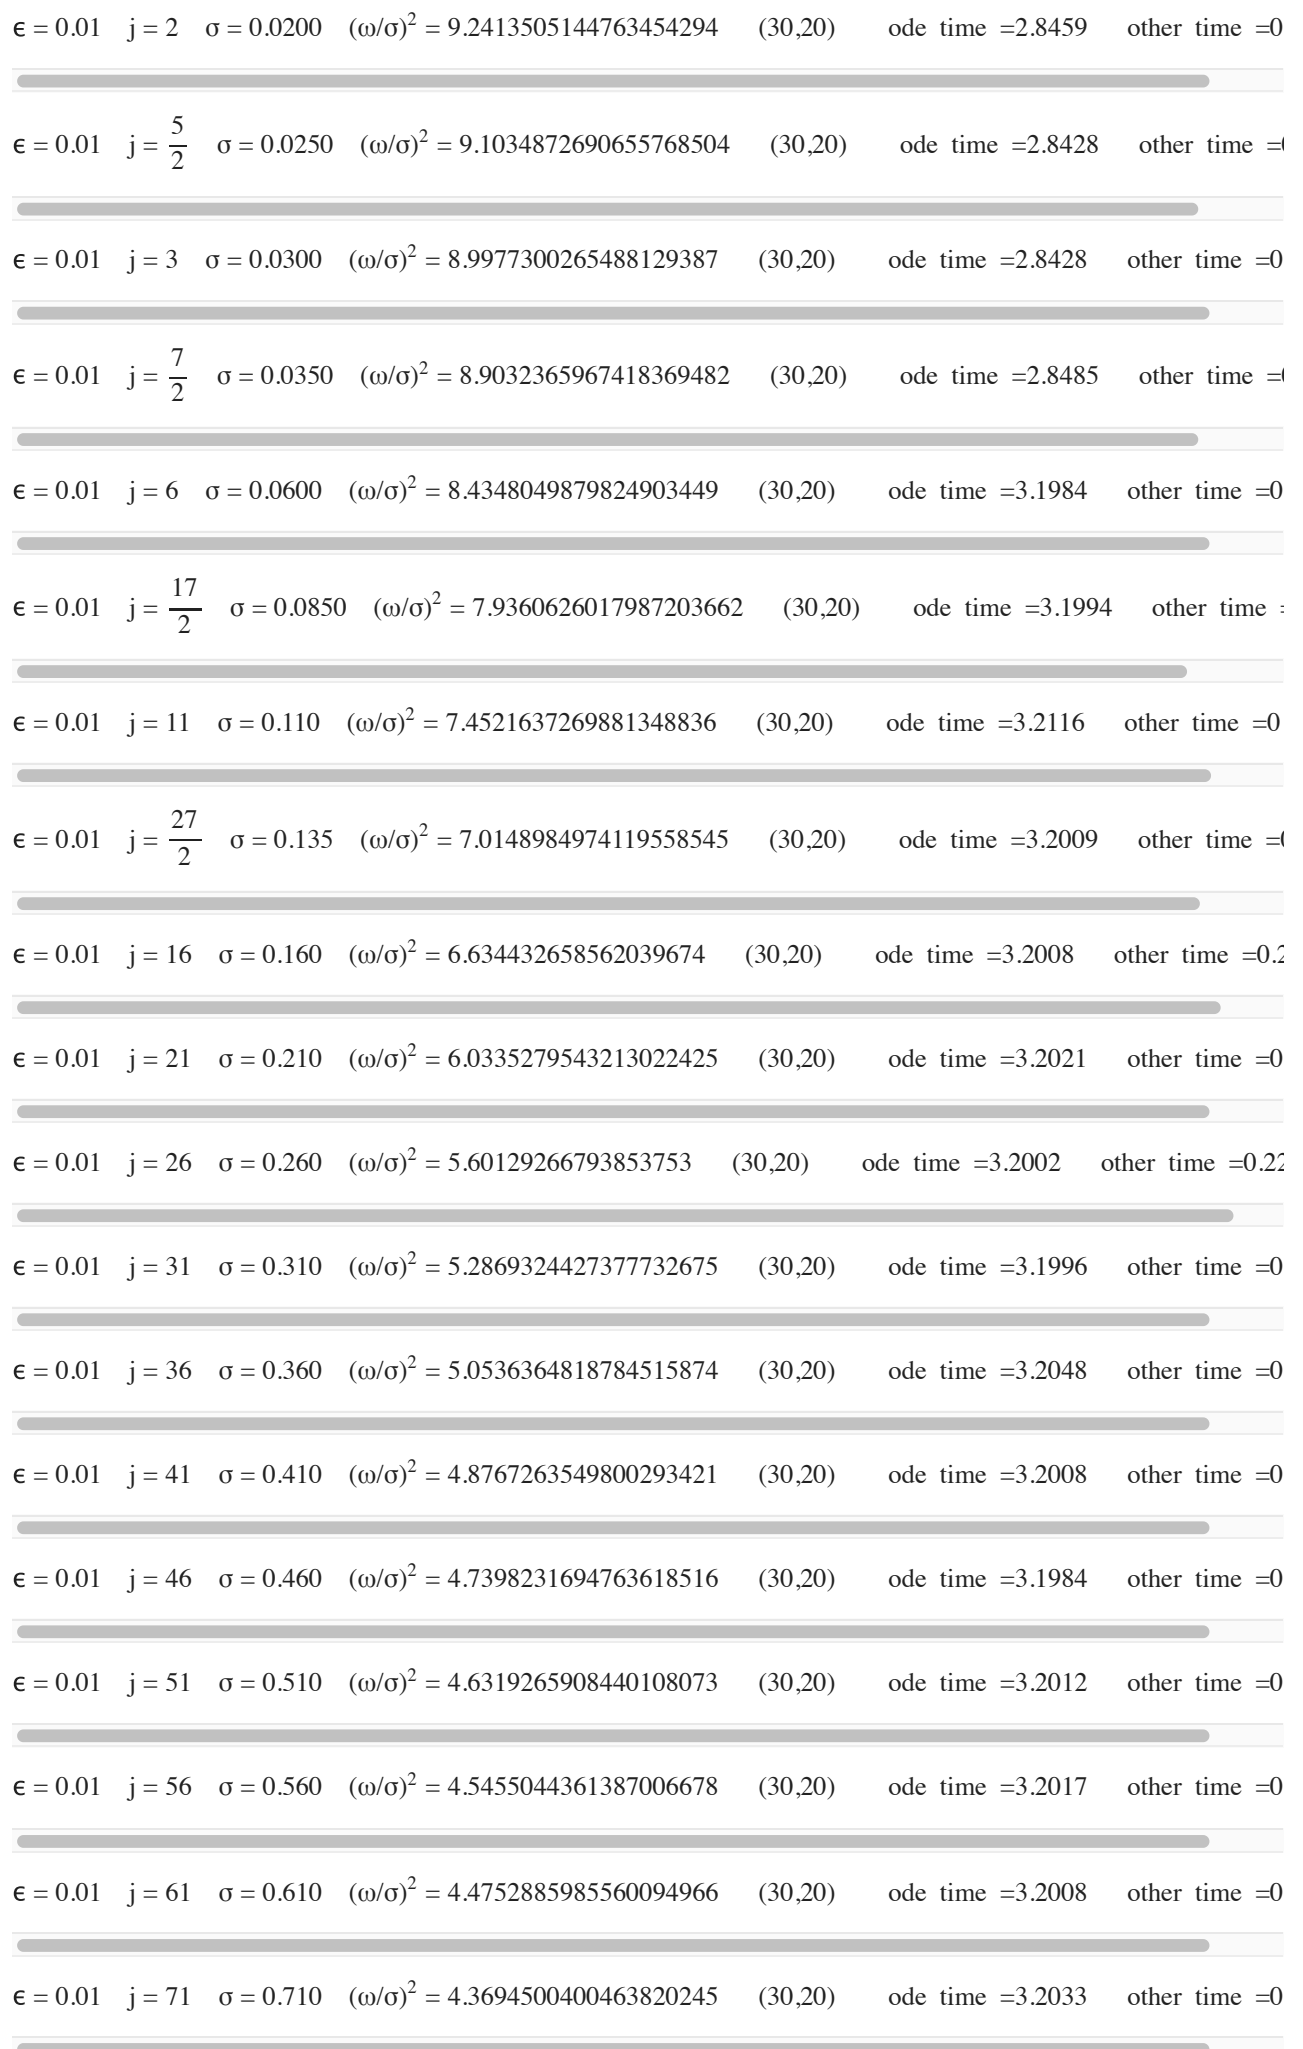   |                    |                   |                                             |         |                  |                  |
| $\epsilon = 0.01$                                                                    | $j = 6$            | $\sigma = 0.0600$ | $(\omega/\sigma)^2 = 8.4348049879824903449$ | (30,20) | ode time =3.1984 | other time =0    |
| 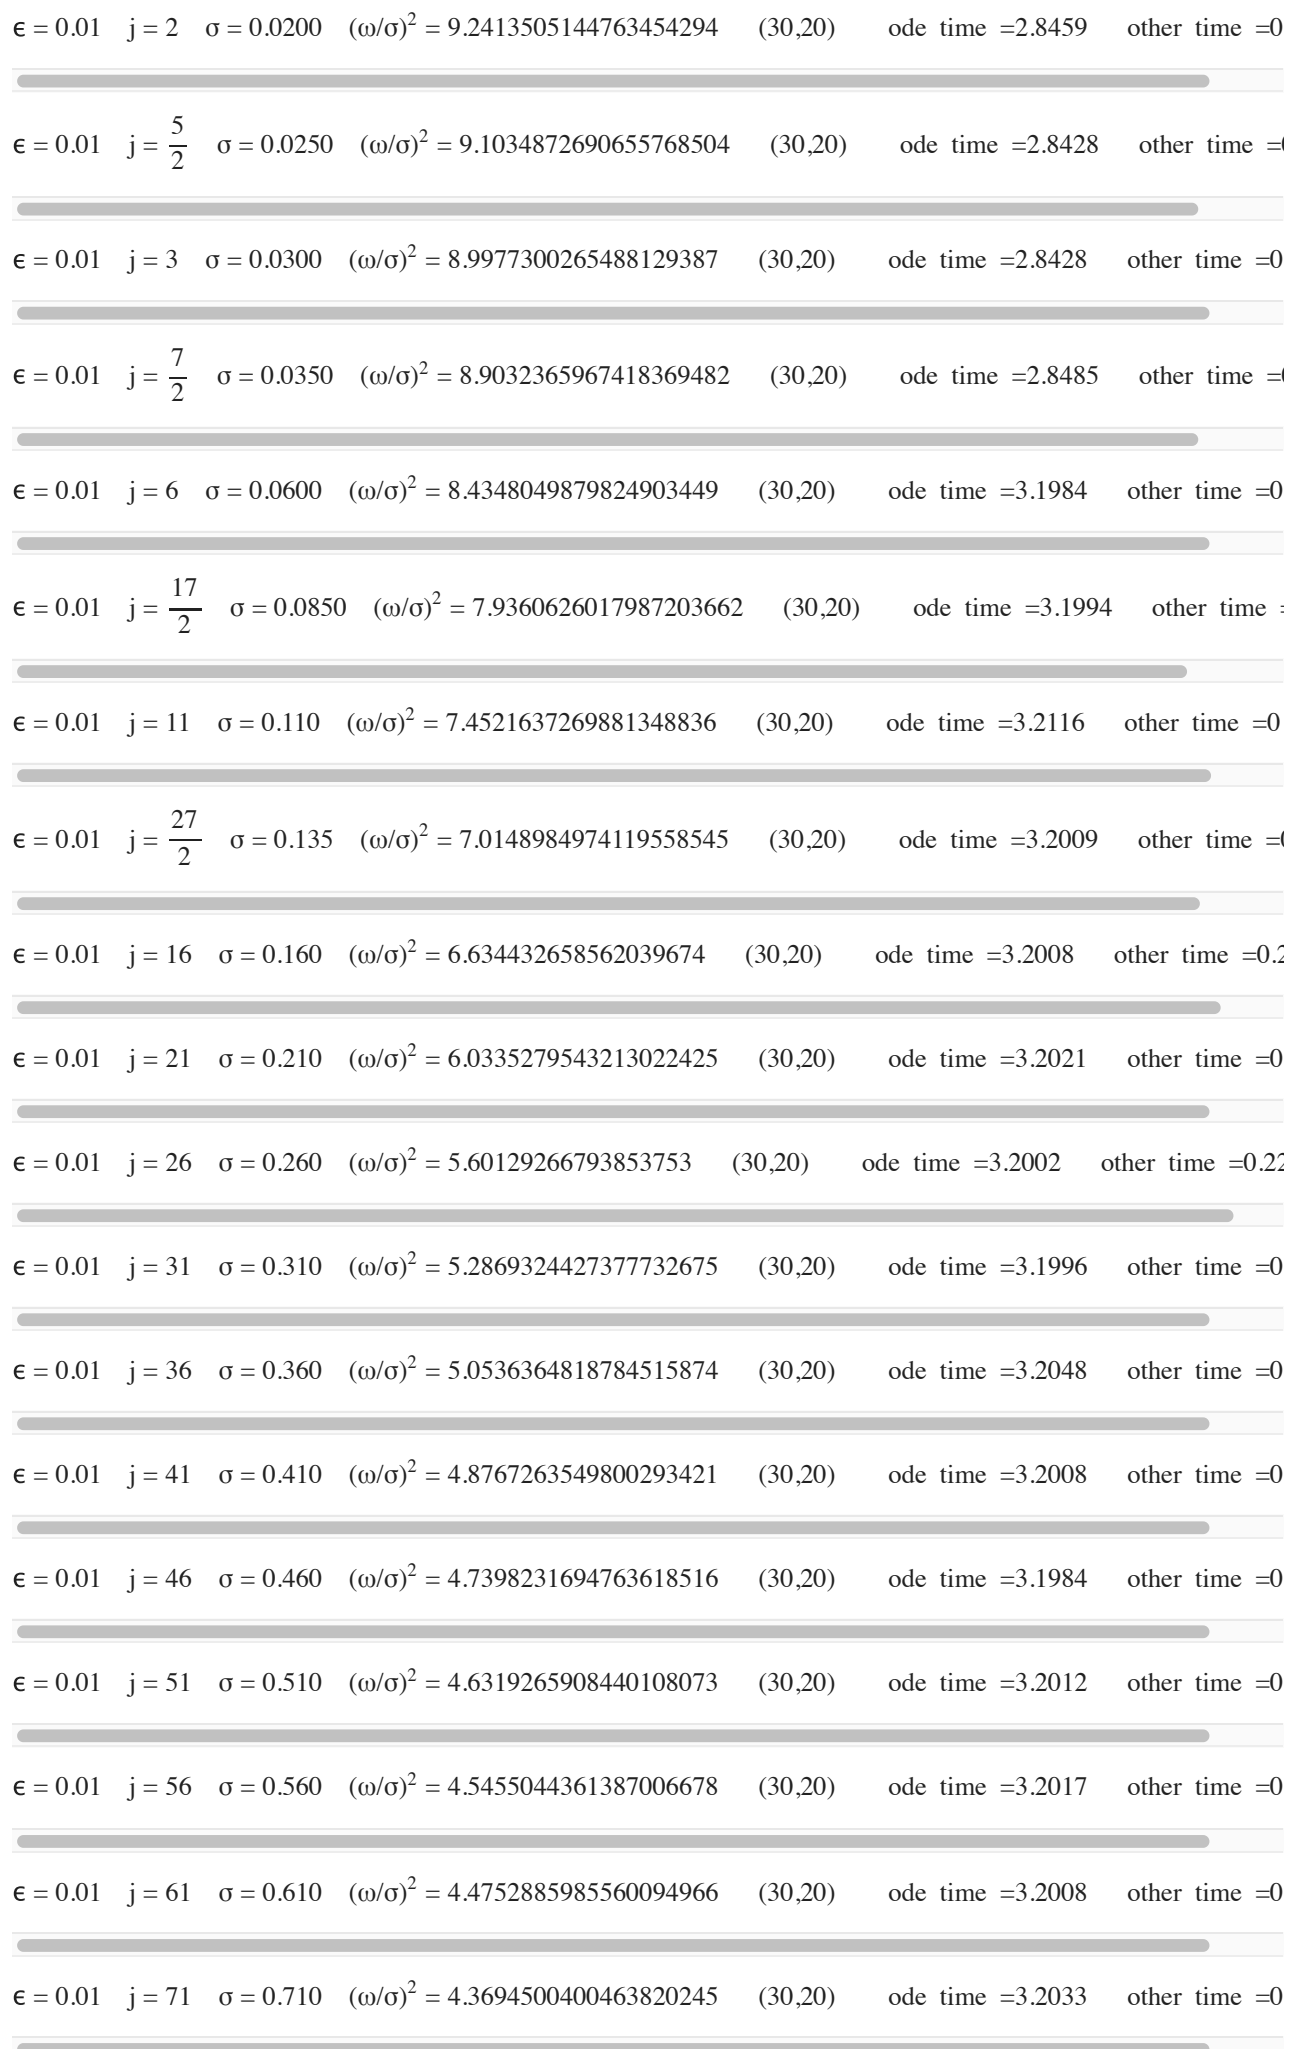   |                    |                   |                                             |         |                  |                  |
| $\epsilon = 0.01$                                                                    | $j = \frac{17}{2}$ | $\sigma = 0.0850$ | $(\omega/\sigma)^2 = 7.9360626017987203662$ | (30,20) | ode time =3.1994 | other time =0    |
| 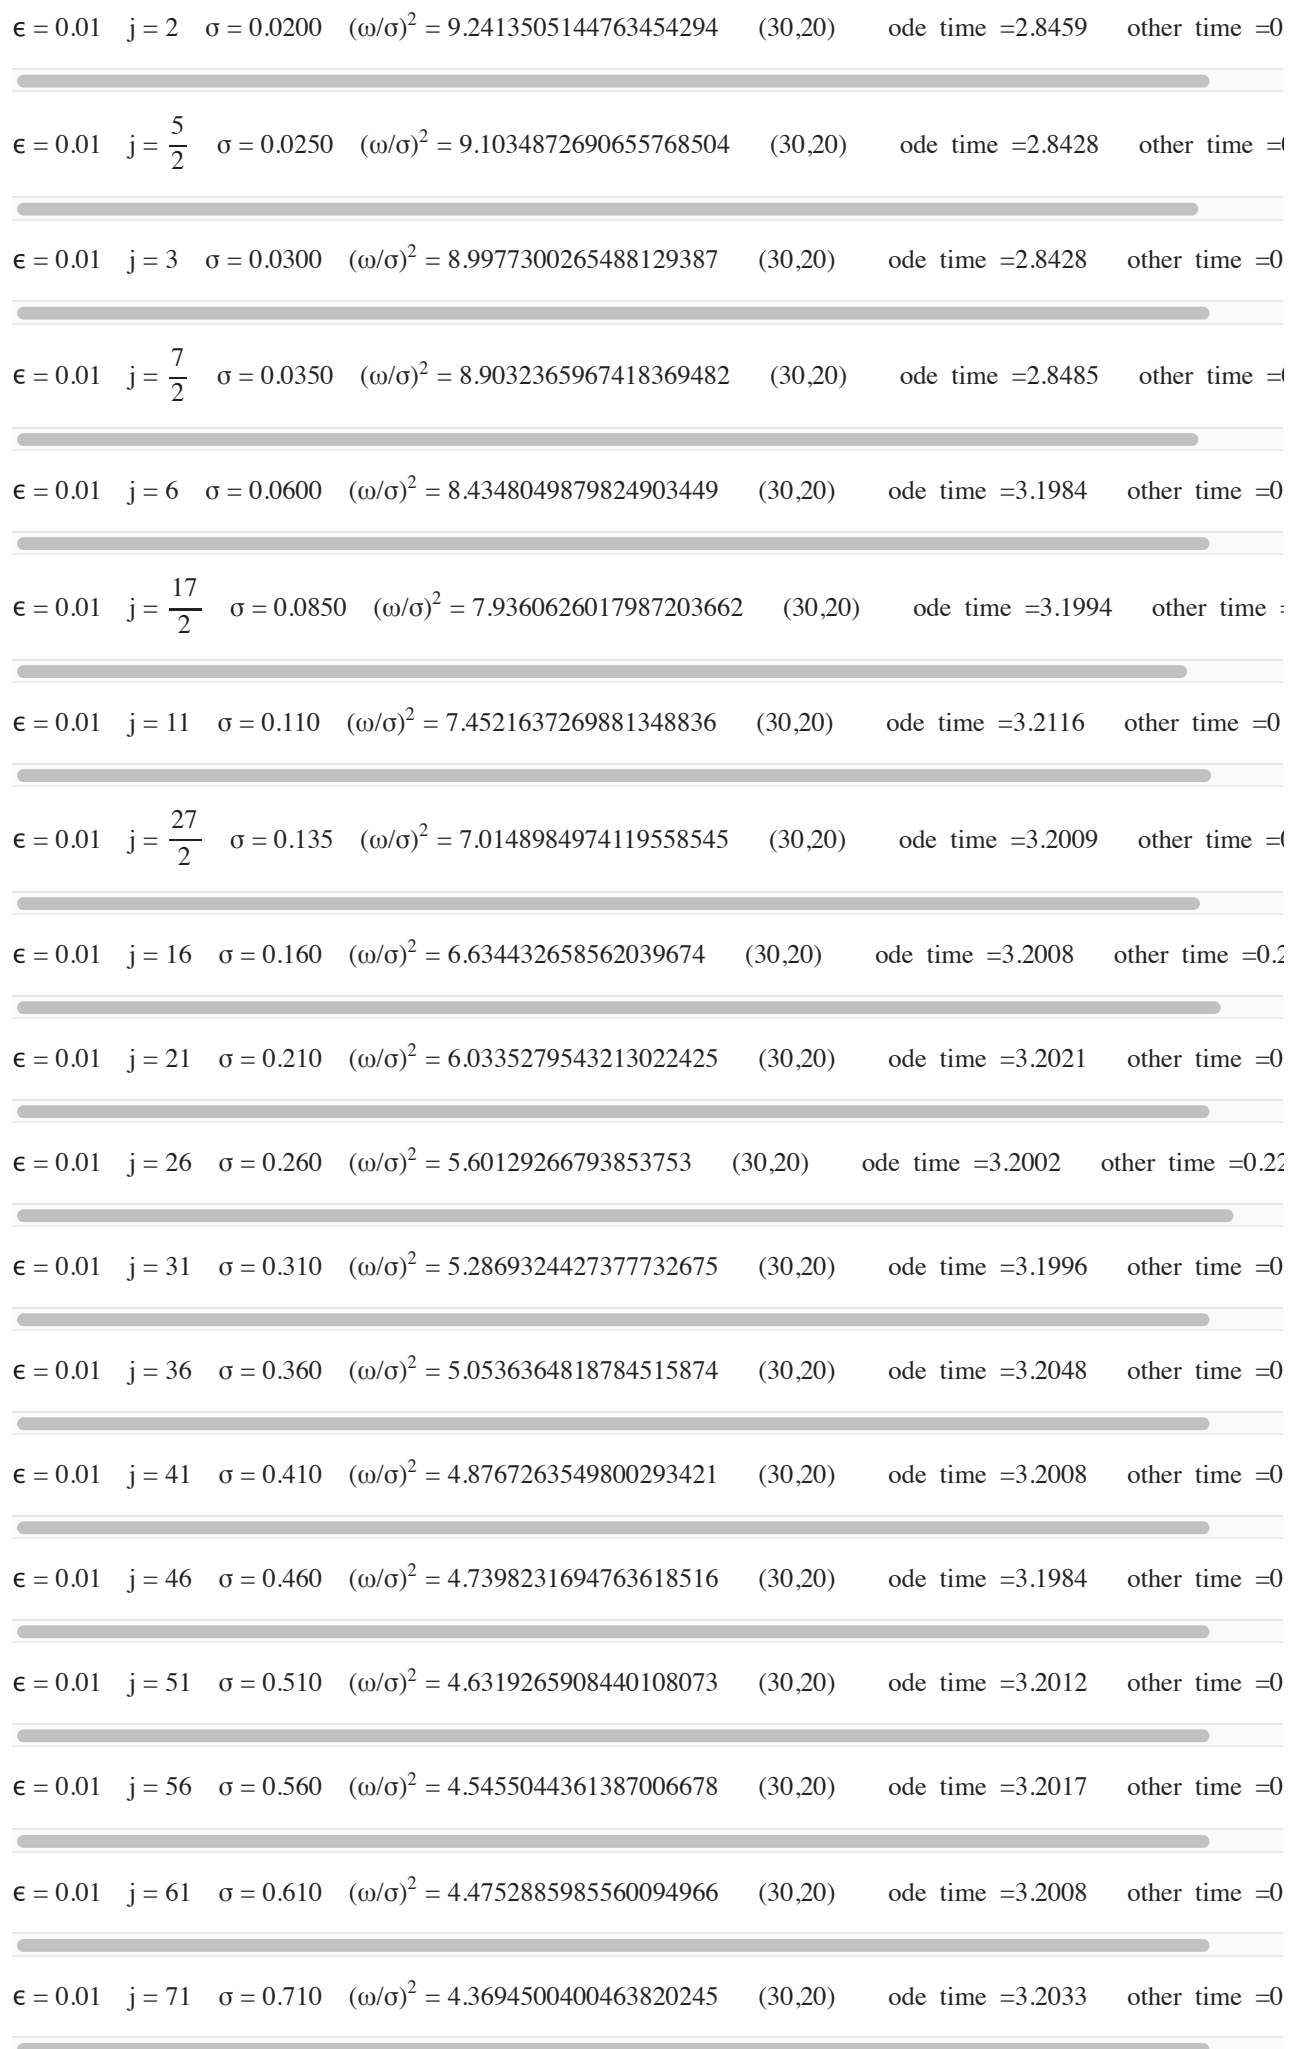   |                    |                   |                                             |         |                  |                  |
| $\epsilon = 0.01$                                                                    | $j = 11$           | $\sigma = 0.110$  | $(\omega/\sigma)^2 = 7.4521637269881348836$ | (30,20) | ode time =3.2116 | other time =0    |
| 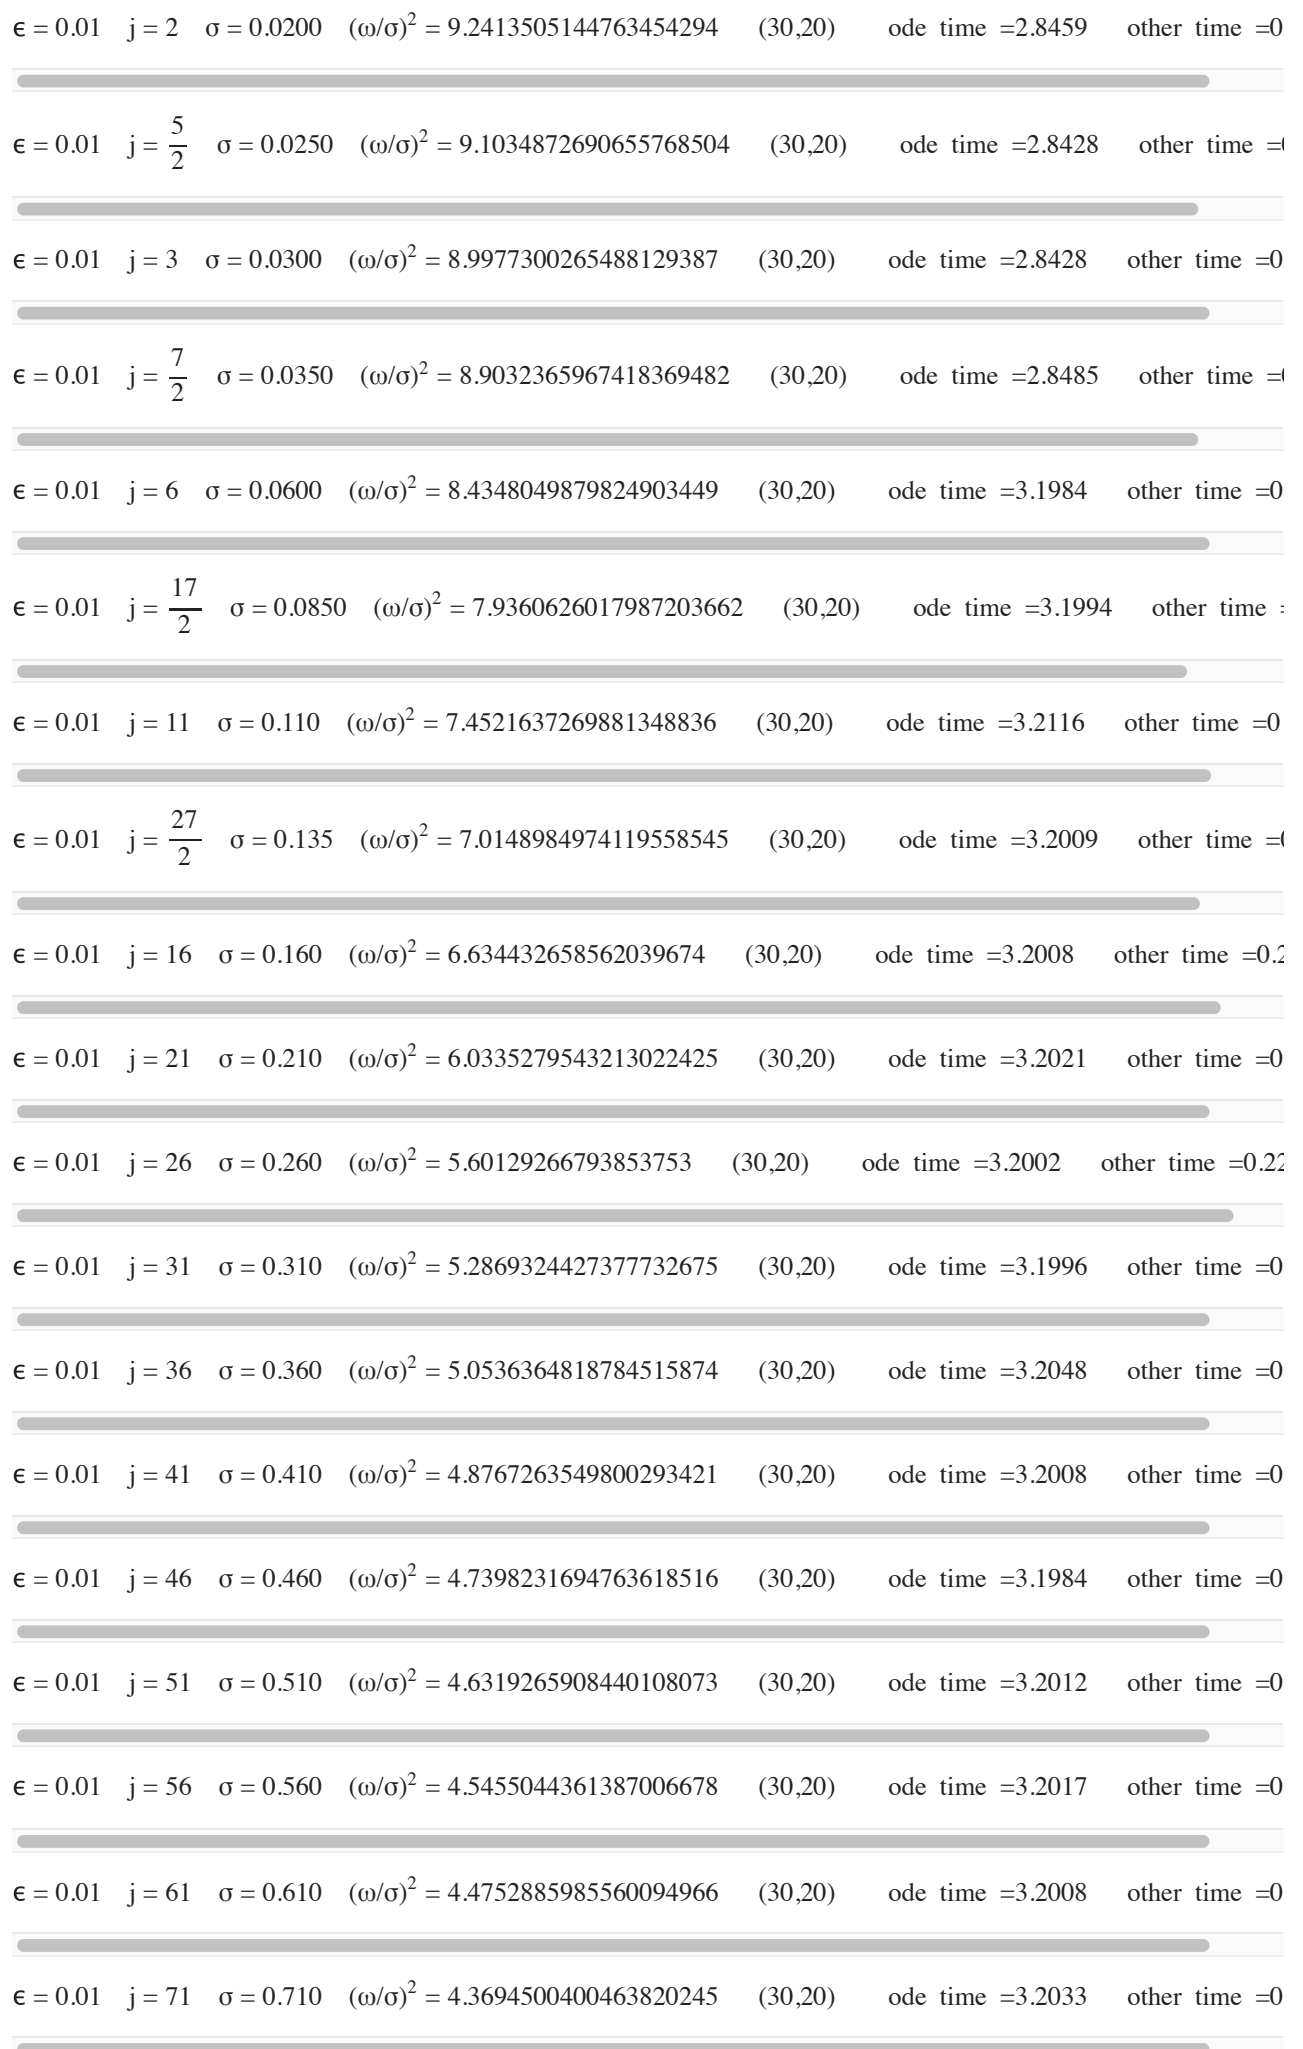   |                    |                   |                                             |         |                  |                  |
| $\epsilon = 0.01$                                                                    | $j = \frac{27}{2}$ | $\sigma = 0.135$  | $(\omega/\sigma)^2 = 7.0148984974119558545$ | (30,20) | ode time =3.2009 | other time =0    |
| 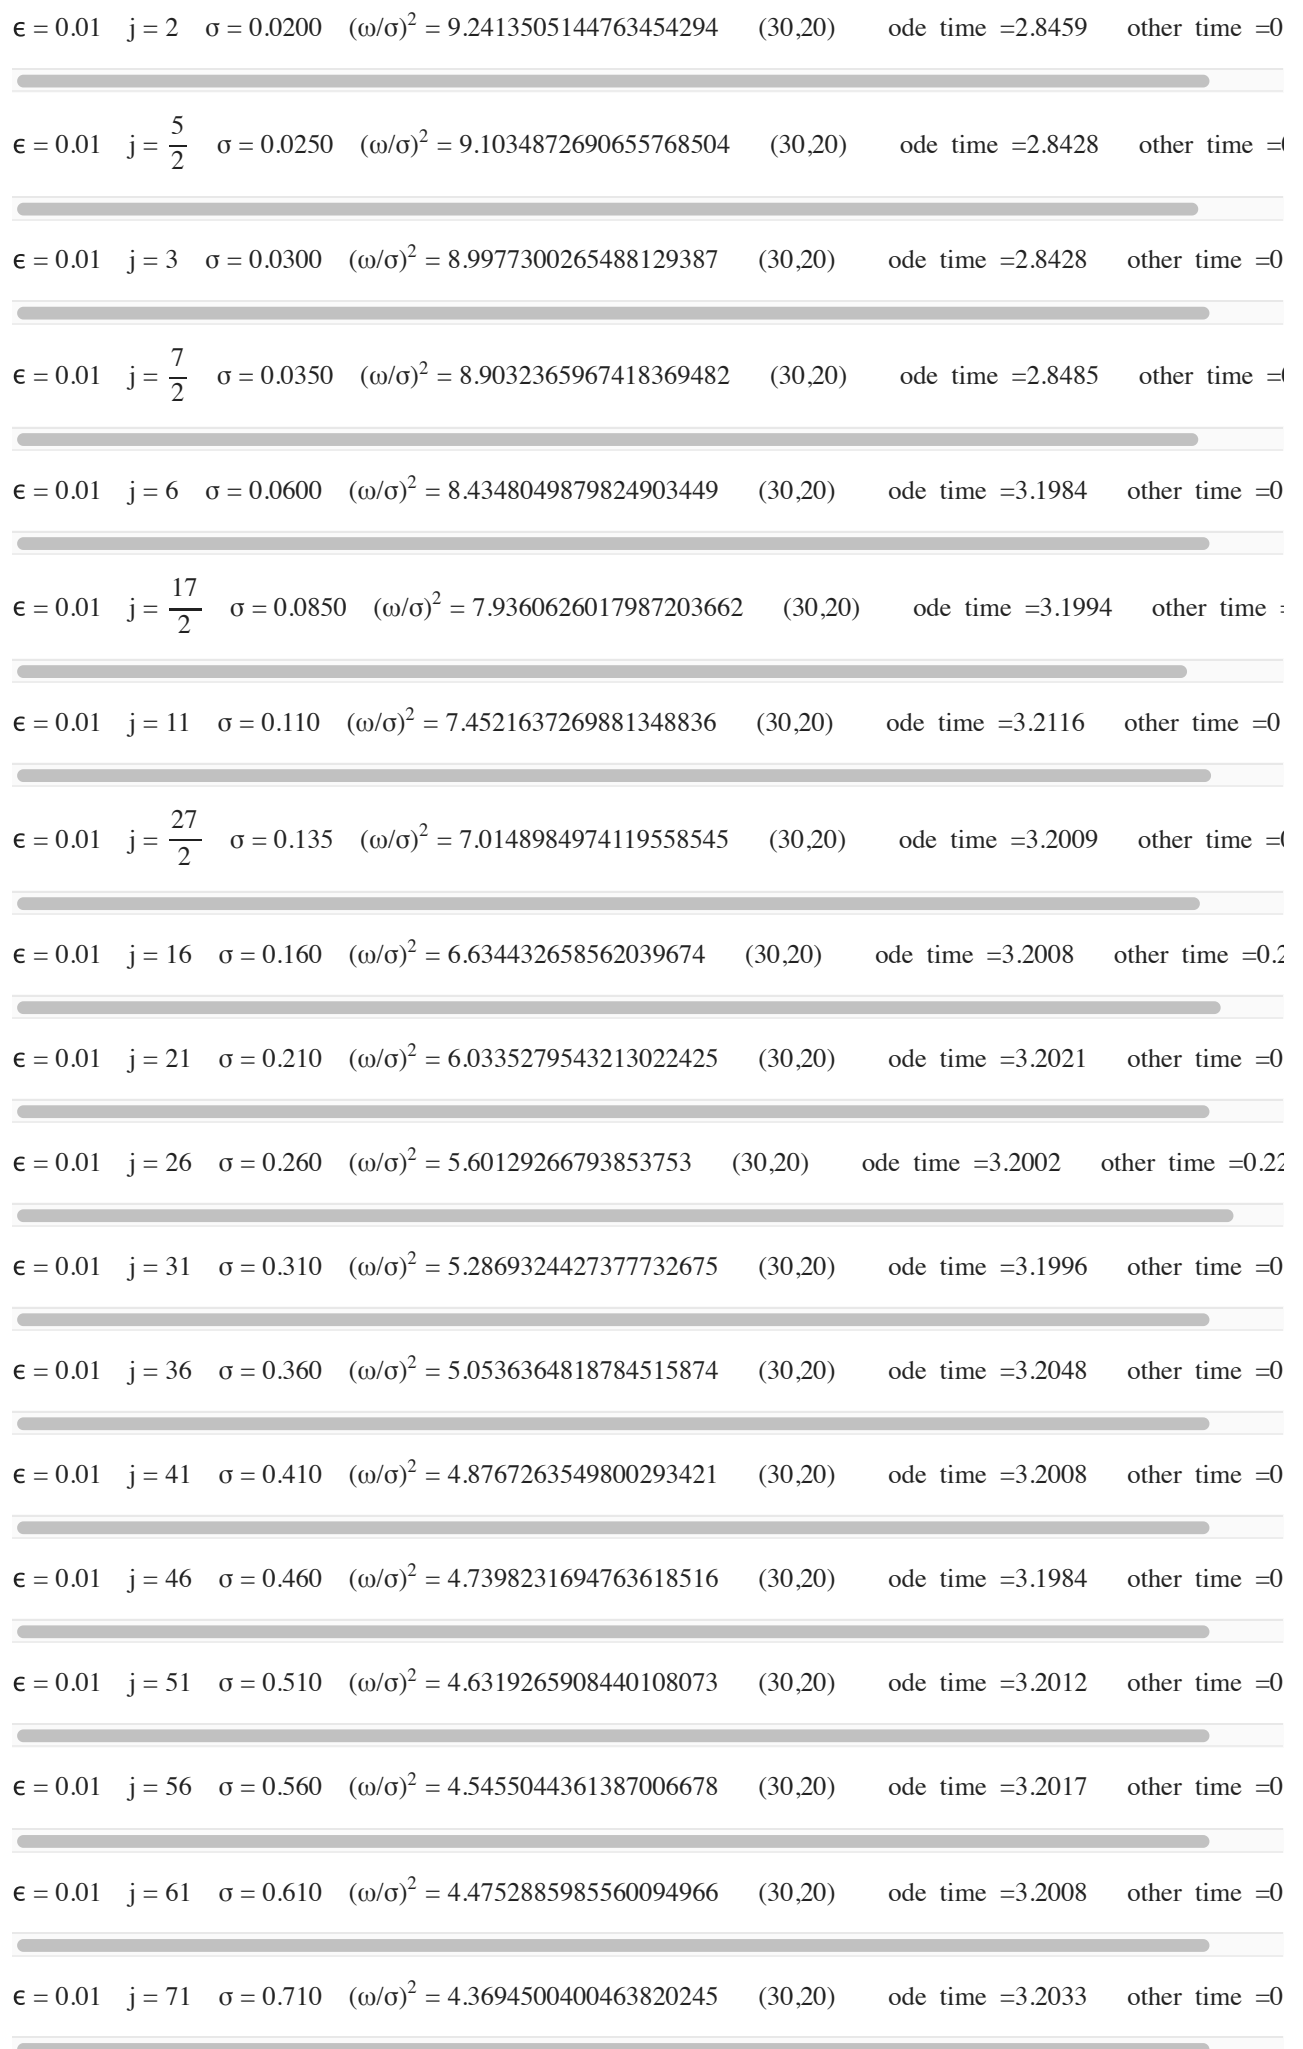   |                    |                   |                                             |         |                  |                  |
| $\epsilon = 0.01$                                                                    | $j = 16$           | $\sigma = 0.160$  | $(\omega/\sigma)^2 = 6.634432658562039674$  | (30,20) | ode time =3.2008 | other time =0.2  |
| 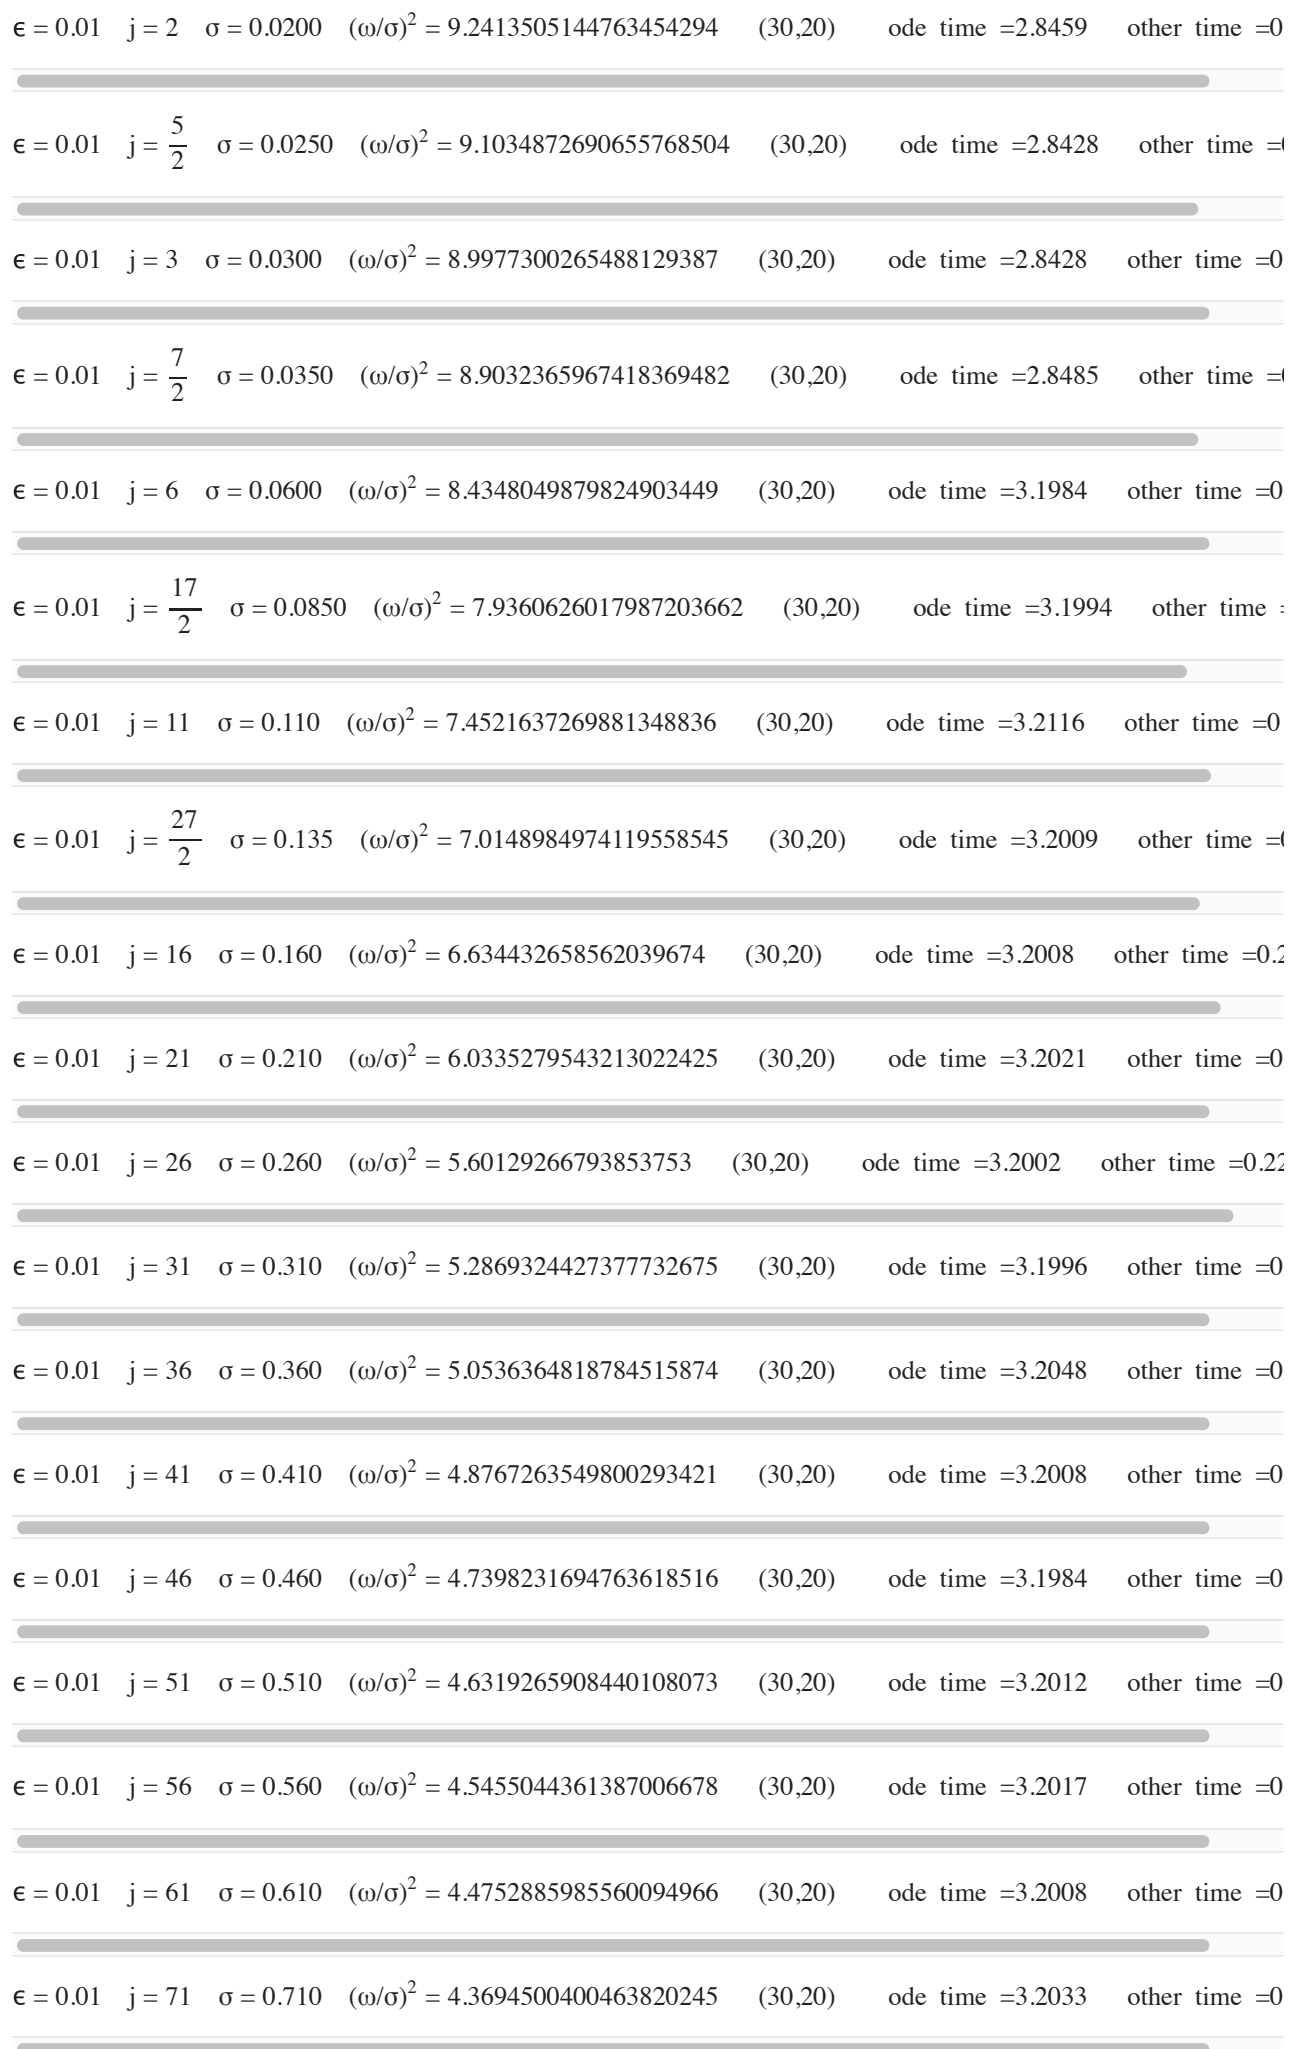 |                    |                   |                                             |         |                  |                  |
| $\epsilon = 0.01$                                                                    | $j = 21$           | $\sigma = 0.210$  | $(\omega/\sigma)^2 = 6.0335279543213022425$ | (30,20) | ode time =3.2021 | other time =0    |
| 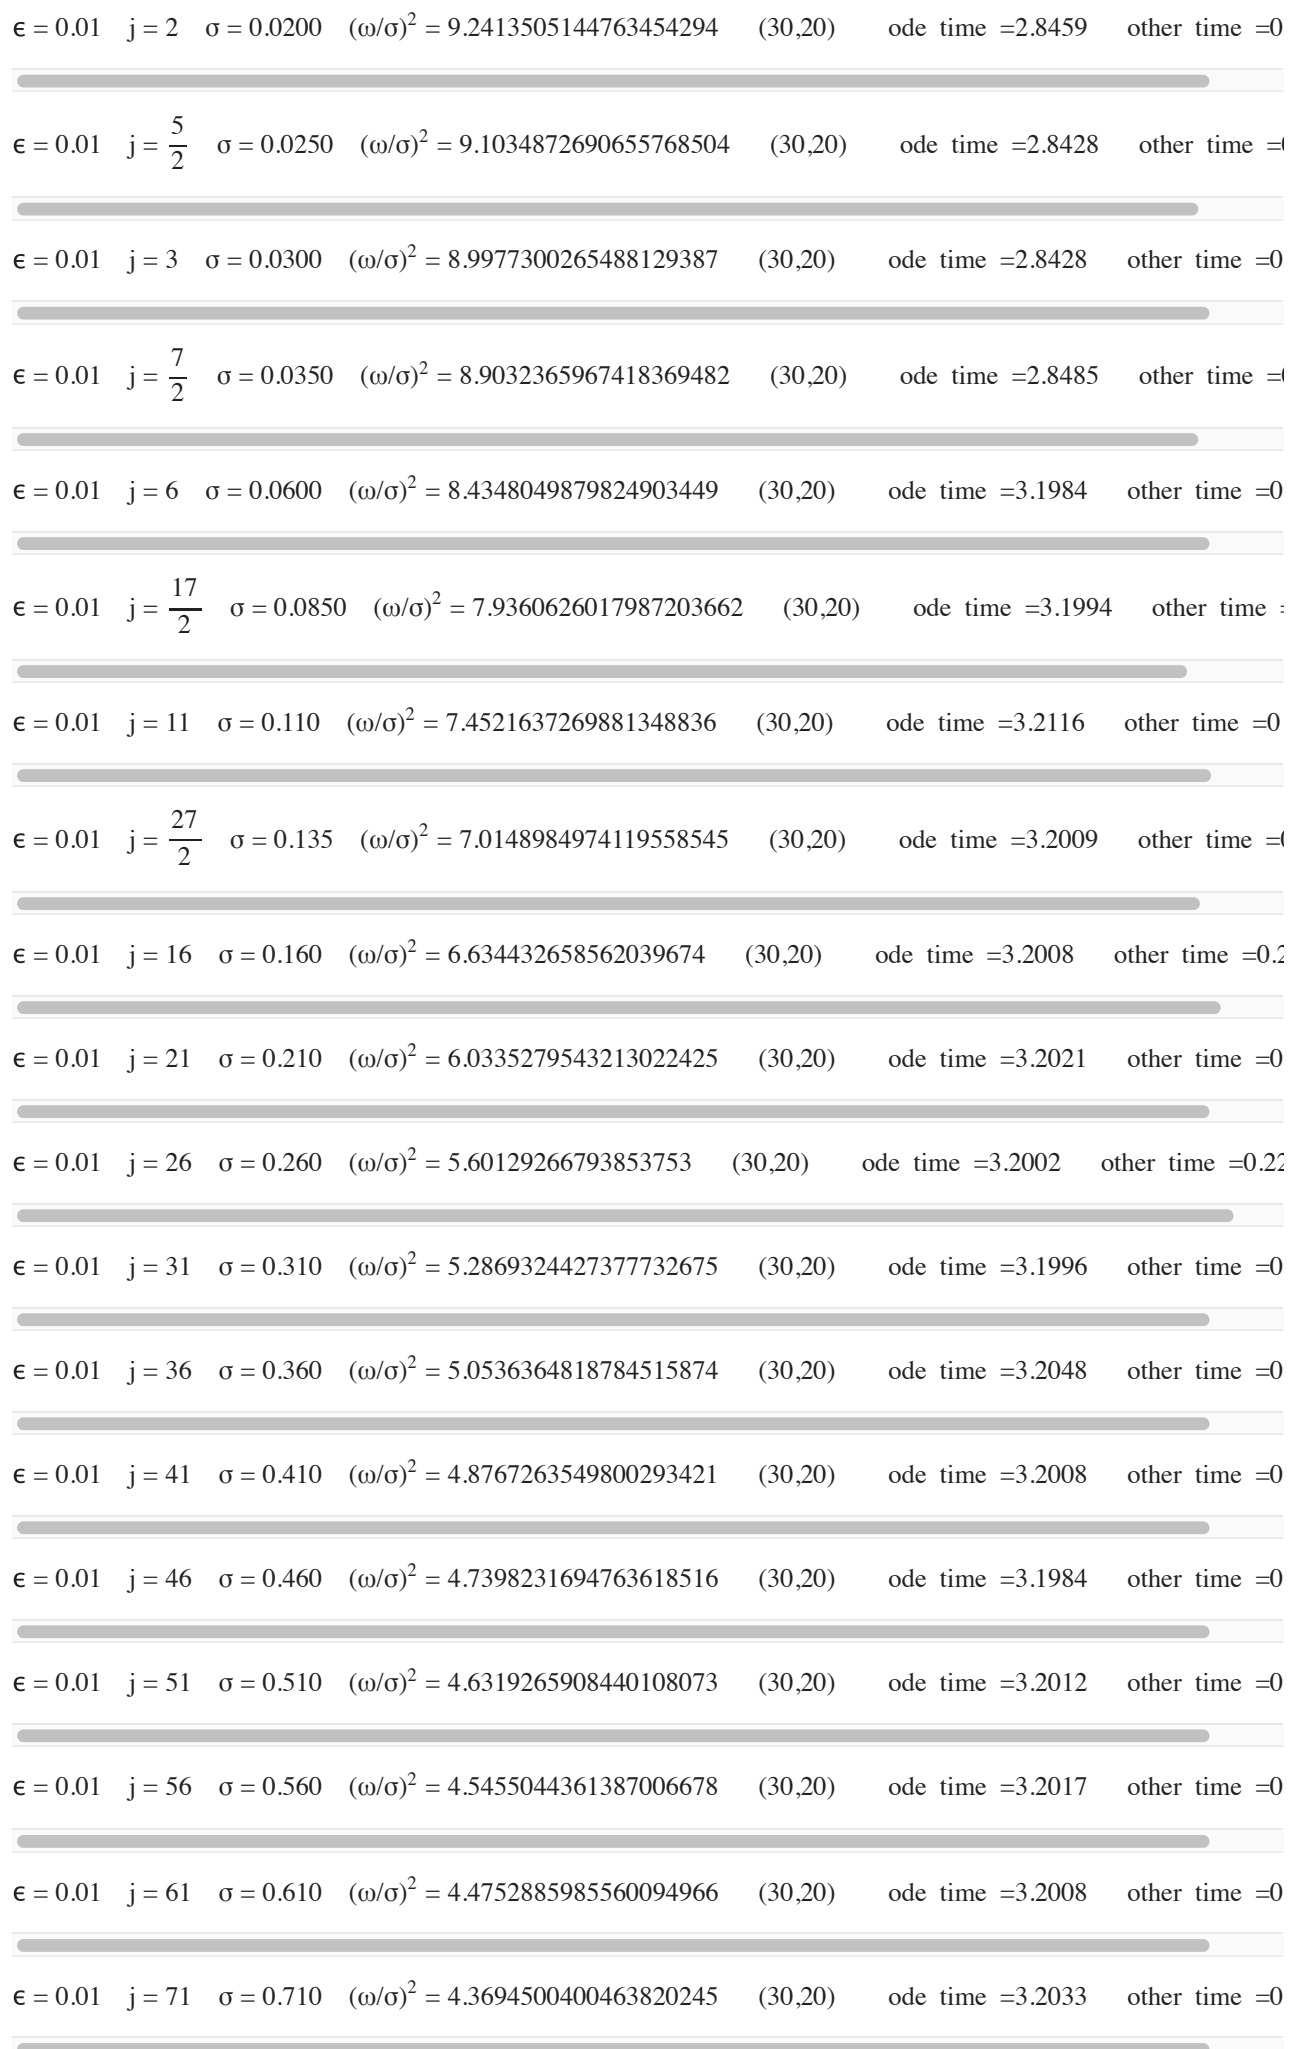 |                    |                   |                                             |         |                  |                  |
| $\epsilon = 0.01$                                                                    | $j = 26$           | $\sigma = 0.260$  | $(\omega/\sigma)^2 = 5.60129266793853753$   | (30,20) | ode time =3.2002 | other time =0.22 |
| 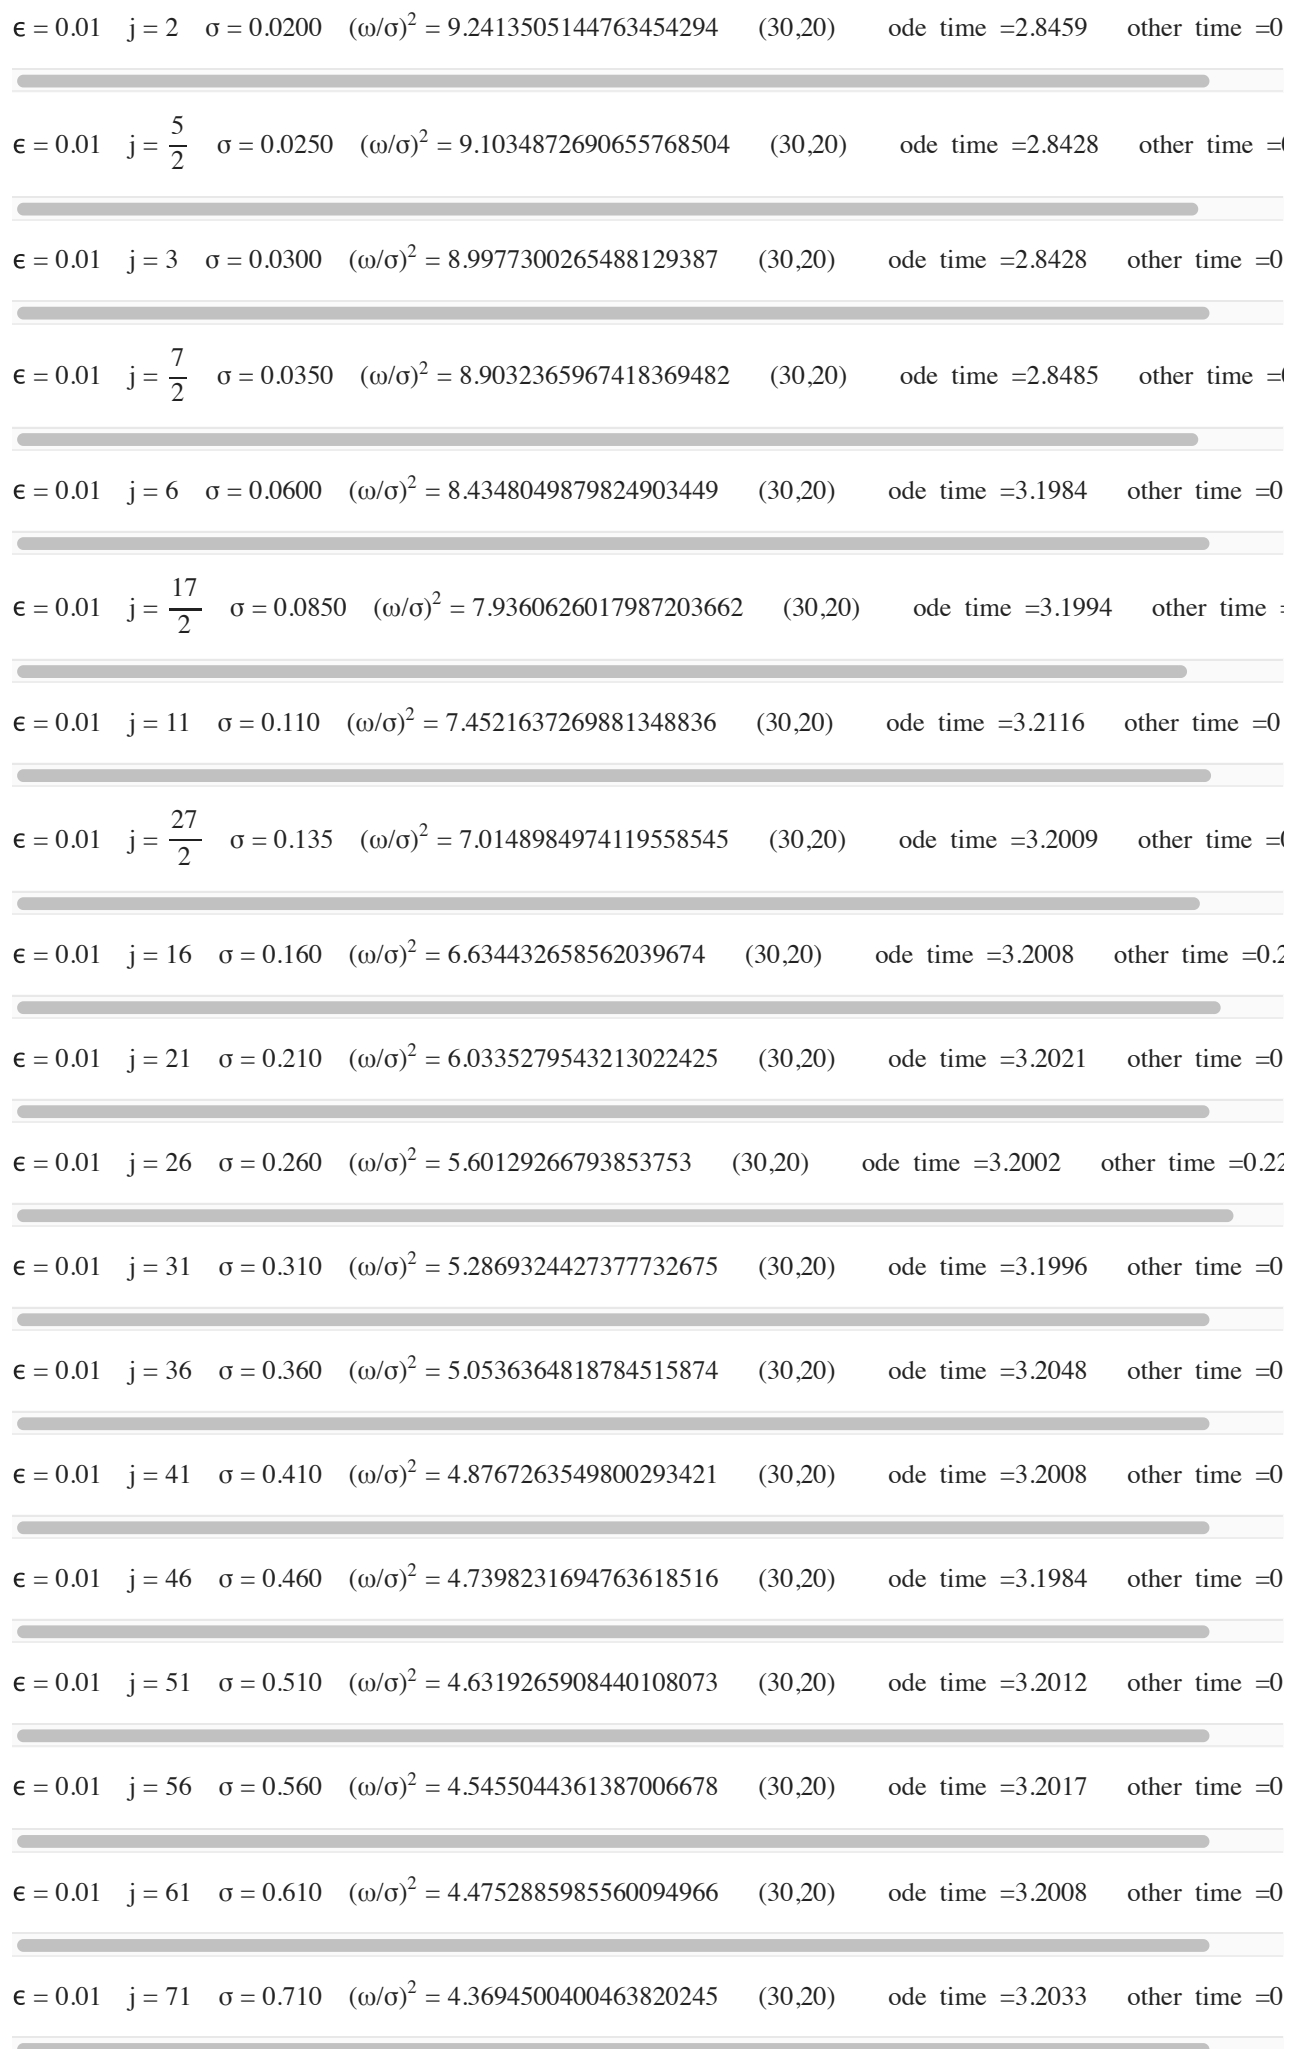 |                    |                   |                                             |         |                  |                  |
| $\epsilon = 0.01$                                                                    | $j = 31$           | $\sigma = 0.310$  | $(\omega/\sigma)^2 = 5.2869324427377732675$ | (30,20) | ode time =3.1996 | other time =0    |
| 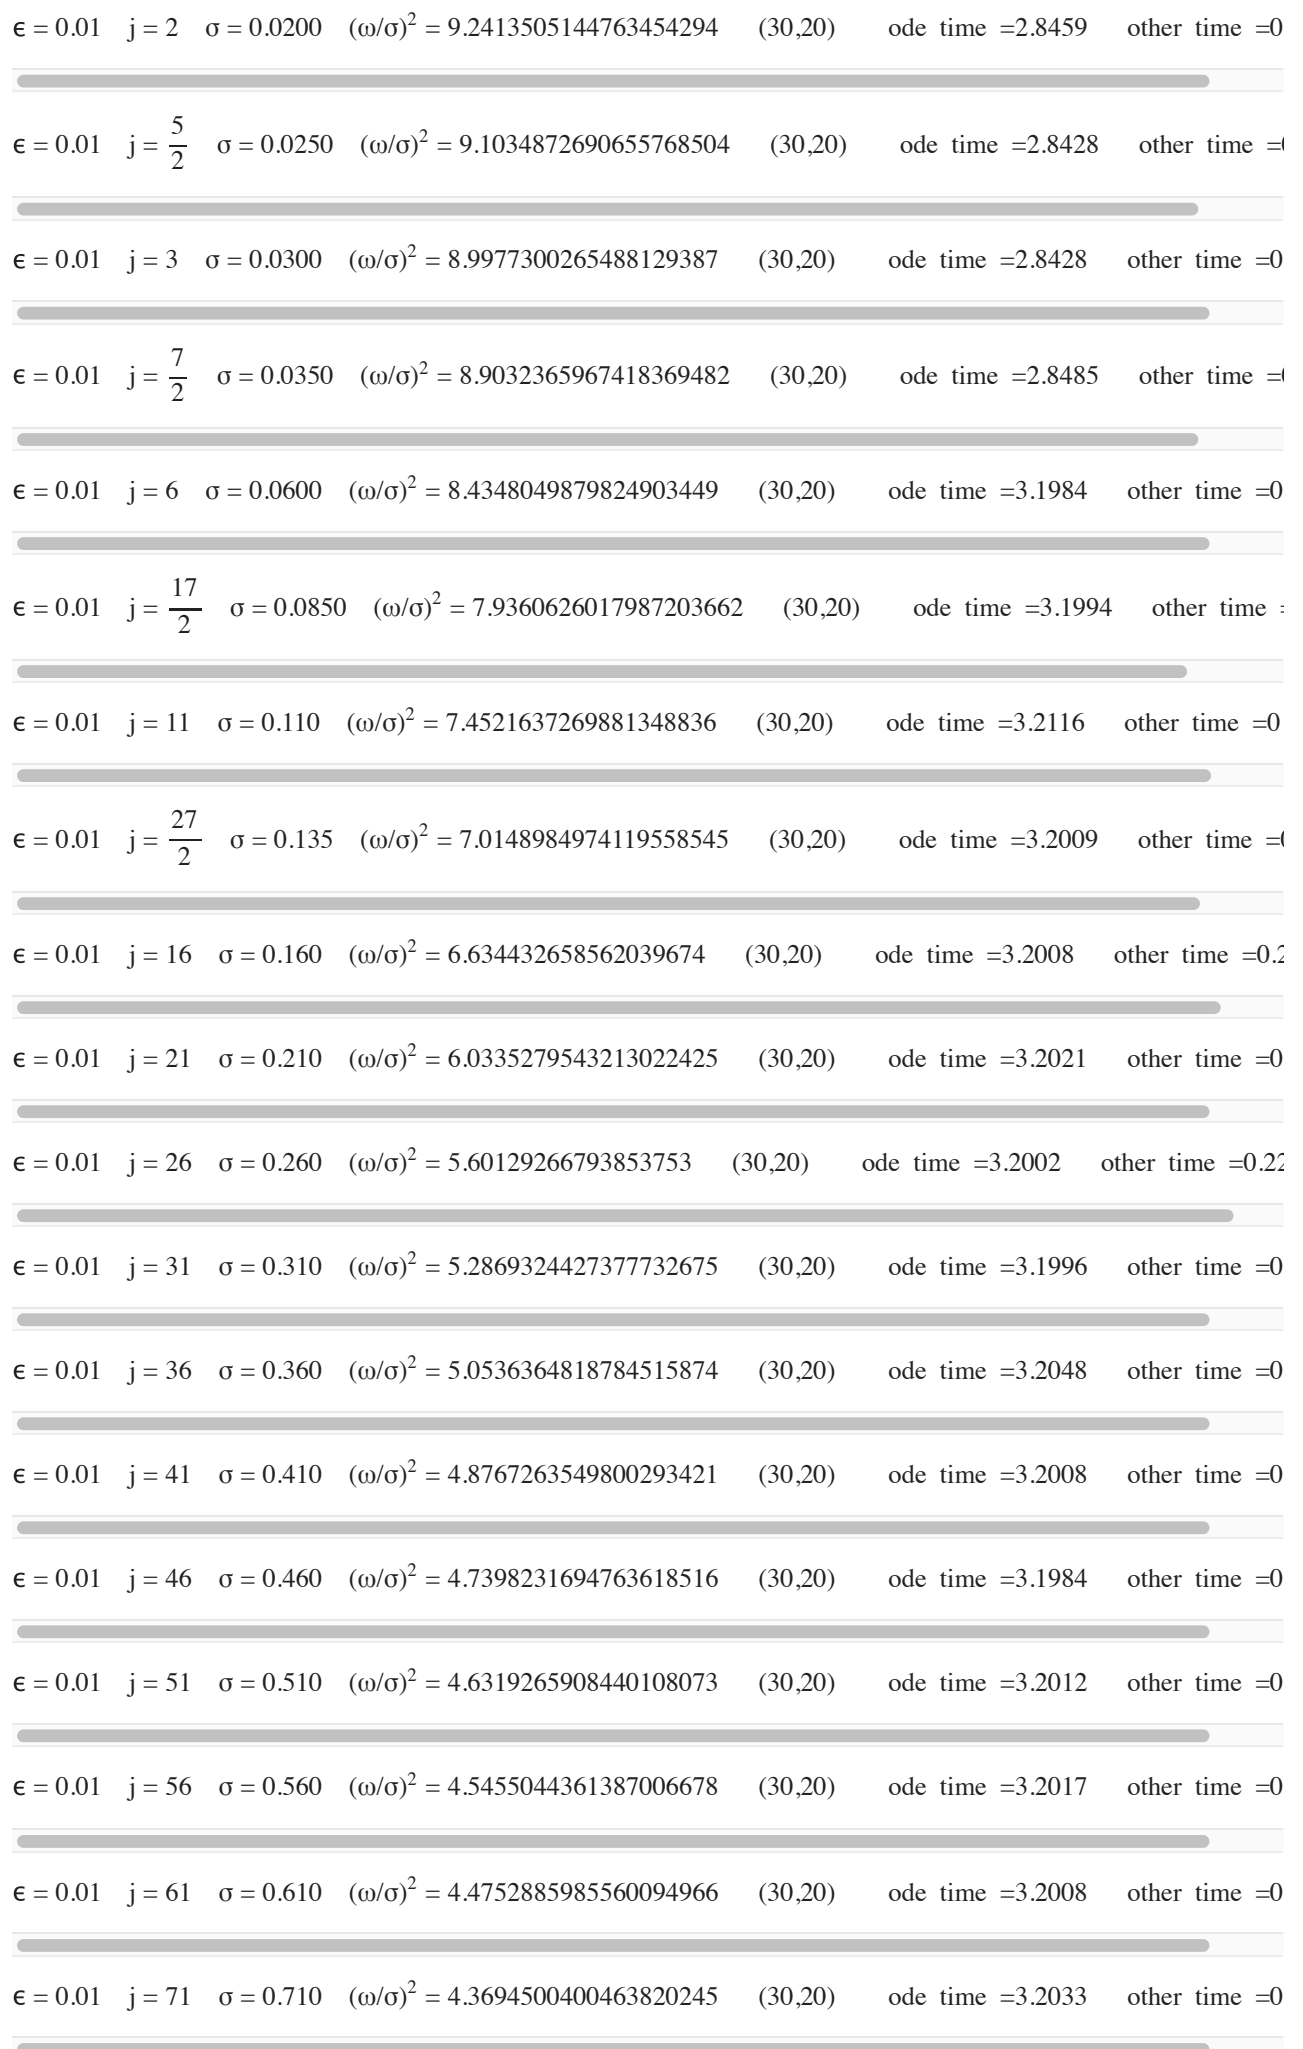 |                    |                   |                                             |         |                  |                  |
| $\epsilon = 0.01$                                                                    | $j = 36$           | $\sigma = 0.360$  | $(\omega/\sigma)^2 = 5.0536364818784515874$ | (30,20) | ode time =3.2048 | other time =0    |
| 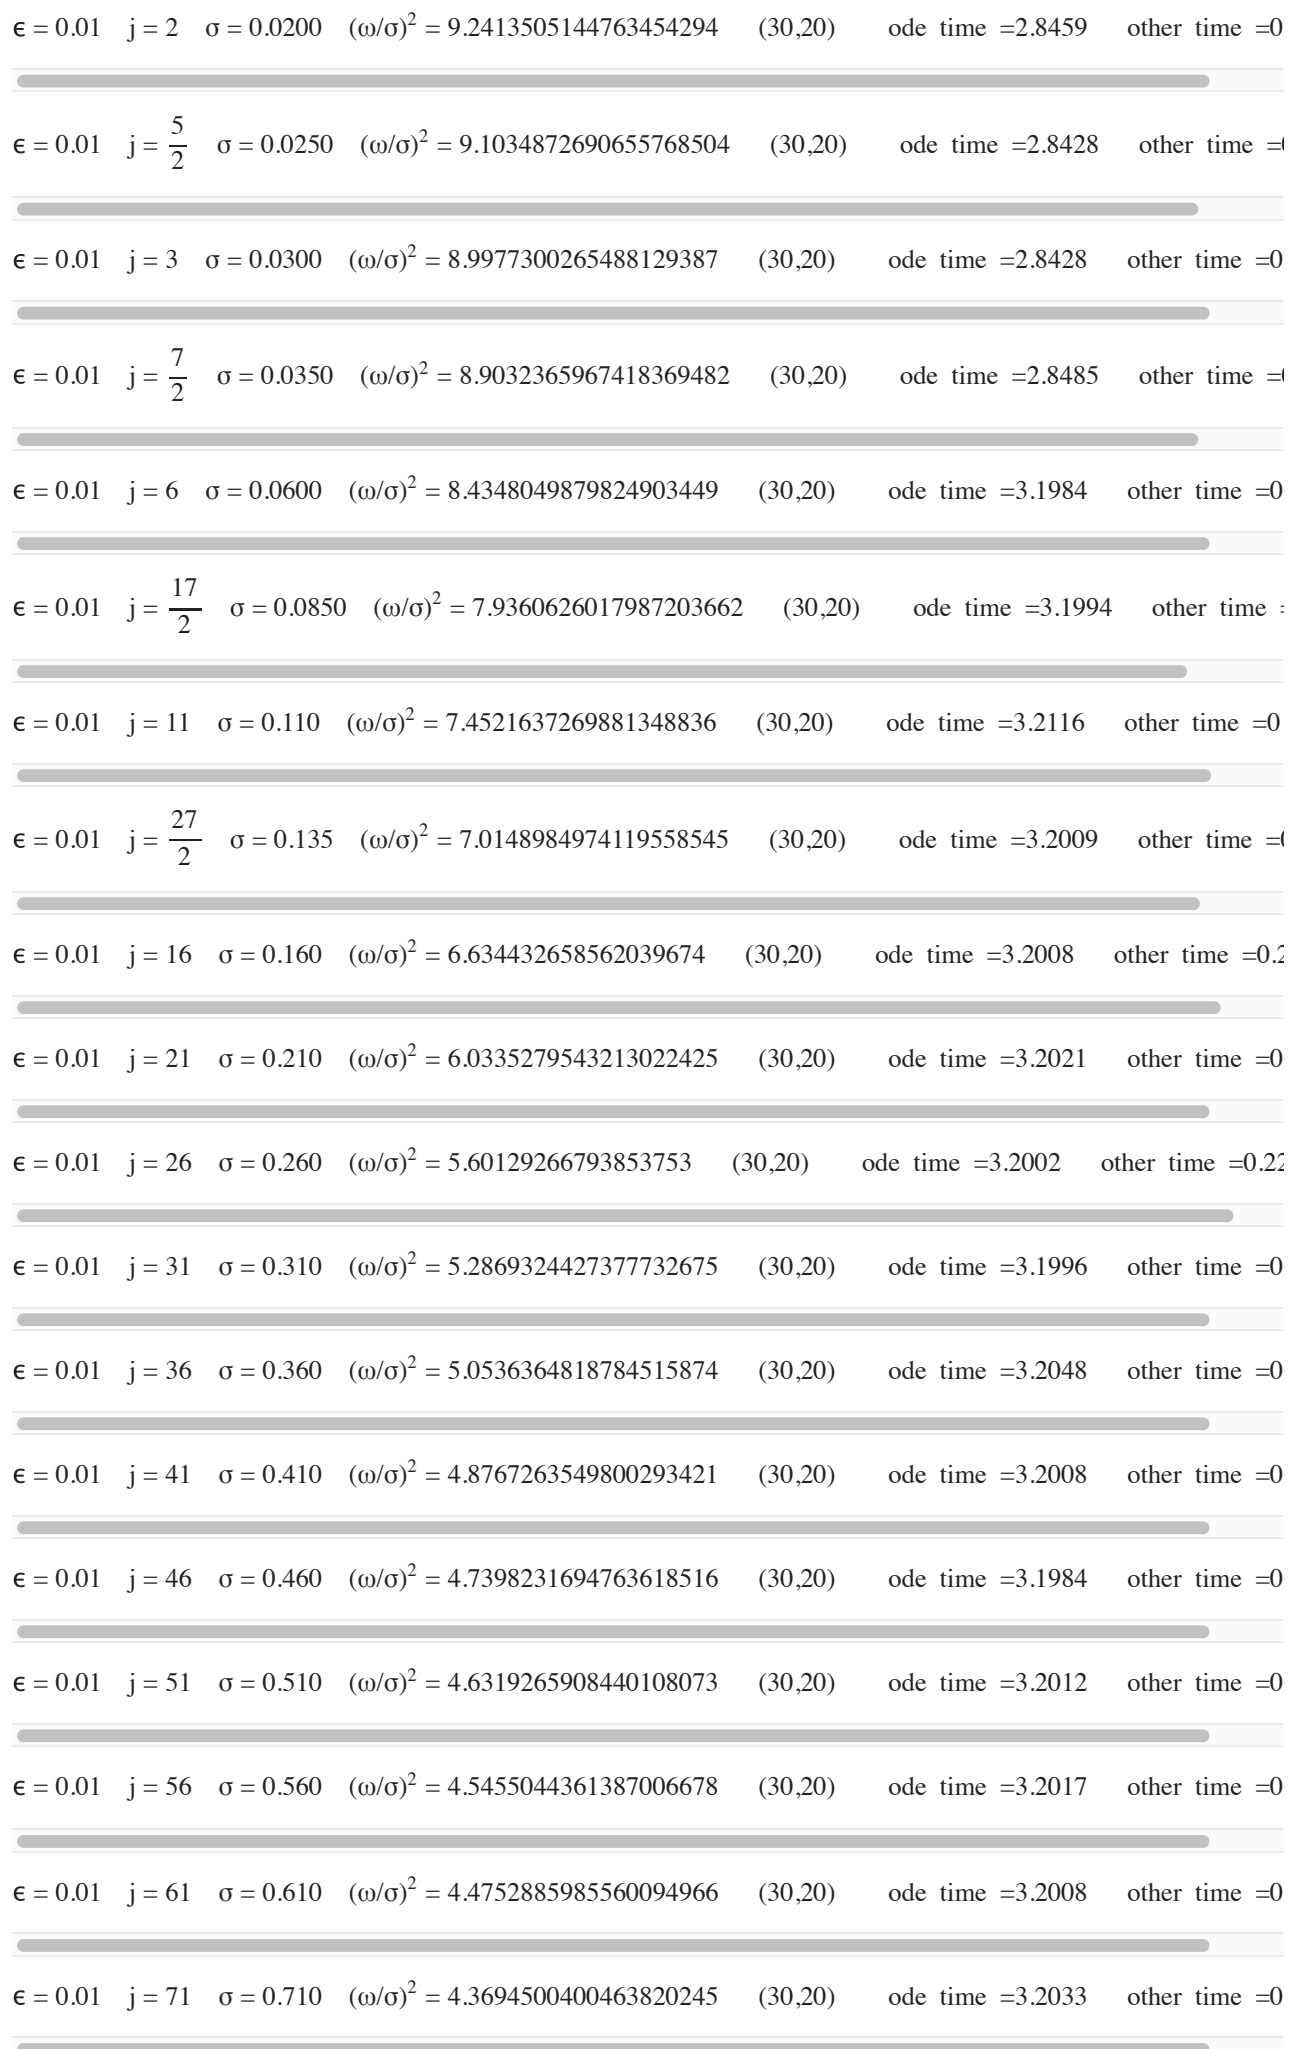 |                    |                   |                                             |         |                  |                  |
| $\epsilon = 0.01$                                                                    | $j = 41$           | $\sigma = 0.410$  | $(\omega/\sigma)^2 = 4.8767263549800293421$ | (30,20) | ode time =3.2008 | other time =0    |
| 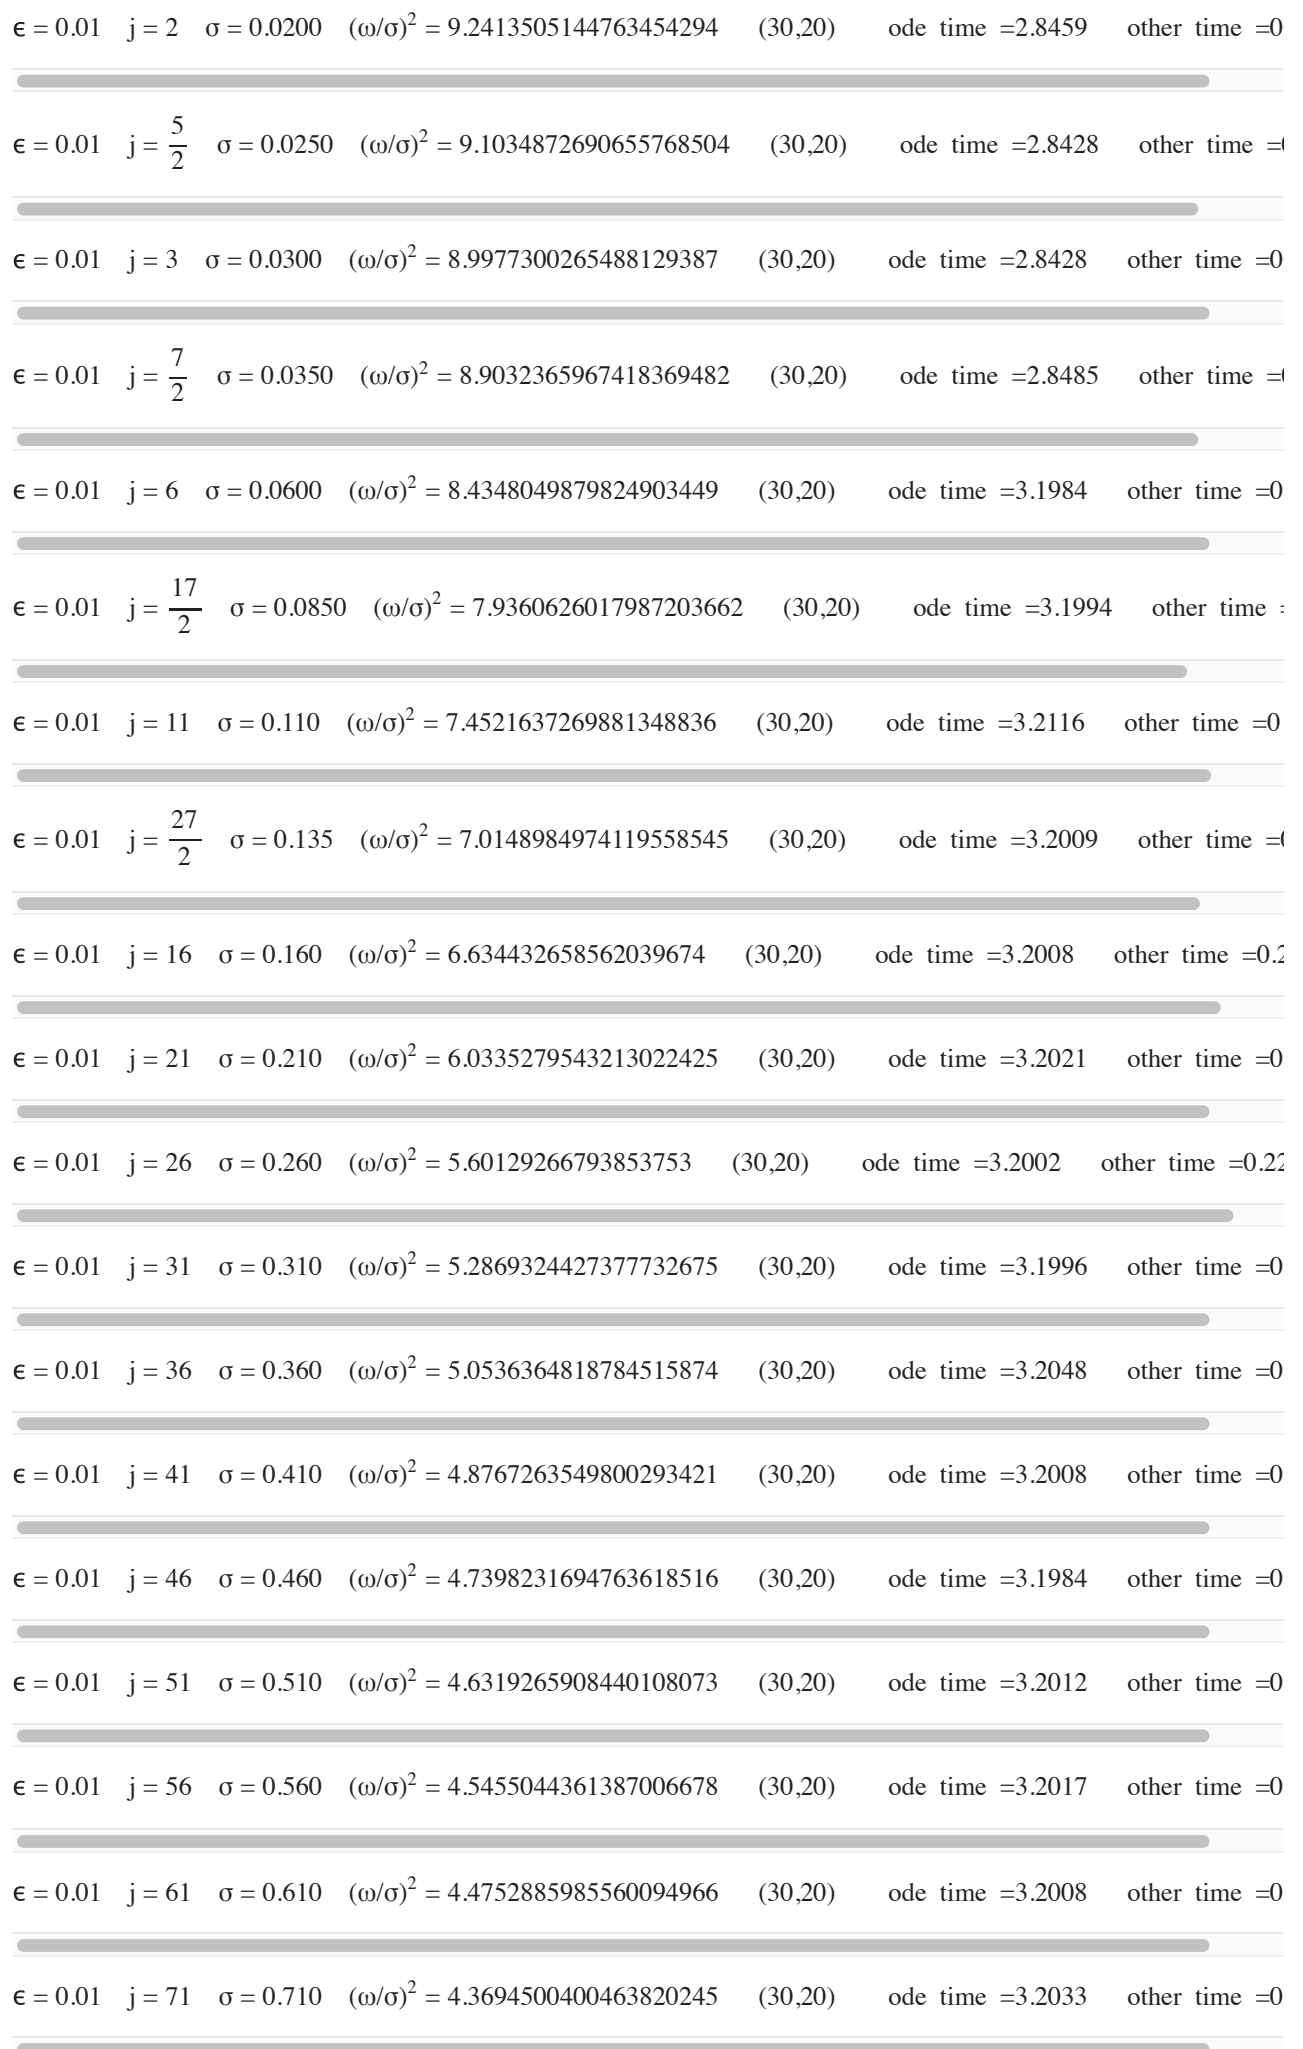 |                    |                   |                                             |         |                  |                  |
| $\epsilon = 0.01$                                                                    | $j = 46$           | $\sigma = 0.460$  | $(\omega/\sigma)^2 = 4.7398231694763618516$ | (30,20) | ode time =3.1984 | other time =0    |
| 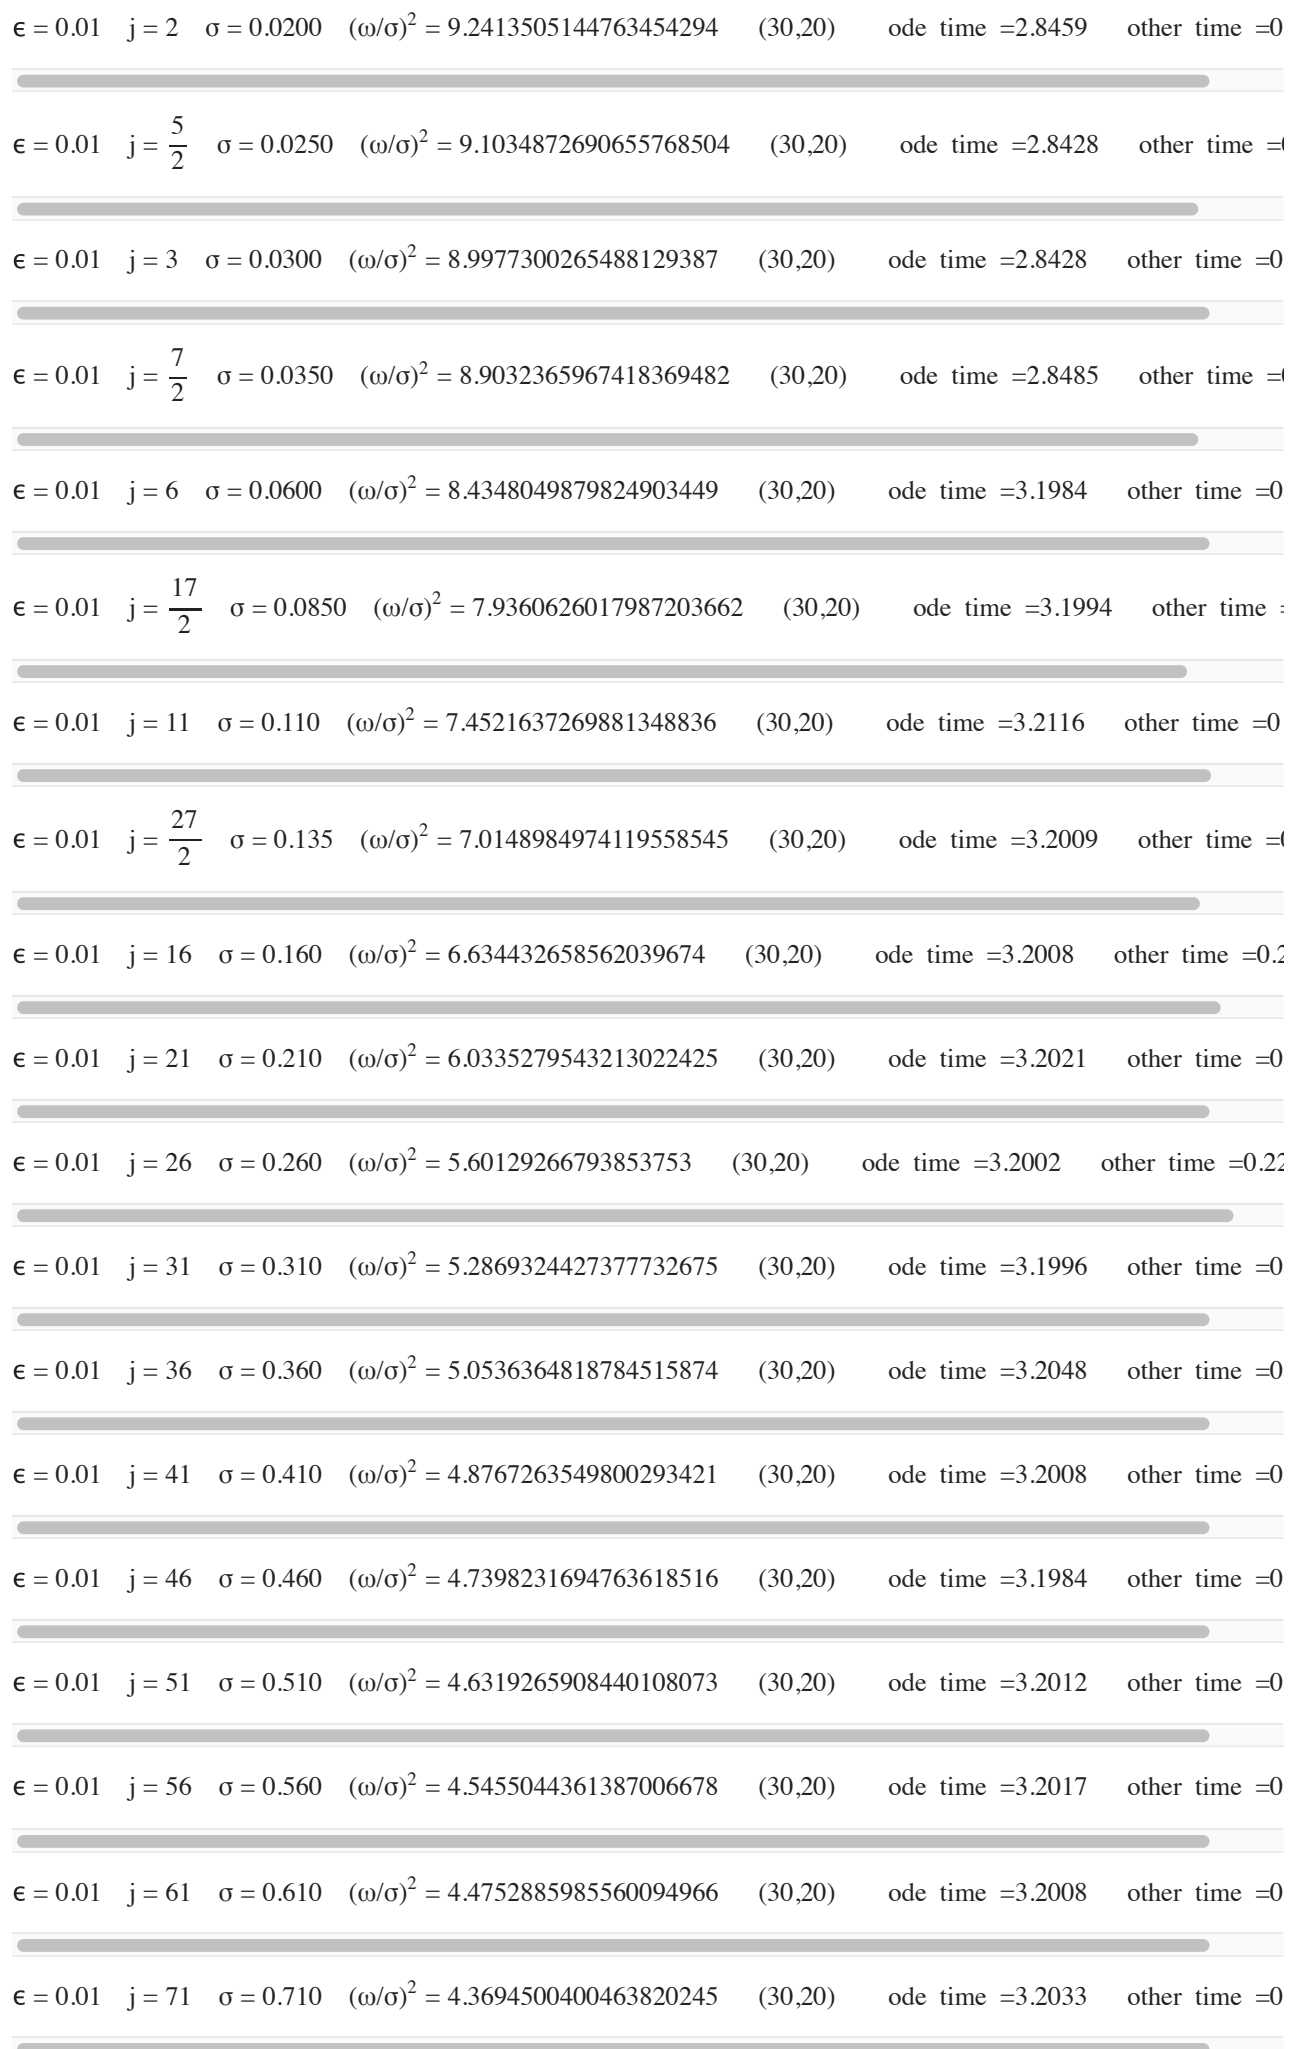 |                    |                   |                                             |         |                  |                  |
| $\epsilon = 0.01$                                                                    | $j = 51$           | $\sigma = 0.510$  | $(\omega/\sigma)^2 = 4.6319265908440108073$ | (30,20) | ode time =3.2012 | other time =0    |
| 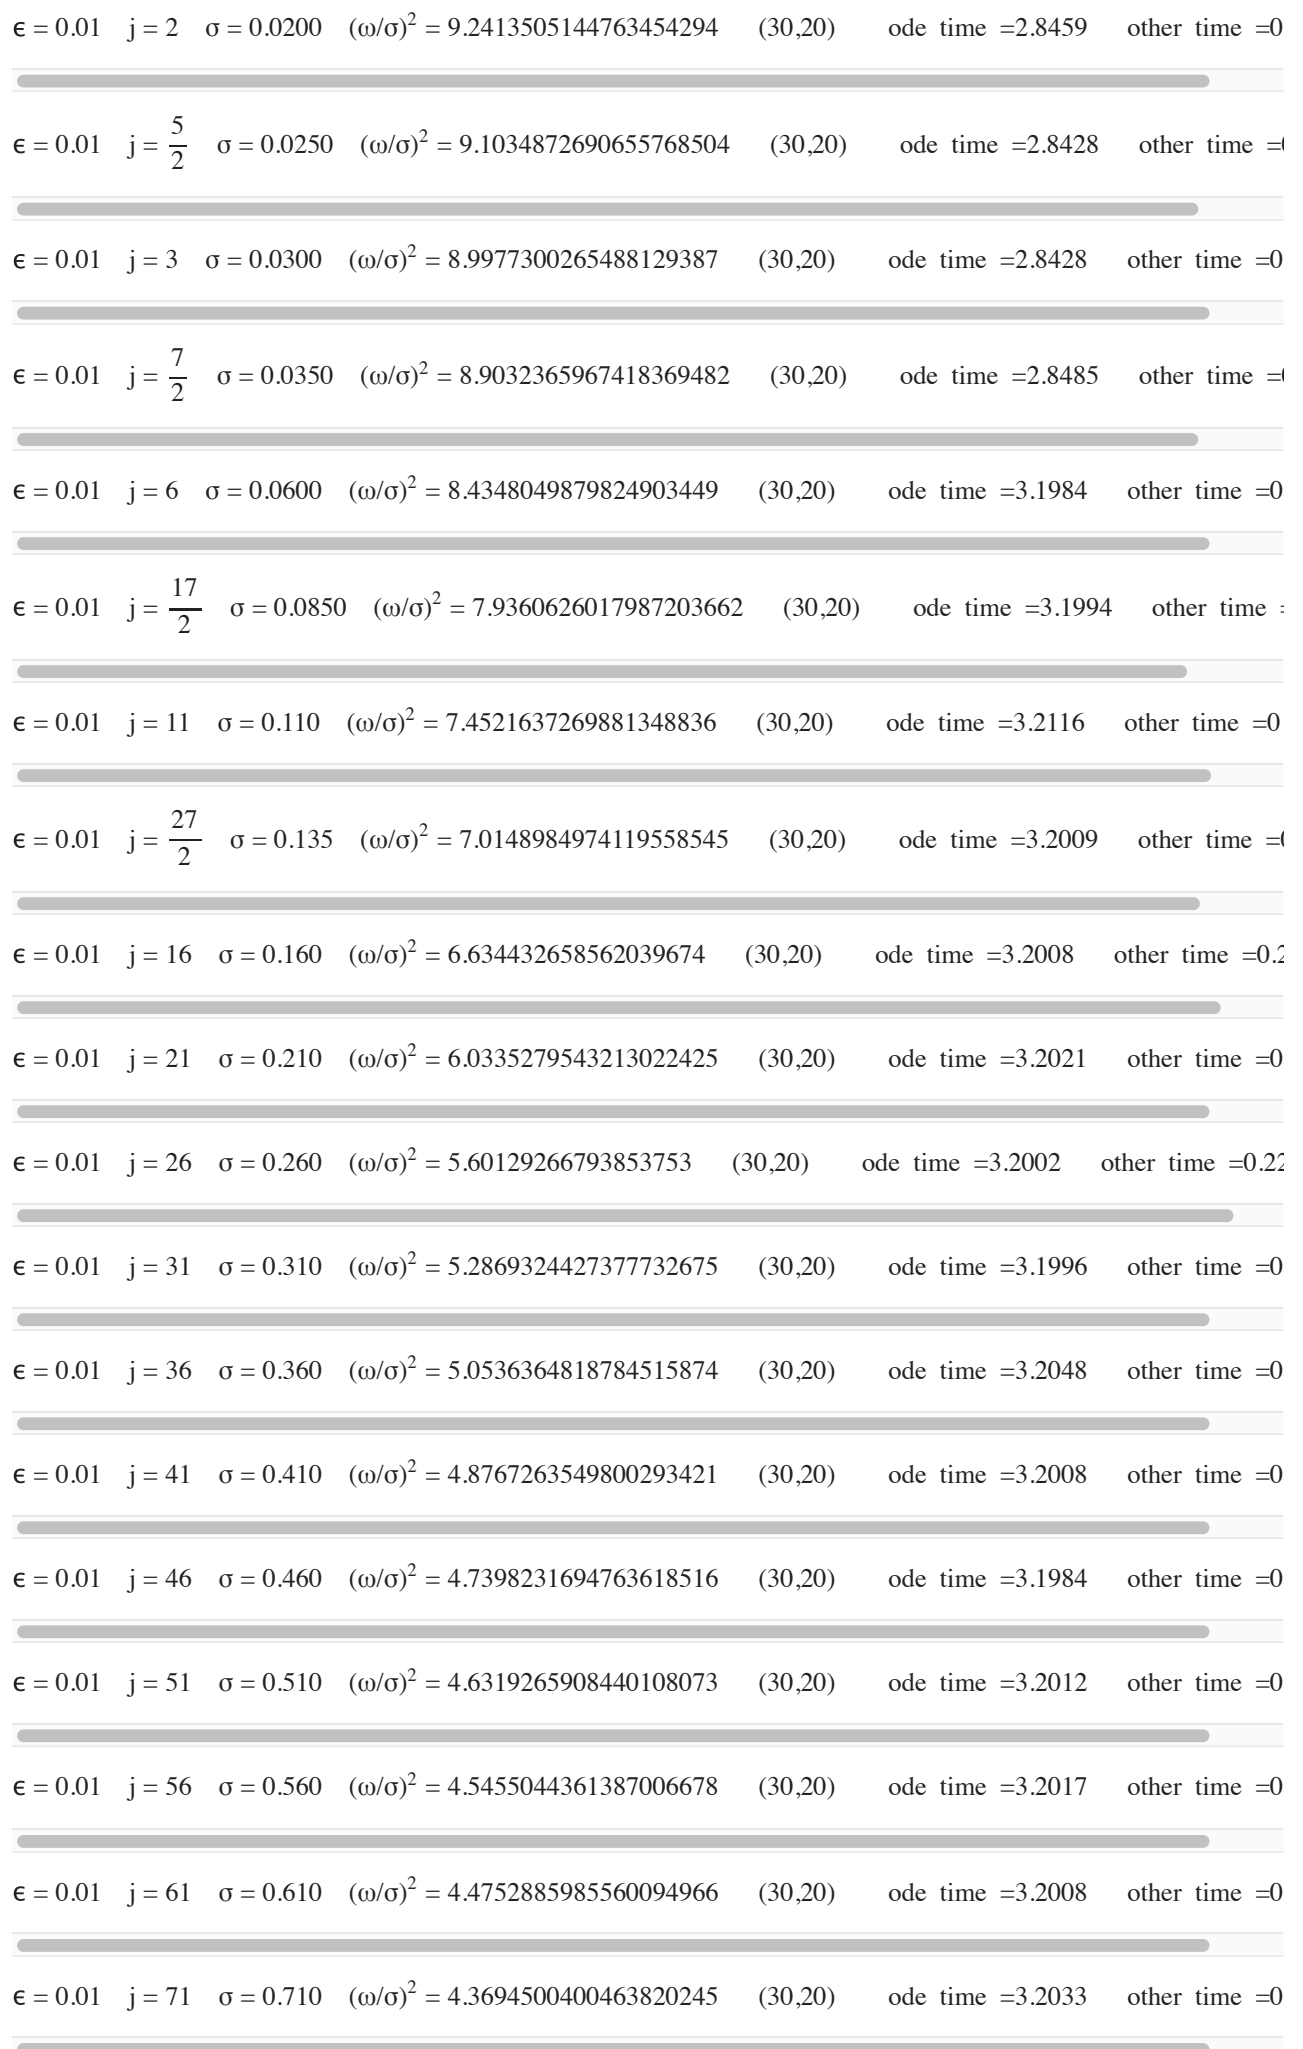 |                    |                   |                                             |         |                  |                  |
| $\epsilon = 0.01$                                                                    | $j = 56$           | $\sigma = 0.560$  | $(\omega/\sigma)^2 = 4.5455044361387006678$ | (30,20) | ode time =3.2017 | other time =0    |
| 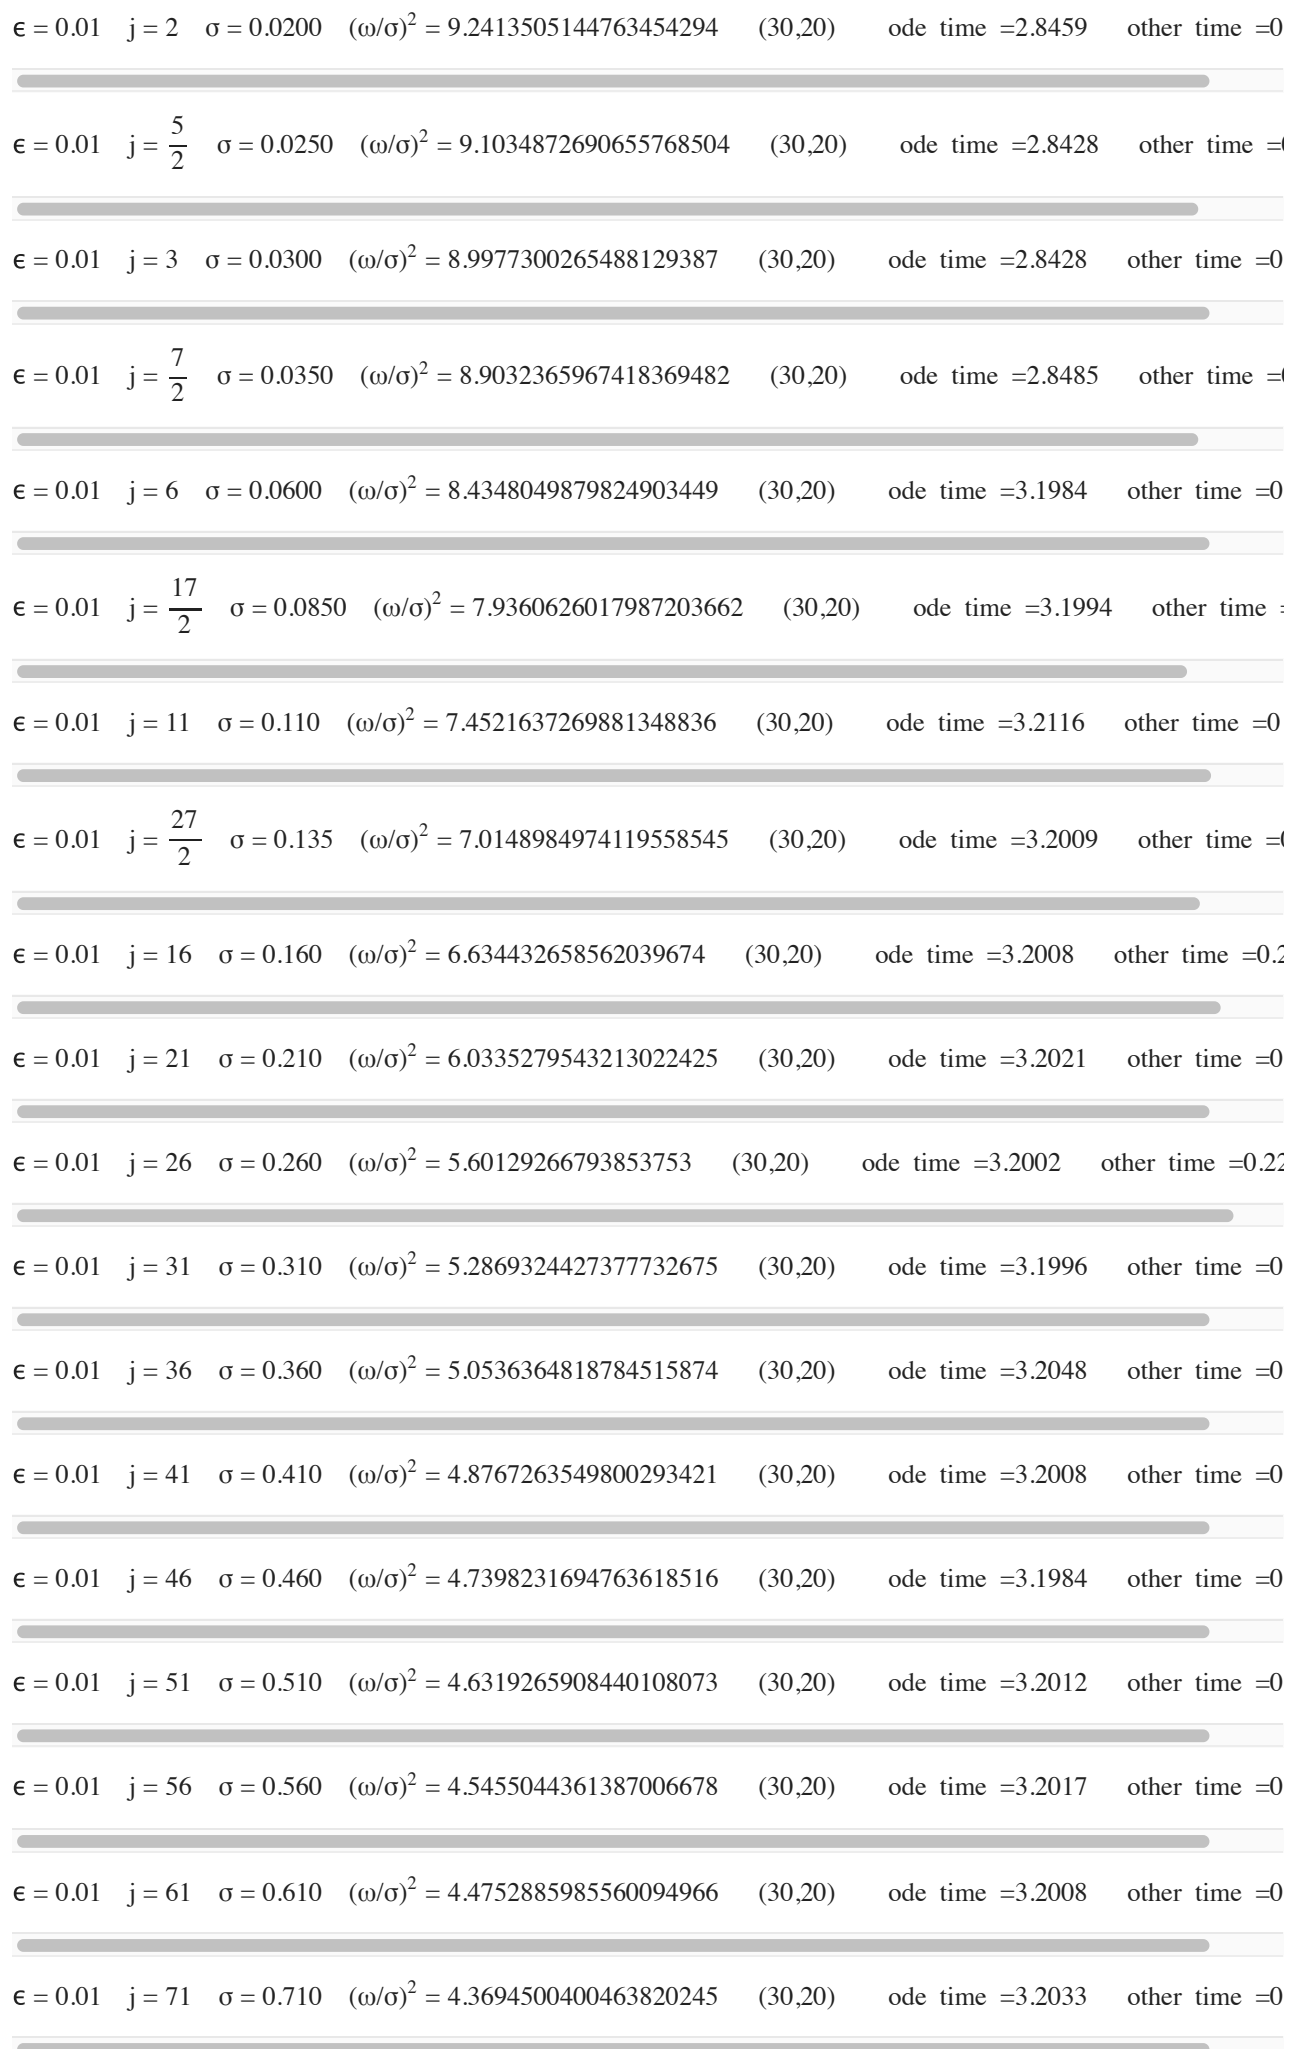 |                    |                   |                                             |         |                  |                  |
| $\epsilon = 0.01$                                                                    | $j = 61$           | $\sigma = 0.610$  | $(\omega/\sigma)^2 = 4.4752885985560094966$ | (30,20) | ode time =3.2008 | other time =0    |
| 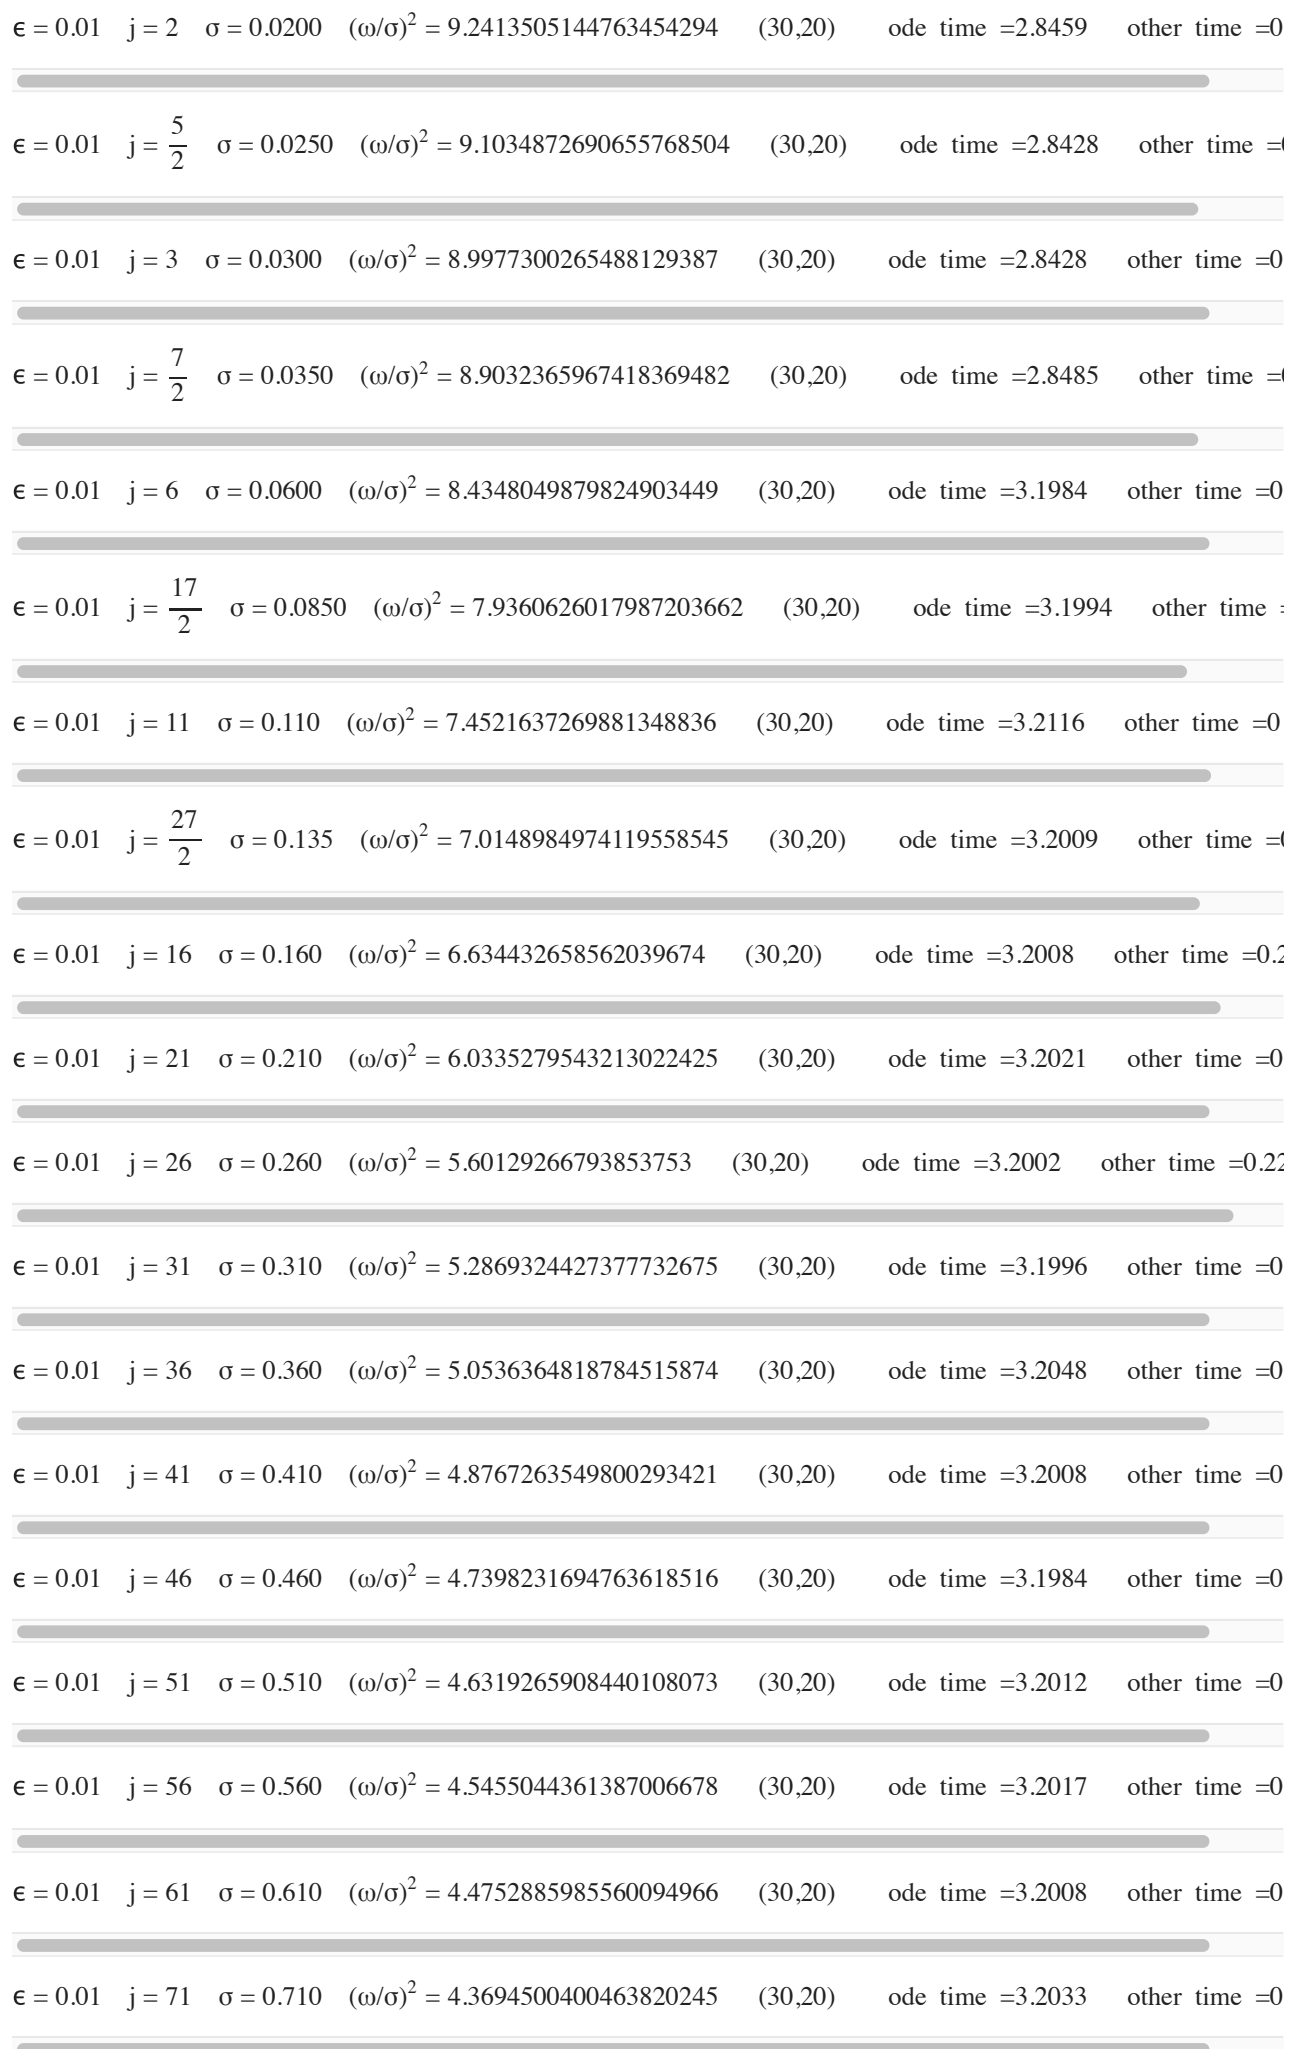 |                    |                   |                                             |         |                  |                  |
| $\epsilon = 0.01$                                                                    | $j = 71$           | $\sigma = 0.710$  | $(\omega/\sigma)^2 = 4.3694500400463820245$ | (30,20) | ode time =3.2033 | other time =0    |
| 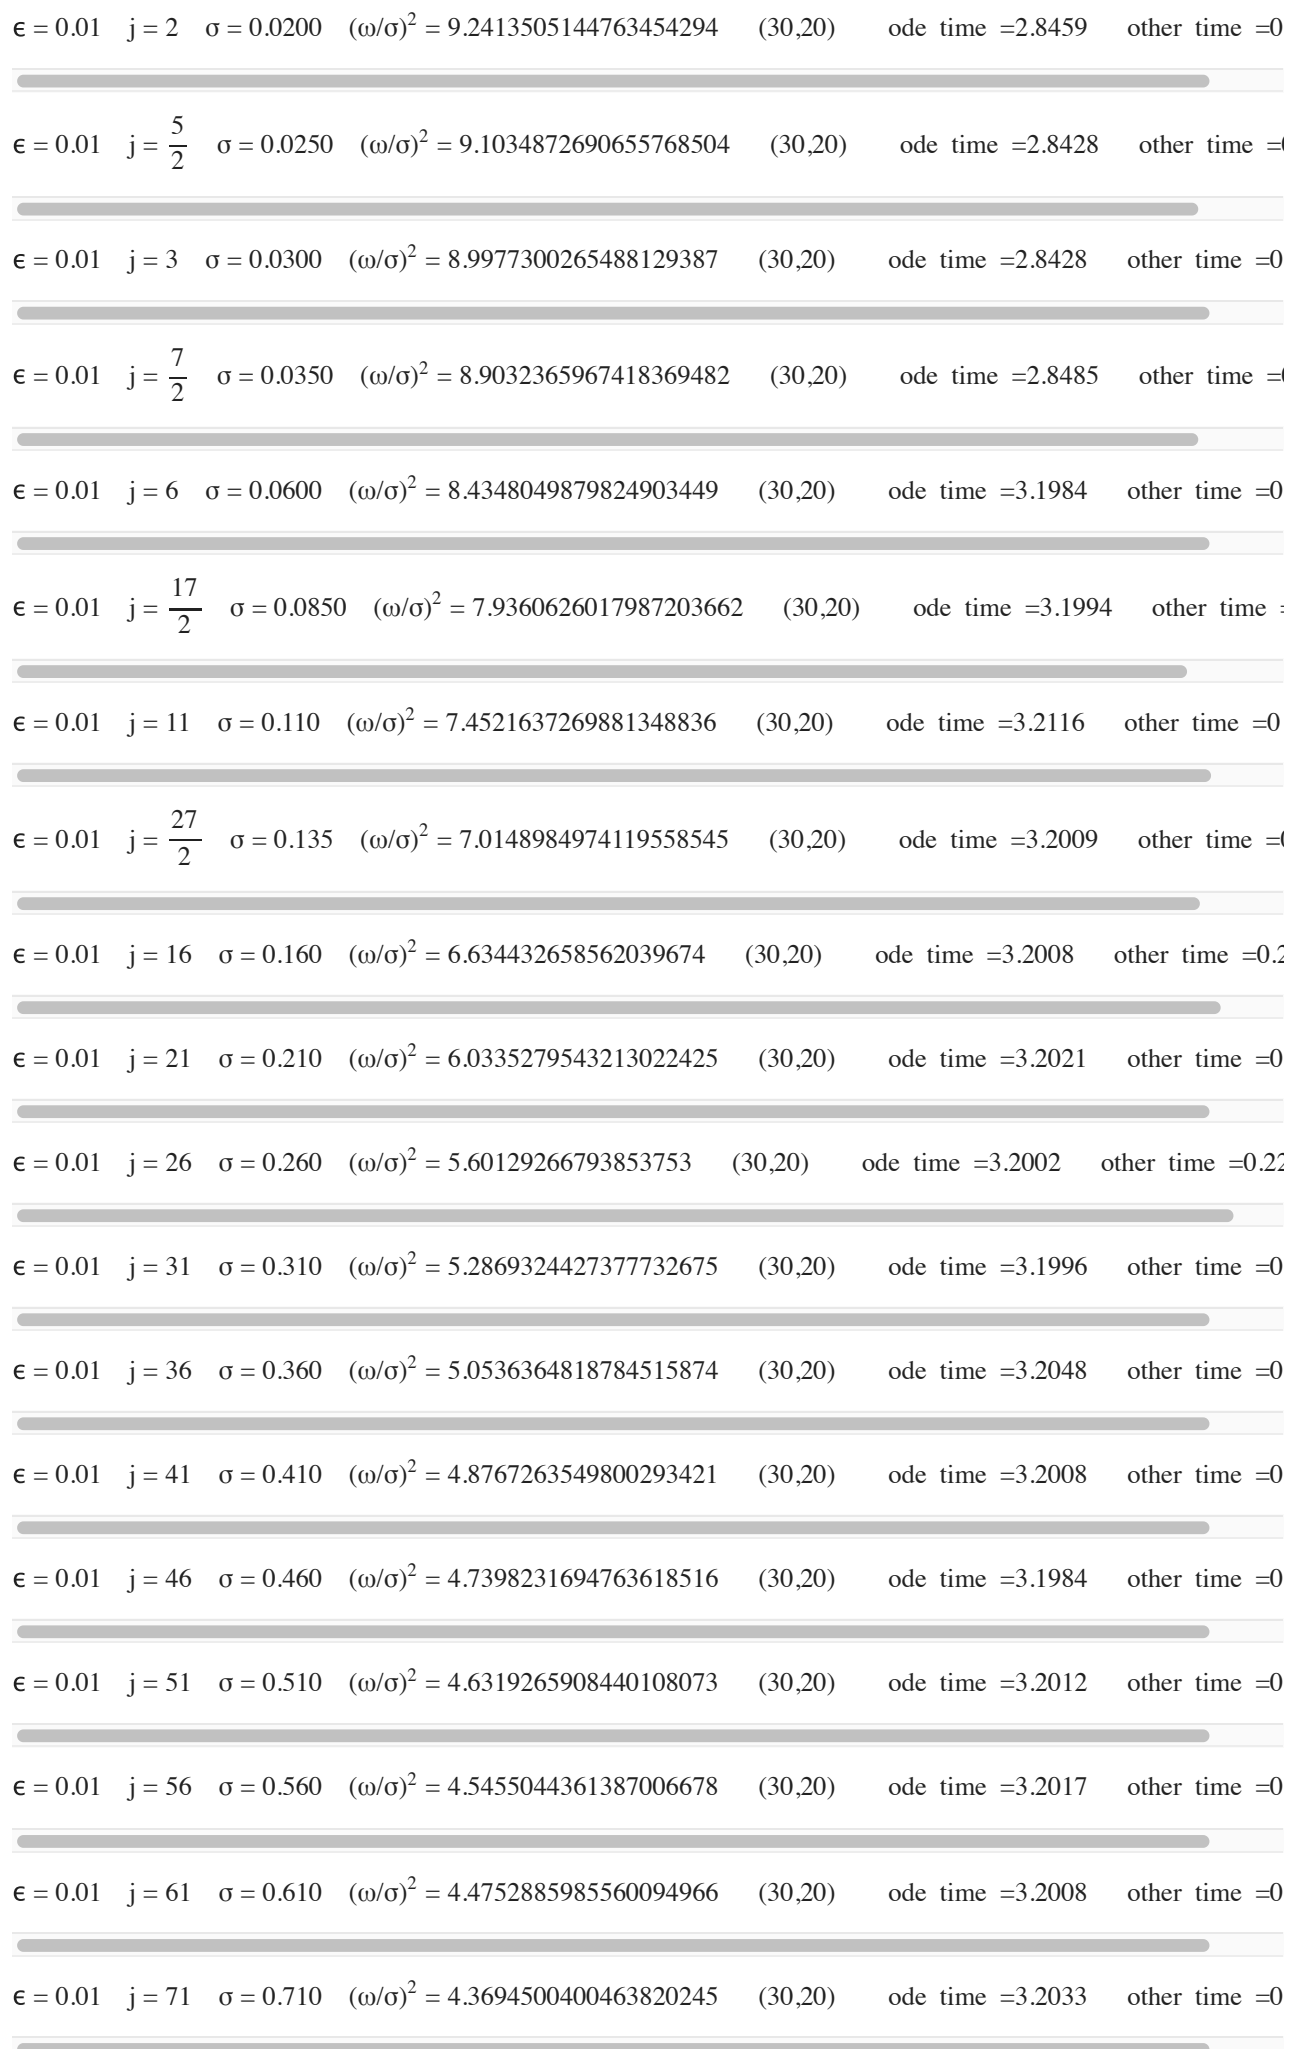 |                    |                   |                                             |         |                  |                  |

|                   |           |                  |                                             |         |                  |                 |
|-------------------|-----------|------------------|---------------------------------------------|---------|------------------|-----------------|
| $\epsilon = 0.01$ | $j = 81$  | $\sigma = 0.810$ | $(\omega/\sigma)^2 = 4.2948079405334089646$ | (30,20) | ode time =3.5615 | other time =0   |
|                   |           |                  |                                             |         |                  |                 |
| $\epsilon = 0.01$ | $j = 91$  | $\sigma = 0.910$ | $(\omega/\sigma)^2 = 4.2403263394586815659$ | (40,20) | ode time =9.3336 | other time =0   |
|                   |           |                  |                                             |         |                  |                 |
| $\epsilon = 0.01$ | $j = 101$ | $\sigma = 1.01$  | $(\omega/\sigma)^2 = 4.1994225594625710714$ | (40,20) | ode time =9.3294 | other time =0   |
|                   |           |                  |                                             |         |                  |                 |
| $\epsilon = 0.01$ | $j = 111$ | $\sigma = 1.11$  | $(\omega/\sigma)^2 = 4.167979915550613492$  | (40,20) | ode time =9.3277 | other time =0.6 |
|                   |           |                  |                                             |         |                  |                 |
| $\epsilon = 0.01$ | $j = 121$ | $\sigma = 1.21$  | $(\omega/\sigma)^2 = 4.143320917670859077$  | (40,20) | ode time =10.360 | other time =0.6 |
|                   |           |                  |                                             |         |                  |                 |
| $\epsilon = 0.01$ | $j = 131$ | $\sigma = 1.31$  | $(\omega/\sigma)^2 = 4.1236456759962382082$ | (40,20) | ode time =10.353 | other time =0   |
|                   |           |                  |                                             |         |                  |                 |
| $\epsilon = 0.01$ | $j = 141$ | $\sigma = 1.41$  | $(\omega/\sigma)^2 = 4.1077096497099901994$ | (40,20) | ode time =10.365 | other time =0   |
|                   |           |                  |                                             |         |                  |                 |
| $\epsilon = 0.01$ | $j = 151$ | $\sigma = 1.51$  | $(\omega/\sigma)^2 = 4.0946310478733501747$ | (40,20) | ode time =10.357 | other time =0   |
|                   |           |                  |                                             |         |                  |                 |
| $\epsilon = 0.01$ | $j = 161$ | $\sigma = 1.61$  | $(\omega/\sigma)^2 = 4.0837716248010645245$ | (40,20) | ode time =10.359 | other time =0   |
|                   |           |                  |                                             |         |                  |                 |
| $\epsilon = 0.01$ | $j = 171$ | $\sigma = 1.71$  | $(\omega/\sigma)^2 = 4.0746606294551170864$ | (50,20) | ode time =25.544 | other time =1   |
|                   |           |                  |                                             |         |                  |                 |
| $\epsilon = 0.01$ | $j = 191$ | $\sigma = 1.91$  | $(\omega/\sigma)^2 = 4.0603558372035246335$ | (50,20) | ode time =25.599 | other time =1   |
|                   |           |                  |                                             |         |                  |                 |
| $\epsilon = 0.01$ | $j = 211$ | $\sigma = 2.11$  | $(\omega/\sigma)^2 = 4.0497725139562661289$ | (50,20) | ode time =25.563 | other time =1   |
|                   |           |                  |                                             |         |                  |                 |
| $\epsilon = 0.01$ | $j = 231$ | $\sigma = 2.31$  | $(\omega/\sigma)^2 = 4.0417303300317987103$ | (50,20) | ode time =25.579 | other time =1   |
|                   |           |                  |                                             |         |                  |                 |
| $\epsilon = 0.01$ | $j = 250$ | $\sigma = 2.50$  | $(\omega/\sigma)^2 = 4.0357586472445873108$ | (60,20) | ode time =54.514 | other time =3   |
|                   |           |                  |                                             |         |                  |                 |
| $\epsilon = 0.01$ | $j = 290$ | $\sigma = 2.90$  | $(\omega/\sigma)^2 = 4.026722737877334427$  | (60,20) | ode time =54.536 | other time =3.5 |

In [57]:

```
ode_name='1j'
epsilon = 0.001

ode_decimal_precision = 30
j_list = [3/2, 2, 5/2, 3, 7/2] + [m/2 for m in range(12, 32, 5)] + [m/2 for m in range(32, 122, 10)]
process_j_list()
```

|                    |                   |                    |                                             |         |                  |              |
|--------------------|-------------------|--------------------|---------------------------------------------|---------|------------------|--------------|
| $\epsilon = 0.001$ | $j = \frac{3}{2}$ | $\sigma = 0.00150$ | $(\omega/\sigma)^2 = 9.5276530065894383767$ | (30,20) | ode time =2.8454 | other time   |
|                    |                   |                    |                                             |         |                  |              |
| $\epsilon = 0.001$ | $j = 2$           | $\sigma = 0.00200$ | $(\omega/\sigma)^2 = 9.3328127565368508927$ | (30,20) | ode time =2.8473 | other time : |
|                    |                   |                    |                                             |         |                  |              |
| $\epsilon = 0.001$ | $j = \frac{5}{2}$ | $\sigma = 0.00250$ | $(\omega/\sigma)^2 = 9.2423039854204874794$ | (30,20) | ode time =2.8417 | other time   |

|                    |                    |                    |                                             |         |                  |              |
|--------------------|--------------------|--------------------|---------------------------------------------|---------|------------------|--------------|
| $\epsilon = 0.001$ | $j = 3$            | $\sigma = 0.00300$ | $(\omega/\sigma)^2 = 9.1927934511757878821$ | (30,20) | ode time =2.8401 | other time : |
| $\epsilon = 0.001$ | $j = \frac{7}{2}$  | $\sigma = 0.00350$ | $(\omega/\sigma)^2 = 9.1625805849842362445$ | (30,20) | ode time =2.8437 | other time : |
| $\epsilon = 0.001$ | $j = 6$            | $\sigma = 0.00600$ | $(\omega/\sigma)^2 = 9.1033675328226328681$ | (30,20) | ode time =2.8393 | other time : |
| $\epsilon = 0.001$ | $j = \frac{17}{2}$ | $\sigma = 0.00850$ | $(\omega/\sigma)^2 = 9.0812815323141515761$ | (30,20) | ode time =2.8400 | other time : |
| $\epsilon = 0.001$ | $j = 11$           | $\sigma = 0.0110$  | $(\omega/\sigma)^2 = 9.0648013382893590722$ | (30,20) | ode time =2.8414 | other time : |
| $\epsilon = 0.001$ | $j = \frac{27}{2}$ | $\sigma = 0.0135$  | $(\omega/\sigma)^2 = 9.0484130879589703181$ | (30,20) | ode time =2.8438 | other time : |
| $\epsilon = 0.001$ | $j = 16$           | $\sigma = 0.0160$  | $(\omega/\sigma)^2 = 9.0305736661629697545$ | (30,20) | ode time =2.8391 | other time : |
| $\epsilon = 0.001$ | $j = 21$           | $\sigma = 0.0210$  | $(\omega/\sigma)^2 = 8.9887608911766755323$ | (30,20) | ode time =2.8449 | other time : |
| $\epsilon = 0.001$ | $j = 26$           | $\sigma = 0.0260$  | $(\omega/\sigma)^2 = 8.9381583304940496491$ | (30,20) | ode time =2.8475 | other time : |
| $\epsilon = 0.001$ | $j = 31$           | $\sigma = 0.0310$  | $(\omega/\sigma)^2 = 8.8790518944857559469$ | (30,20) | ode time =2.8438 | other time : |
| $\epsilon = 0.001$ | $j = 36$           | $\sigma = 0.0360$  | $(\omega/\sigma)^2 = 8.8121375510479175313$ | (30,20) | ode time =2.8420 | other time : |
| $\epsilon = 0.001$ | $j = 41$           | $\sigma = 0.0410$  | $(\omega/\sigma)^2 = 8.7382692060644393831$ | (30,20) | ode time =2.8434 | other time : |
| $\epsilon = 0.001$ | $j = 46$           | $\sigma = 0.0460$  | $(\omega/\sigma)^2 = 8.6583643093475697946$ | (30,20) | ode time =2.8423 | other time : |
| $\epsilon = 0.001$ | $j = 51$           | $\sigma = 0.0510$  | $(\omega/\sigma)^2 = 8.5733536534673498756$ | (30,20) | ode time =2.8476 | other time : |
| $\epsilon = 0.001$ | $j = 56$           | $\sigma = 0.0560$  | $(\omega/\sigma)^2 = 8.4841488567930561233$ | (30,20) | ode time =3.1985 | other time : |

$j \rightarrow \infty$

In [58]:

```
ode_decimal_precision = 30
sigma_list = [0.001,0.01,0.02,0.04,.06,.08,.10,0.15,0.2,0.25,0.3,0.35,0.4,0.45,0.5,.6,0.7,0.8]
process_sigma_list()

ode_decimal_precision = 40
sigma_list = [0.9,1.00,1.15,1.30,1.45,1.6]
process_sigma_list()

ode_decimal_precision = 50
sigma_list = [1.85,2.10,2.35]
process_sigma_list()
```

```
ode_decimal_precision = 60
sigma_list = [2.65, 3.0]
process_sigma_list()
```

|                 |               |                    |                                             |         |                  |                 |
|-----------------|---------------|--------------------|---------------------------------------------|---------|------------------|-----------------|
| $\epsilon = 0.$ | $j = +\infty$ | $\sigma = 0.00100$ | $(\omega/\sigma)^2 = 9.0835330455416439274$ | (30,20) | ode time =2.8446 | other time =0.  |
| $\epsilon = 0.$ | $j = +\infty$ | $\sigma = 0.0100$  | $(\omega/\sigma)^2 = 9.0612674877696019662$ | (30,20) | ode time =2.8430 | other time =0.  |
| $\epsilon = 0.$ | $j = +\infty$ | $\sigma = 0.0200$  | $(\omega/\sigma)^2 = 8.9953627256328547181$ | (30,20) | ode time =2.8435 | other time =0.  |
| $\epsilon = 0.$ | $j = +\infty$ | $\sigma = 0.0400$  | $(\omega/\sigma)^2 = 8.7529666561250607944$ | (30,20) | ode time =2.8420 | other time =0.  |
| $\epsilon = 0.$ | $j = +\infty$ | $\sigma = 0.0600$  | $(\omega/\sigma)^2 = 8.4101046362495019905$ | (30,20) | ode time =3.1951 | other time =0.  |
| $\epsilon = 0.$ | $j = +\infty$ | $\sigma = 0.0800$  | $(\omega/\sigma)^2 = 8.023039607122564902$  | (30,20) | ode time =3.1970 | other time =0.2 |
| $\epsilon = 0.$ | $j = +\infty$ | $\sigma = 0.100$   | $(\omega/\sigma)^2 = 7.6333997588370682807$ | (30,20) | ode time =3.1977 | other time =0.2 |
| $\epsilon = 0.$ | $j = +\infty$ | $\sigma = 0.150$   | $(\omega/\sigma)^2 = 6.7765482096795657426$ | (30,20) | ode time =3.1939 | other time =0.2 |
| $\epsilon = 0.$ | $j = +\infty$ | $\sigma = 0.200$   | $(\omega/\sigma)^2 = 6.1366900976602906555$ | (30,20) | ode time =3.1971 | other time =0.2 |
| $\epsilon = 0.$ | $j = +\infty$ | $\sigma = 0.250$   | $(\omega/\sigma)^2 = 5.6758107936233344452$ | (30,20) | ode time =3.1979 | other time =0.2 |
| $\epsilon = 0.$ | $j = +\infty$ | $\sigma = 0.300$   | $(\omega/\sigma)^2 = 5.3416107840948261744$ | (30,20) | ode time =3.2002 | other time =0.2 |
| $\epsilon = 0.$ | $j = +\infty$ | $\sigma = 0.350$   | $(\omega/\sigma)^2 = 5.0946036902475815238$ | (30,20) | ode time =3.2015 | other time =0.2 |
| $\epsilon = 0.$ | $j = +\infty$ | $\sigma = 0.400$   | $(\omega/\sigma)^2 = 4.9080698932375542945$ | (30,20) | ode time =3.1974 | other time =0.2 |
| $\epsilon = 0.$ | $j = +\infty$ | $\sigma = 0.450$   | $(\omega/\sigma)^2 = 4.7642709897178321575$ | (30,20) | ode time =3.1954 | other time =0.2 |
| $\epsilon = 0.$ | $j = +\infty$ | $\sigma = 0.500$   | $(\omega/\sigma)^2 = 4.6513274620791411213$ | (30,20) | ode time =3.1941 | other time =0.2 |
| $\epsilon = 0.$ | $j = +\infty$ | $\sigma = 0.600$   | $(\omega/\sigma)^2 = 4.4880550633673341101$ | (30,20) | ode time =3.1988 | other time =0.2 |
| $\epsilon = 0.$ | $j = +\infty$ | $\sigma = 0.700$   | $(\omega/\sigma)^2 = 4.3782629343472021188$ | (30,20) | ode time =3.3357 | other time =0.3 |
| $\epsilon = 0.$ | $j = +\infty$ | $\sigma = 0.800$   | $(\omega/\sigma)^2 = 4.3011278478124393871$ | (30,20) | ode time =3.7687 | other time =0.2 |
| $\epsilon = 0.$ | $j = +\infty$ | $\sigma = 0.900$   | $(\omega/\sigma)^2 = 4.2450010384491445038$ | (40,20) | ode time =9.3235 | other time =0.6 |

|                 |               |                 |                                             |         |                  |                    |
|-----------------|---------------|-----------------|---------------------------------------------|---------|------------------|--------------------|
| $\epsilon = 0.$ | $j = +\infty$ | $\sigma = 1.00$ | $(\omega/\sigma)^2 = 4.2029703221284508332$ | (40,20) | ode time =9.3210 | other time =0.67   |
| $\epsilon = 0.$ | $j = +\infty$ | $\sigma = 1.15$ | $(\omega/\sigma)^2 = 4.1573713863219759644$ | (40,20) | ode time =10.358 | other time =0.67   |
| $\epsilon = 0.$ | $j = +\infty$ | $\sigma = 1.30$ | $(\omega/\sigma)^2 = 4.12539105593133652$   | (40,20) | ode time =10.365 | other time =0.6724 |
| $\epsilon = 0.$ | $j = +\infty$ | $\sigma = 1.45$ | $(\omega/\sigma)^2 = 4.1021461737375348904$ | (40,20) | ode time =10.355 | other time =0.67   |
| $\epsilon = 0.$ | $j = +\infty$ | $\sigma = 1.60$ | $(\omega/\sigma)^2 = 4.0847481269085376936$ | (40,20) | ode time =10.358 | other time =0.67   |
| $\epsilon = 0.$ | $j = +\infty$ | $\sigma = 1.85$ | $(\omega/\sigma)^2 = 4.0641690184776466222$ | (50,20) | ode time =25.565 | other time =1.74   |
| $\epsilon = 0.$ | $j = +\infty$ | $\sigma = 2.10$ | $(\omega/\sigma)^2 = 4.0502197825876173506$ | (50,20) | ode time =25.575 | other time =1.74   |
| $\epsilon = 0.$ | $j = +\infty$ | $\sigma = 2.35$ | $(\omega/\sigma)^2 = 4.0403445880660037356$ | (50,20) | ode time =25.599 | other time =1.73   |
| $\epsilon = 0.$ | $j = +\infty$ | $\sigma = 2.65$ | $(\omega/\sigma)^2 = 4.0318918859941641937$ | (60,20) | ode time =54.594 | other time =3.93   |
| $\epsilon = 0.$ | $j = +\infty$ | $\sigma = 3.00$ | $(\omega/\sigma)^2 = 4.0249908291237605178$ | (60,20) | ode time =54.584 | other time =3.94   |

## Graphics

In [59]:

```
ode_name='3j'
plot_data_j = {}
for eps_string, eps_data in data[ode_name]['finite'].items():
    if eps_string not in plot_data_j:
        plot_data_j[eps_string] = []
    for jval, item in eps_data.items():
        sigmaval = item['sigmaval']
        pval = sqrt(6)*sigmaval
        p = RDF(pval)
        fs_ratio = RDF(item['fs_ratio']*sigmaval^2/pval^2)
        plot_data_j[eps_string].append((p, fs_ratio))
epsvals = list(plot_data_j.keys())
epsvals.sort()
print(epsvals)
```

```
['0.01', '0.3', '0.4', '0.55', '0.7071']
```

In [60]:

```
p=\
list_plot(plot_data_j['0.01'], legend_label=r'\epsilon=.01$', marker='.', markersize=2, plotjoined=True,
+list_plot(plot_data_j['0.3'], legend_label=r'\epsilon=.3$', marker='.', markersize=2, plotjoined=True,
+list_plot(plot_data_j['0.4'], legend_label=r'\epsilon=.4$', marker='.', markersize=2, plotjoined=True,
+list_plot(plot_data_j['0.55'], legend_label=r'\epsilon=.55$', marker='.', markersize=2, plotjoined=True,
+list_plot(plot_data_j['0.7071'], legend_label=r'\epsilon=.7071$', marker='.', markersize=2, plotjoined=True)
+text(r"\bf ode-3_j", (3,.6), fontsize=18, color='black')\
+line([(0,1), (7.2,1)], linestyle=":")
p.set_legend_options(loc='center right', markerscale=1, numpoints=1, shadow=False)
p.axes_labels(['$p$', '$\omega_{\min}^2/p^2$'])
p.axes_labels_size(1.5)
p.show(ticks_integer=True, ymin=0.3)
p.save('3j_finite.pdf', dpi=600, ticks_integer=True, ymin=0.3)
```



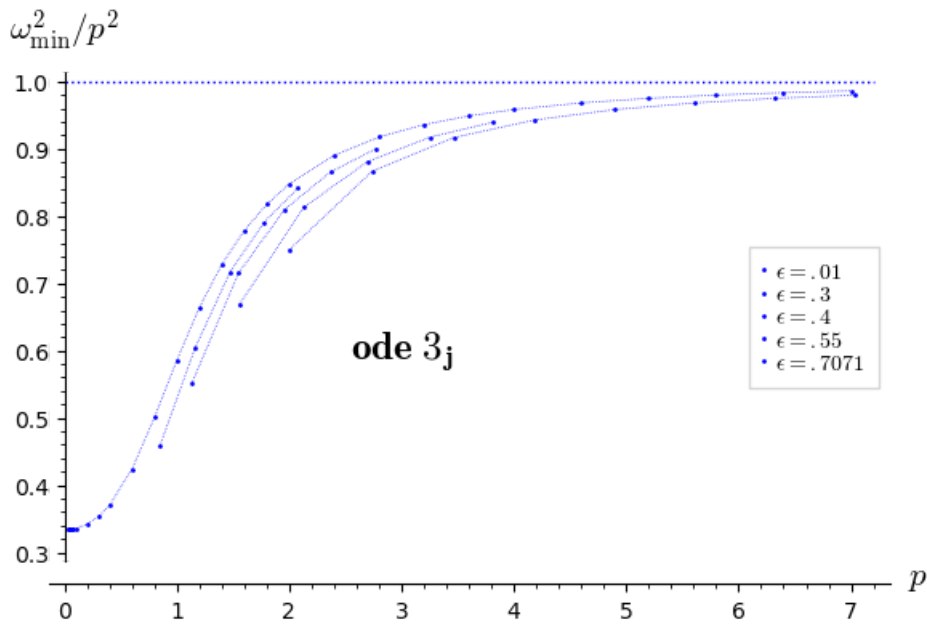

```
In [61]:
ode_name='3j'
plot_data_asyp = []
for key,item in data[ode_name]['asyp'].items():
    sigmaval = item['sigmaval']
    pval = sqrt(6)*sigmaval
    p = RDF(pval)
    fs_ratio = RDF(item['fs_ratio']*sigmaval^2/pval^2)
    plot_data_asyp.append((p,fs_ratio))
```

```
In [62]:
p=\
list_plot(plot_data_asyp,legend_label=r'$\epsilon=0$',marker=r'$\circ$',size=10)\
+list_plot(plot_data_j['0.01'],legend_label=r'$\epsilon=.01$',marker='.',size=8)\
+text(r"${\bf ode-3-j}$",(3,.6),fontsize=18,color='black')\
+line([(0,1),(7.5,1)],linestyle=":")
p.set_legend_options(loc='center right',markerscale=1,numpoints=1,shadow=False)
p.axes_labels(['$p$', '$\omega_{\min}^2/p^2$'])
p.axes_labels_size(1.5)
p.show(ticks_integer=True,ymin=0.3)
p.save('3j_asyp.pdf',dpi=600,ticks_integer=True,ymin=0.3)
```

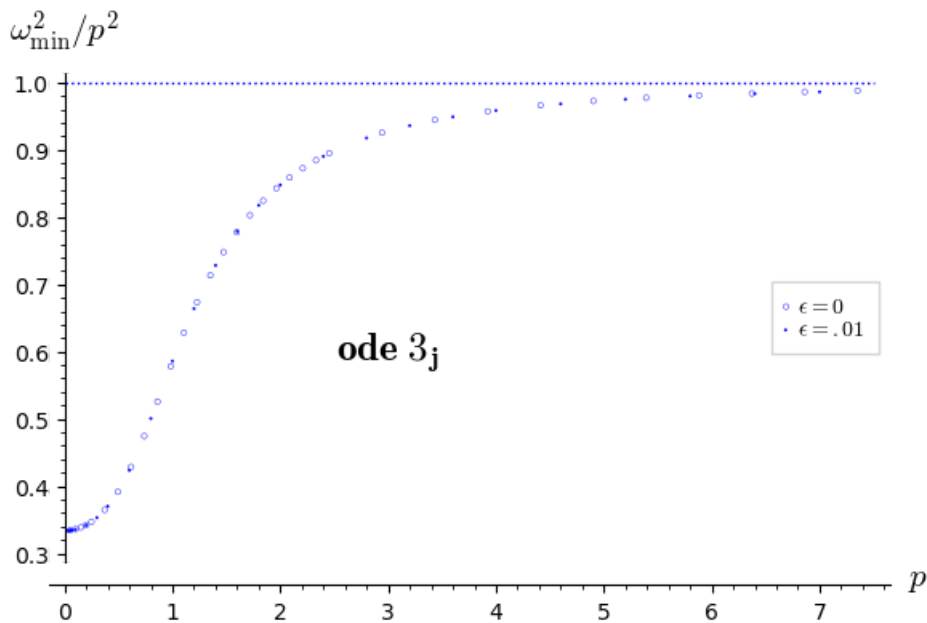

```
In [63]:
ode_name='2j'
plot_data_j = {}
for eps_string,eps_data in data[ode_name]['finite'].items():
    if eps_string not in plot_data_j:
        plot_data_j[eps_string]=[]
    for jval,item in eps_data.items():
```

```

    sigmaval = item['sigmaval']
    pval = 2*sigmaval
    p = RDF(pval)
    fs_ratio = RDF(item['fs_ratio']*sigmaval^2/pval^2)
    plot_data_j[eps_string].append((p,fs_ratio))
epsvals= list(plot_data_j.keys())
epsvals.sort()
print(epsvals)

```

```
['0.01', '0.08', '0.1', '0.125', '0.15', '0.2', '0.25', '0.325', '0.4', '0.5', '0.6', '0.7071']
```

In [64]:

```

p=\
list_plot(plot_data_j['0.01'],legend_label=r'\epsilon=.01$',marker='.',markersize=2,plotjoined=True)
+list_plot(plot_data_j['0.08'],legend_label=r'\epsilon=.08$',marker='.',markersize=2,plotjoined=True)
+list_plot(plot_data_j['0.1'],legend_label=r'\epsilon=.1$',marker='.',markersize=2,plotjoined=True)
+list_plot(plot_data_j['0.125'],legend_label=r'\epsilon=.125$',marker='.',markersize=2,plotjoined=True)
+list_plot(plot_data_j['0.15'],legend_label=r'\epsilon=.15$',marker='.',markersize=2,plotjoined=True)
+list_plot(plot_data_j['0.2'],legend_label=r'\epsilon=.2$',marker='.',markersize=2,plotjoined=True)
+list_plot(plot_data_j['0.25'],legend_label=r'\epsilon=.25$',marker='.',markersize=2,plotjoined=True)
+list_plot(plot_data_j['0.325'],legend_label=r'\epsilon=.325$',marker='.',markersize=2,plotjoined=True)
+list_plot(plot_data_j['0.4'],legend_label=r'\epsilon=.4$',marker='.',markersize=2,plotjoined=True)
+list_plot(plot_data_j['0.5'],legend_label=r'\epsilon=.5$',marker='.',markersize=2,plotjoined=True)
+list_plot(plot_data_j['0.6'],legend_label=r'\epsilon=.6$',marker='.',markersize=2,plotjoined=True)
+list_plot(plot_data_j['0.7071'],legend_label=r'\epsilon=.7071$',marker='.',markersize=2,plotjoined=True)
+text(r"\bf ode-2_j", (4.5, .85), fontsize=18, color='black')\
+line([(0,1),(8,1)],linestyle=":")
p.set_legend_options(loc='center right',markerscale=1,numpoints=1,shadow=False)
p.axes_labels(['$p$', '$\omega_{\min}^2/p^2$'])
p.axes_labels_size(1.5)
p.show(ticks_integer=True,xmin=0)
p.save('2j_finite.pdf',dpi=600,ticks_integer=True,xmin=0)

```

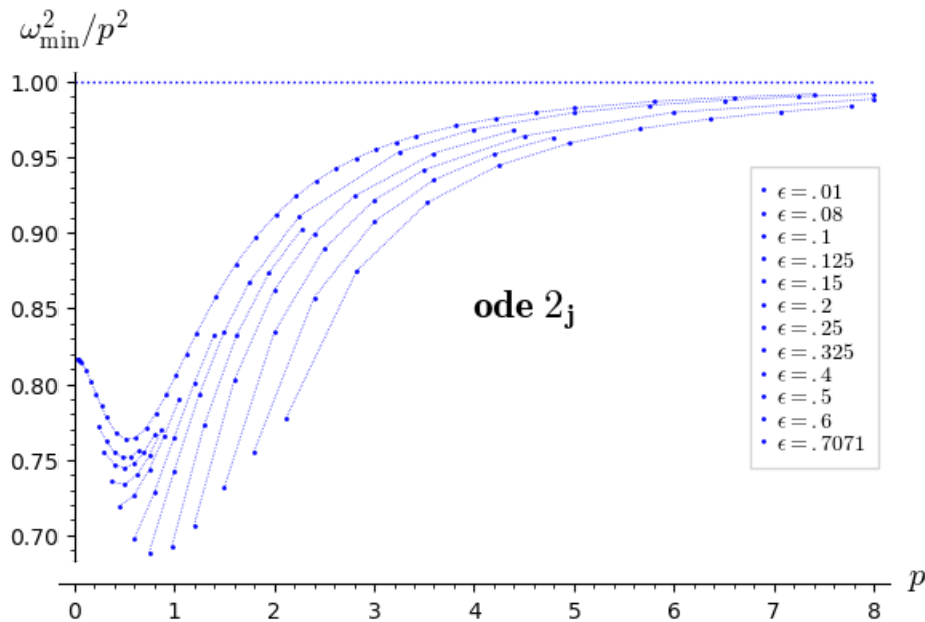

In [65]:

```

ode_name='2j'
plot_data_asymp=[]
for key,item in data[ode_name]['asymp'].items():
    sigmaval = item['sigmaval']
    pval = 2*sigmaval
    p = RDF(pval)
    fs_ratio = RDF(item['fs_ratio']*sigmaval^2/pval^2)
    plot_data_asymp.append((p,fs_ratio))

```

In [66]:

```

p=list_plot(plot_data_asymp,legend_label=r'\epsilon=0$',marker=r'\circ$',size=10)\
+list_plot(plot_data_j['0.01'],legend_label=r'\epsilon=.01$',marker='.',size=8)\
+text(r"\bf ode-2_j", (4.5, .85), fontsize=18, color='black')\
+line([(0,1),(8,1)],linestyle=":")
p.set_legend_options(loc='center right',markerscale=1,numpoints=1,shadow=False)
p.axes_labels(['$p$', '$\omega_{\min}^2/p^2$'])
p.axes_labels_size(1.5)
p.show(ticks_integer=True)
p.save('2j_asymp.pdf',dpi=600,ticks_integer=True)

```

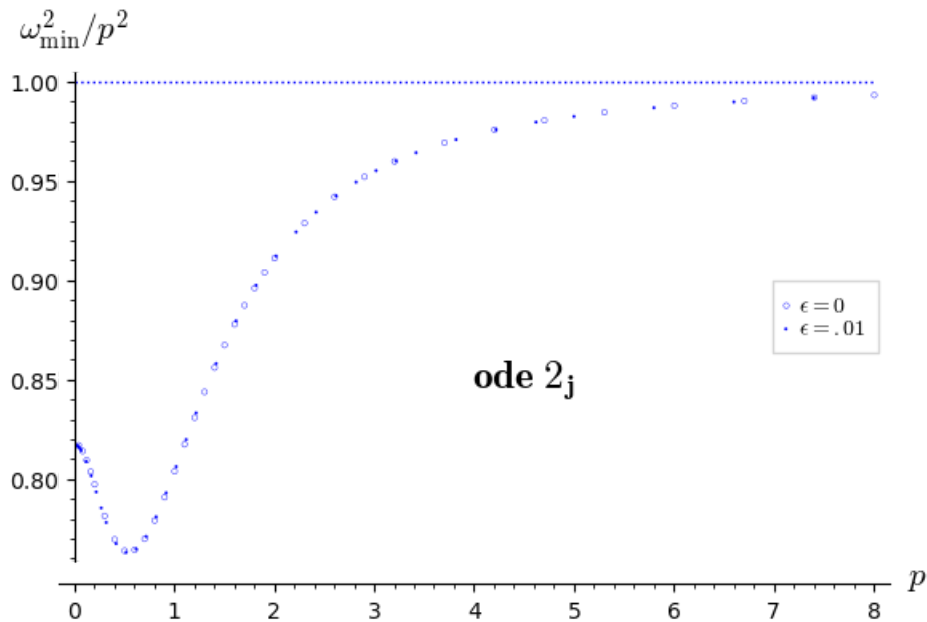

In [67]:

```
ode_name='1j'
plot_data_j = {}
for eps_string, eps_data in data[ode_name]['finite'].items():
    if eps_string not in plot_data_j:
        plot_data_j[eps_string] = []
    for jval, item in eps_data.items():
        sigmaval = item['sigmaval']
        epsval = item['epsilonb']
        pval = sqrt(4*sigmaval^2+3*epsval^2)
        p = RDF(pval)
        fs_ratio = RDF(item['fs_ratio']*sigmaval^2/pval^2)
        plot_data_j[eps_string].append((p, fs_ratio))
epsvals = list(plot_data_j.keys())
epsvals.sort()
print(epsvals)
```

```
['0.001', '0.01', '0.15', '0.25', '0.35', '0.5', '0.7071']
```

In [68]:

```
p = \
list_plot(plot_data_j['0.01'], legend_label=r'$\epsilon=.01$', marker='.', markersize=2, plotjoined=True)
+list_plot(plot_data_j['0.15'], legend_label=r'$\epsilon=.15$', marker='.', markersize=2, plotjoined=True)
+list_plot(plot_data_j['0.25'], legend_label=r'$\epsilon=.25$', marker='.', markersize=2, plotjoined=True)
+list_plot(plot_data_j['0.35'], legend_label=r'$\epsilon=.35$', marker='.', markersize=2, plotjoined=True)
+list_plot(plot_data_j['0.5'], legend_label=r'$\epsilon=.5$', marker='.', markersize=2, plotjoined=True)
+list_plot(plot_data_j['0.7071'], legend_label=r'$\epsilon=.7071$', marker='.', markersize=2, plotjoined=True)
+text(r"${\bf ode-1_j}$", (2.5, 1.5), fontsize=18, color='black')
p.set_legend_options(loc='center right', markerscale=1, numpoints=1, shadow=False)
p.axes_labels(['$p$', '$\omega_{\min}^2/p^2$'])
p.axes_labels_size(1.5)
p.show(ticks_integer=True)
p.save('1j_finite.pdf', dpi=600, ticks_integer=True)
```

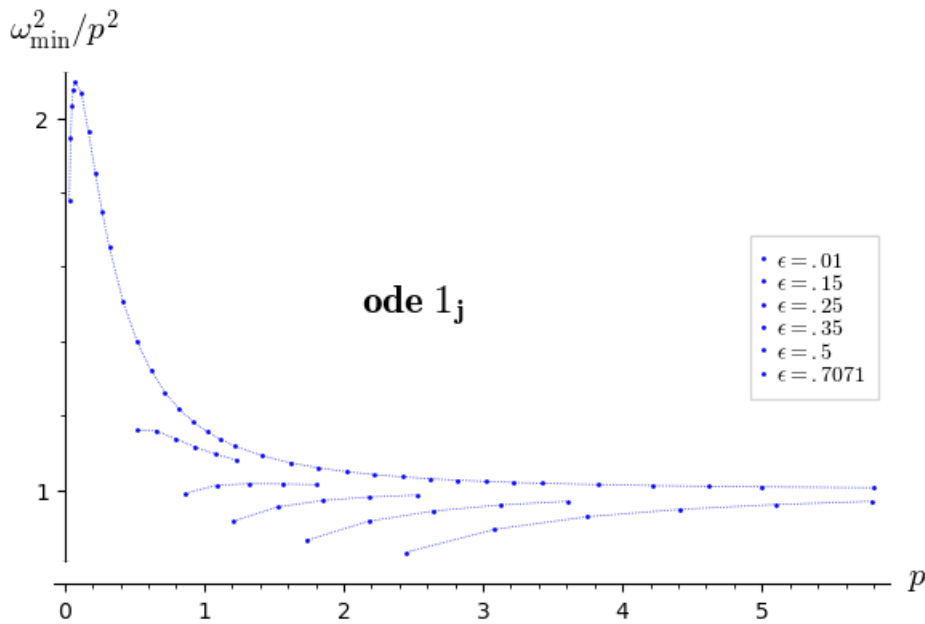

```
In [69]:
ode_name='1j'
plot_data_asympt = []
for key,item in data[ode_name]['asympt'].items():
    sigmaval = item['sigmaval']
    pval = 2*sigmaval
    # pval = sqrt(4*sigmaval^2+3*epsval^2)
    p = RDF(pval)
    fs_ratio = RDF(item['fs_ratio']*sigmaval^2/pval^2)
    plot_data_asympt.append((p,fs_ratio))
```

```
In [70]:
p=list_plot(plot_data_asympt,legend_label=r'$\epsilon=0$',marker=r'$\circ$',size=10)\
+list_plot(plot_data_j['0.01'],legend_label=r'$\epsilon=.01$',marker='.',size=8)\
+text(r"${\bf ode-1_j}$",(2.5,1.5),fontsize=18,color='black')\
+line([(0,1),(6.0,1)],linestyle=":")
#p.set_legend_options(loc='center right',markerscale=1,numpoints=1,shadow=False)
p.axes_labels(['$p$', '$\omega_{\min}^2/p^2$'])
p.set_legend_options(loc='center right',markerscale=1.5,shadow=False)
p.axes_labels_size(1.5)
p.show(ticks_integer=True,ymin=1)
p.save('1j_asympt.pdf',dpi=600,ticks_integer=True,ymin=1)
```

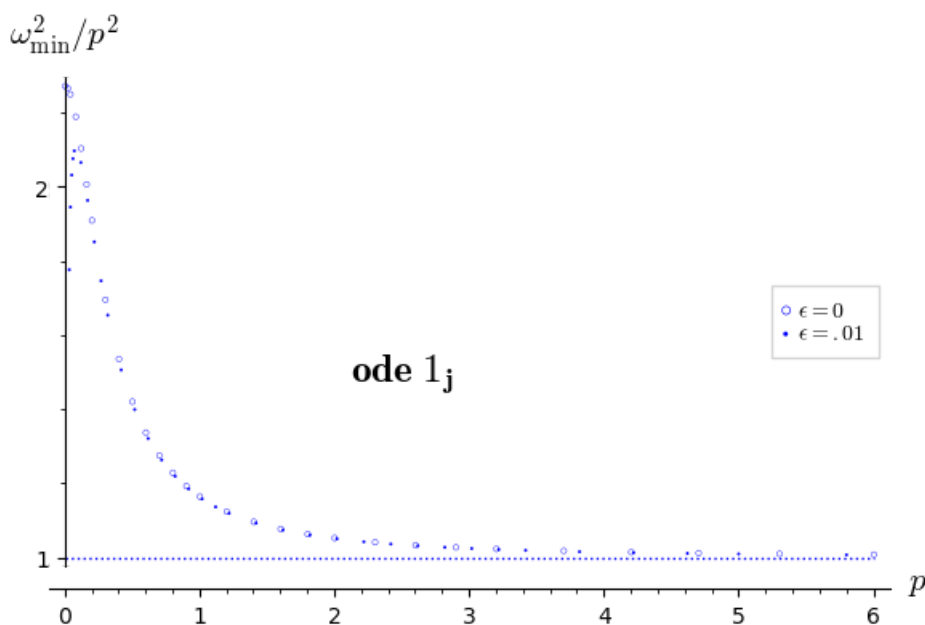

```
In [78]:
p=list_plot(plot_data_asympt,legend_label=r'$\epsilon=0$',marker=r'$\circ$',size=24)\
+list_plot(plot_data_j['0.001'],legend_label=r'$\epsilon=.001$',marker='.',markersize=3,plotjoined=True)\
+text(r"${\bf ode-1_j}$",(0.1,1.8),fontsize=18,color='black')\
+list_plot(plot_data_j['0.01'],legend_label=r'$\epsilon=.01$',marker='x',markersize=3,plotjoined=True)\
p.axes_labels(['$p$', '$\omega_{\min}^2/p^2$'])
```

```

p.set_legend_options(shadow=False)
#p.set_legend_options(loc='center right',markerscale=1.5,shadow=False)
p.axes_labels_size(1.5)
p.show(xmax=.2,ymin=1.7)
p.save('1j_smallp.pdf',dpi=600,xmax=.2,ymin=1.7)

```

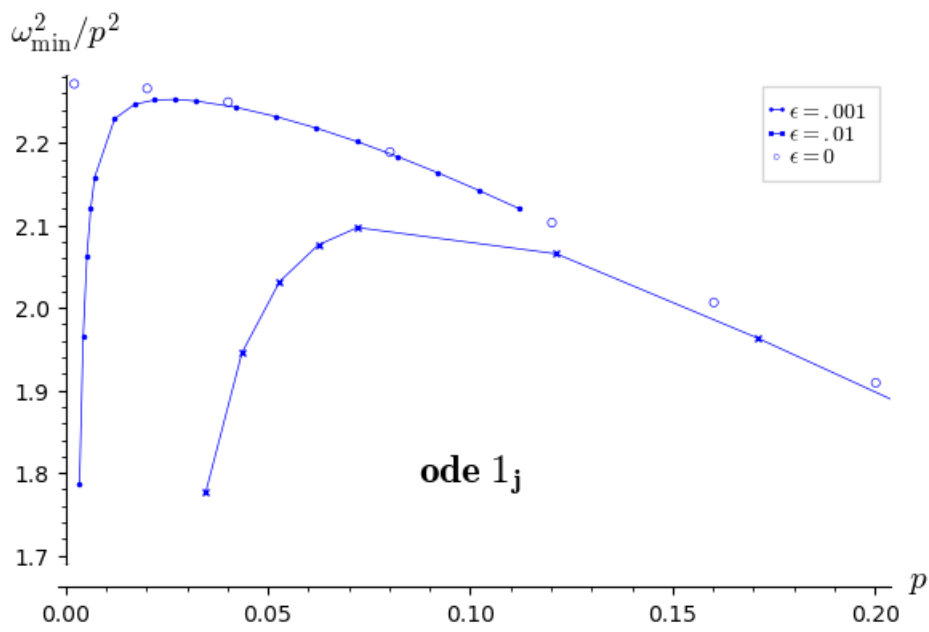

Supplement: Supplementary file 3 [file property_P.pdf]
